# Supplementary material for: PECAN: A Product-Quantized Content Addressable Memory Network
Source: arXiv:2208.13571 source file (2022-08-13)
Supplement: Supplementary file 1 [file Exp_Jie.tex]

\documentclass[10pt,twocolumn,letterpaper]{article}
\usepackage[rebuttal]{cvpr}

% Include other packages here, before hyperref.
\usepackage{graphicx}
\usepackage{amsmath}
\usepackage{amssymb}
\usepackage{booktabs}
\usepackage{multirow}

% If you comment hyperref and then uncomment it, you should delete
% egpaper.aux before re-running latex.  (Or just hit 'q' on the first latex
% run, let it finish, and you should be clear).
\usepackage[pagebackref=blue,breaklinks,colorlinks=true,allcolors=blue,bookmarks=false]{hyperref}

% Support for easy cross-referencing
\usepackage[capitalize]{cleveref}
\crefname{section}{Sec.}{Secs.}
\Crefname{section}{Section}{Sections}
\Crefname{table}{Table}{Tables}
\crefname{table}{Tab.}{Tabs.}
\usepackage{xcolor}

% If you wish to avoid re-using figure, table, and equation numbers from
% the main paper, please uncomment the following and change the numbers
% appropriately.
%\setcounter{figure}{2}
%\setcounter{table}{1}
%\setcounter{equation}{2}

% If you wish to avoid re-using reference numbers from the main paper,
% please uncomment the following and change the counter for `enumiv' to
% the number of references you have in the main paper (here, 6).
%\let\oldthebibliography=\thebibliography
%\let\oldendthebibliography=\endthebibliography
%\renewenvironment{thebibliography}[1]{%
%     \oldthebibliography{#1}%
%     \setcounter{enumiv}{6}%
%}{\oldendthebibliography}

%%%%%%%%% PAPER ID  - PLEASE UPDATE
 % *** Enter the CVPR Paper ID here

\begin{document}

%%%%%%%%% TITLE - PLEASE UPDATE
\title{Experiments}  % **** Enter the paper title here

\maketitle
\thispagestyle{empty}
\appendix

%%%%%%%%% BODY TEXT - ENTER YOUR RESPONSE BELOW
%%%% Check im2col in PyTorch %%%%
\section{Different template matching schemes}
{\color{red}{\textbf{Date: 2021.10.22 Friday}}} \\

1) We use dot product to match the template between subvectors in Feature matrix and prototypes.

2) We use L1-norm to match the template and L2-norm for BP to update prototypes.

3) We use L1-norm to match the template and epoch-aware scheme for BP to update prototypes.

Since $|x| = sign(x) \times x$, we use an approximation function for $sign(x)$.

\begin{equation}
    F(x) = \begin{cases}
    k (-sign (x) \frac{t^2 x^3}{2} + \sqrt{2}tx^2), & |x| < \frac{4\sqrt{2}}{3t} \\
    sign(x) k x, & else
    \end{cases}
\end{equation}
where $t = 10^{T_{min}+T_{max} \cdot \frac{e}{E}}$, $k = \max(\frac{1}{t}, 1)$, $e$ is the current epoch, $E$ is the total number of epochs. Then 
\begin{equation}
    F'(x) = clip(k(2\sqrt{2}tx - \frac{3}{2}sign(x)t^2 x^2),-k,k)
\end{equation}

Experiment results are shown in Tab~\ref{tab:different_schemes}.

\setlength{\tabcolsep}{5mm}{
\begin{table}[htbp]
\scriptsize
\centering
\begin{tabular}{cc}
\toprule
Model & Accuracy ($\%$) \\
\midrule
Baseline & $99.44$ \\
\midrule
All-CoBoLeNet (Dot Product) & $98.66$ \\
\midrule
All-CoBoLeNet (L2-norm) & $97.36$ \\
\midrule
All-CoBoLeNet (epoch-aware) & $98.39$ \\
\bottomrule
\end{tabular}
\caption{We compare three different template matching schemes above.}
\label{tab:different_schemes}
\end{table}}

\section{L1-Norm on the Latent Vector to shrink prototypes}
{\color{red}{\textbf{Date: 2021.11.05 Friday}}} \\
{\color{red}{One problem:}} Till now only prototypes are updated, that's to say, weights in the CoBo layer are totally adopted from the pretrained network.

%%%%%%%%% REFERENCES
{\small
\bibliographystyle{ieee_fullname}
\bibliography{egbib}
}

\end{document}
