# Supplementary material for: PECAN: A Product-Quantized Content Addressable Memory Network
Source: arXiv:2208.13571 source file (2022-08-13)
Supplement: Supplementary file 2 [file SM.tex]

\documentclass[10pt,twocolumn,letterpaper]{article}
\usepackage[rebuttal]{cvpr}

% Include other packages here, before hyperref.
\usepackage{graphicx}
\usepackage{amsmath}
\usepackage{amssymb}
\usepackage{booktabs}

% If you comment hyperref and then uncomment it, you should delete
% egpaper.aux before re-running latex.  (Or just hit 'q' on the first latex
% run, let it finish, and you should be clear).
\usepackage[pagebackref,breaklinks,colorlinks,bookmarks=false]{hyperref}

% Support for easy cross-referencing
\usepackage[capitalize]{cleveref}
\crefname{section}{Sec.}{Secs.}
\Crefname{section}{Section}{Sections}
\Crefname{table}{Table}{Tables}
\crefname{table}{Tab.}{Tabs.}

% If you wish to avoid re-using figure, table, and equation numbers from
% the main paper, please uncomment the following and change the numbers
% appropriately.
%\setcounter{figure}{2}
%\setcounter{table}{1}
%\setcounter{equation}{2}

% If you wish to avoid re-using reference numbers from the main paper,
% please uncomment the following and change the counter for `enumiv' to
% the number of references you have in the main paper (here, 6).
%\let\oldthebibliography=\thebibliography
%\let\oldendthebibliography=\endthebibliography
%\renewenvironment{thebibliography}[1]{%
%     \oldthebibliography{#1}%
%     \setcounter{enumiv}{6}%
%}{\oldendthebibliography}

%%%%%%%%% PAPER ID  - PLEASE UPDATE
 % *** Enter the CVPR Paper ID here

\begin{document}

%%%%%%%%% TITLE - PLEASE UPDATE
\title{\LaTeX\ Guidelines for Author Response}  % **** Enter the paper title here

\maketitle
\thispagestyle{empty}
\appendix

%%%%%%%%% BODY TEXT - ENTER YOUR RESPONSE BELOW
\section{Introduction}

After receiving paper reviews, authors may optionally submit a rebuttal to address the reviewers' comments, which will be limited to a {\bf one page} PDF file.
Please follow the steps and style guidelines outlined below for submitting your author response.

The author rebuttal is optional and, following similar guidelines to previous CVPR conferences, is meant to provide you with an opportunity to rebut factual errors or to supply additional information requested by the reviewers.
It is NOT intended to add new contributions (theorems, algorithms, experiments) that were absent in the original submission and NOT specifically requested by the reviewers.
You may optionally add a figure, graph, or proof to your rebuttal to better illustrate your answer to the reviewers' comments.

Per a passed 2018 PAMI-TC motion, reviewers should refrain from requesting significant additional experiments for the rebuttal or penalize for lack of additional experiments.
Authors should refrain from including new experimental results in the rebuttal, especially when not specifically requested to do so by the reviewers.
Authors may include figures with illustrations or comparison tables of results reported in the submission/supplemental material or in other papers.

Just like the original submission, the rebuttal must maintain anonymity and cannot include external links that reveal the author identity or circumvent the length restriction.
The rebuttal must comply with this template (the use of sections is not required, though it is recommended to structure the rebuttal for ease of reading).

%-------------------------------------------------------------------------

\subsection{Response length}
Author responses must be no longer than 1 page in length including any references and figures.
Overlength responses will simply not be reviewed.
This includes responses where the margins and formatting are deemed to have been significantly altered from those laid down by this style guide.
Note that this \LaTeX\ guide already sets figure captions and references in a smaller font.

%------------------------------------------------------------------------
\section{Formatting your Response}

{\bf Make sure to update the paper title and paper ID in the appropriate place in the tex file.}

All text must be in a two-column format.
The total allowable size of the text area is $6\frac78$ inches (17.46 cm) wide by $8\frac78$ inches (22.54 cm) high.
Columns are to be $3\frac14$ inches (8.25 cm) wide, with a $\frac{5}{16}$ inch (0.8 cm) space between them.
The top margin should begin 1 inch (2.54 cm) from the top edge of the page.
The bottom margin should be $1\frac{1}{8}$ inches (2.86 cm) from the bottom edge of the page for $8.5 \times 11$-inch paper;
for A4 paper, approximately $1\frac{5}{8}$ inches (4.13 cm) from the bottom edge of the page.

Please number any displayed equations.
It is important for readers to be able to refer to any particular equation.

Wherever Times is specified, Times Roman may also be used.
Main text should be in 10-point Times, single-spaced.
Section headings should be in 10 or 12 point Times.
All paragraphs should be indented 1 pica (approx.~$\frac{1}{6}$ inch or 0.422 cm).
Figure and table captions should be 9-point Roman type as in \cref{fig:onecol}.

List and number all bibliographical references in 9-point Times, single-spaced,
at the end of your response.
When referenced in the text, enclose the citation number in square brackets, for example~\cite{Alpher05}.
Where appropriate, include the name(s) of editors of referenced books.

\begin{figure}[t]
  \centering
  \fbox{\rule{0pt}{0.5in} \rule{0.9\linewidth}{0pt}}
   \caption{Example of caption.  It is set in Roman so that mathematics
   (always set in Roman: $B \sin A = A \sin B$) may be included without an
   ugly clash.}
   \label{fig:onecol}
\end{figure}

To avoid ambiguities, it is best if the numbering for equations, figures, tables, and references in the author response does not overlap with that in the main paper (the reviewer may wonder if you talk about \cref{fig:onecol} in the author response or in the paper).
See \LaTeX\ template for a workaround.

%-------------------------------------------------------------------------
\subsection{Illustrations, graphs, and photographs}

All graphics should be centered.
Please ensure that any point you wish to make is resolvable in a printed copy of the response.
Resize fonts in figures to match the font in the body text, and choose line widths which render effectively in print.
Readers (and reviewers), even of an electronic copy, may choose to print your response in order to read it.
You cannot insist that they do otherwise, and therefore must not assume that they can zoom in to see tiny details on a graphic.

When placing figures in \LaTeX, it is almost always best to use \verb+\includegraphics+, and to specify the  figure width as a multiple of the line width as in the example below
{\small\begin{verbatim}
   \usepackage{graphicx} ...
   \includegraphics[width=0.8\linewidth]
                   {myfile.pdf}
\end{verbatim}
}

%%%%%%%%% REFERENCES
{\small
\bibliographystyle{ieee_fullname}
\bibliography{egbib}
}

\end{document}
