# Supplementary material for: PECAN: A Product-Quantized Content Addressable Memory Network
Source: arXiv:2208.13571 source file (2022-08-13)
Supplement: Supplementary file 3 [file Records.tex]

\documentclass[10pt,twocolumn,letterpaper]{article}
\usepackage[rebuttal]{cvpr}

% Include other packages here, before hyperref.
\usepackage{graphicx}
\usepackage{amsmath}
\usepackage{amssymb}
\usepackage{booktabs}
\usepackage{multirow}

% If you comment hyperref and then uncomment it, you should delete
% egpaper.aux before re-running latex.  (Or just hit 'q' on the first latex
% run, let it finish, and you should be clear).
\usepackage[pagebackref=blue,breaklinks,colorlinks=true,allcolors=blue,bookmarks=false]{hyperref}

% Support for easy cross-referencing
\usepackage[capitalize]{cleveref}
\crefname{section}{Sec.}{Secs.}
\Crefname{section}{Section}{Sections}
\Crefname{table}{Table}{Tables}
\crefname{table}{Tab.}{Tabs.}
\usepackage{xcolor}
\newcommand{\Jie}{\color{orange}{}}
\newcommand{\Rui}{\color{blue}{}}

% If you wish to avoid re-using figure, table, and equation numbers from
% the main paper, please uncomment the following and change the numbers
% appropriately.
%\setcounter{figure}{2}
%\setcounter{table}{1}
%\setcounter{equation}{2}

% If you wish to avoid re-using reference numbers from the main paper,
% please uncomment the following and change the counter for `enumiv' to
% the number of references you have in the main paper (here, 6).
%\let\oldthebibliography=\thebibliography
%\let\oldendthebibliography=\endthebibliography
%\renewenvironment{thebibliography}[1]{%
%     \oldthebibliography{#1}%
%     \setcounter{enumiv}{6}%
%}{\oldendthebibliography}


%%%%%%%%% PAPER ID  - PLEASE UPDATE
\def\cvprPaperID{*****} % *** Enter the CVPR Paper ID here
\def\confName{CVPR}
\def\confYear{2022}

\begin{document}

%%%%%%%%% TITLE - PLEASE UPDATE
\title{\LaTeX\ Guidelines for Author Response}  % **** Enter the paper title here

\maketitle
\thispagestyle{empty}
\appendix

%%%%%%%%% BODY TEXT - ENTER YOUR RESPONSE BELOW
%%%% Check im2col in PyTorch %%%%
\section{Check im2col in PyTorch}
{\color{red}{\textbf{Date: 2021.09.14 Tuesday}}}

% im2col operation
For im2col:

1) 'it should be like that in debut but in row fashion' $\xrightarrow[]{}$ Yes, im2col operation in PyTorch is in row fashion.

2) \href{https://hackmd.io/@bouteille/B1Cmns09I}{https://hackmd.io/@bouteille/B1Cmns09I} $\xrightarrow[]{}$ Yes, this is what python does.

3) A \href{https://github.com/RuiLin0212/demos/blob/main/python_im2col_fold_check.ipynb}{demo} to show the im2col (unfold) operation in PyTorch. I built the input the same as Figure 2 in DeBut, and it is obvious the result got by PyTorch is different from that shown in our paper. PyTorch is in row fashion and DeBut paper is in the column fashion

% folding operation
For folding operation:

Its relationship with im2col (unfold) is input = fold(unfold(input)) / divisor, the divisor is needed since the blocks overlapped. Please check the \href{https://github.com/RuiLin0212/demos/blob/main/python_im2col_fold_check.ipynb}{demo} to see their relationships and how divisor looks like. 


%%%% WHT experiments %%%%
\section{WHT experimental results}
\label{sec:WHT_preliminary}
{\color{red}{\textbf{Date: 2021.09.15 Wednesday}}}

%% case 1
\textbf{Case 1: Delete the Bottom Row to Make the number of dimensions equal to 8.}

Experimental Details:
\begin{enumerate}
\item Select an image from CIFAR-10 dataset, the size of the image is $[1, 3, 32, 32]$.
\item Use $\rm{im2col}$ operation to get the flattened input, which is of size $[1, 27, 900]$.
\item Cut the flattened input into three bands, each of which is of size $[1, 9, 900]$.
\item Delete the bottom row of each band, and each new band is of size $[1, 8, 900]$.
\item Apply 1-D Fast Walsh-Hadamard transform (WHT) on each new band.
\item Visualize the bands before and after WHT to see the clustering results by t-SNE.
\item Compare the prototype assignments in the spatial and frequency domains.
\item Check whether l1-norm can work along with the WHT operation to assign the proper prototype to each sample in the frequency domain.
\end{enumerate}

Figure~\ref{fig:tsne} is the t-SNE visualization results of step 6.
\begin{figure*}
\centering
\includegraphics[scale=0.45]{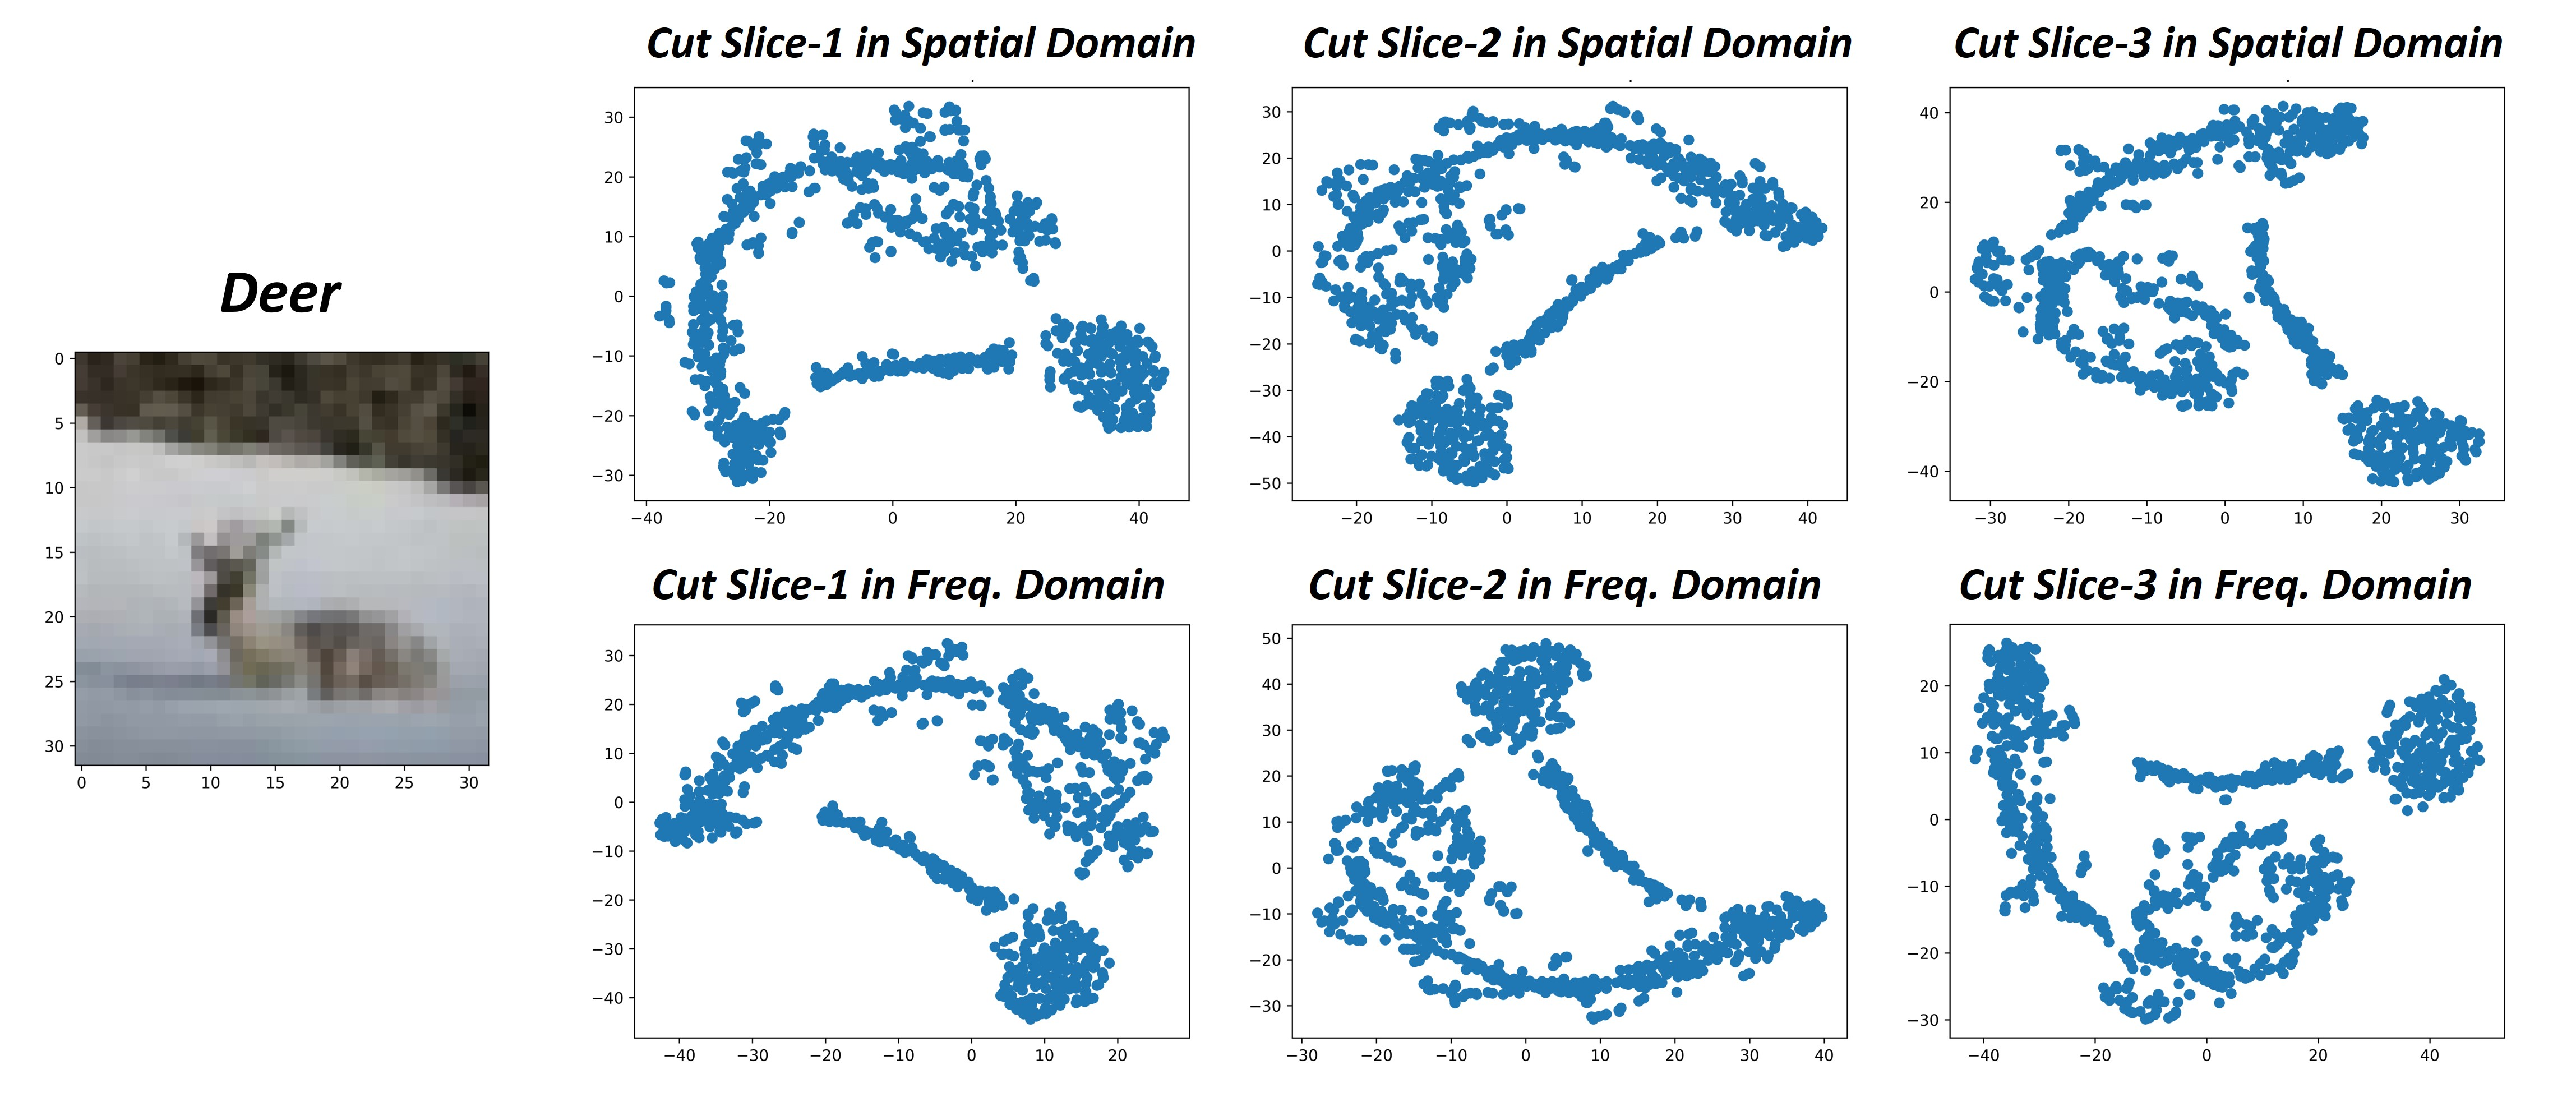}

\centering
\includegraphics[scale=0.45]{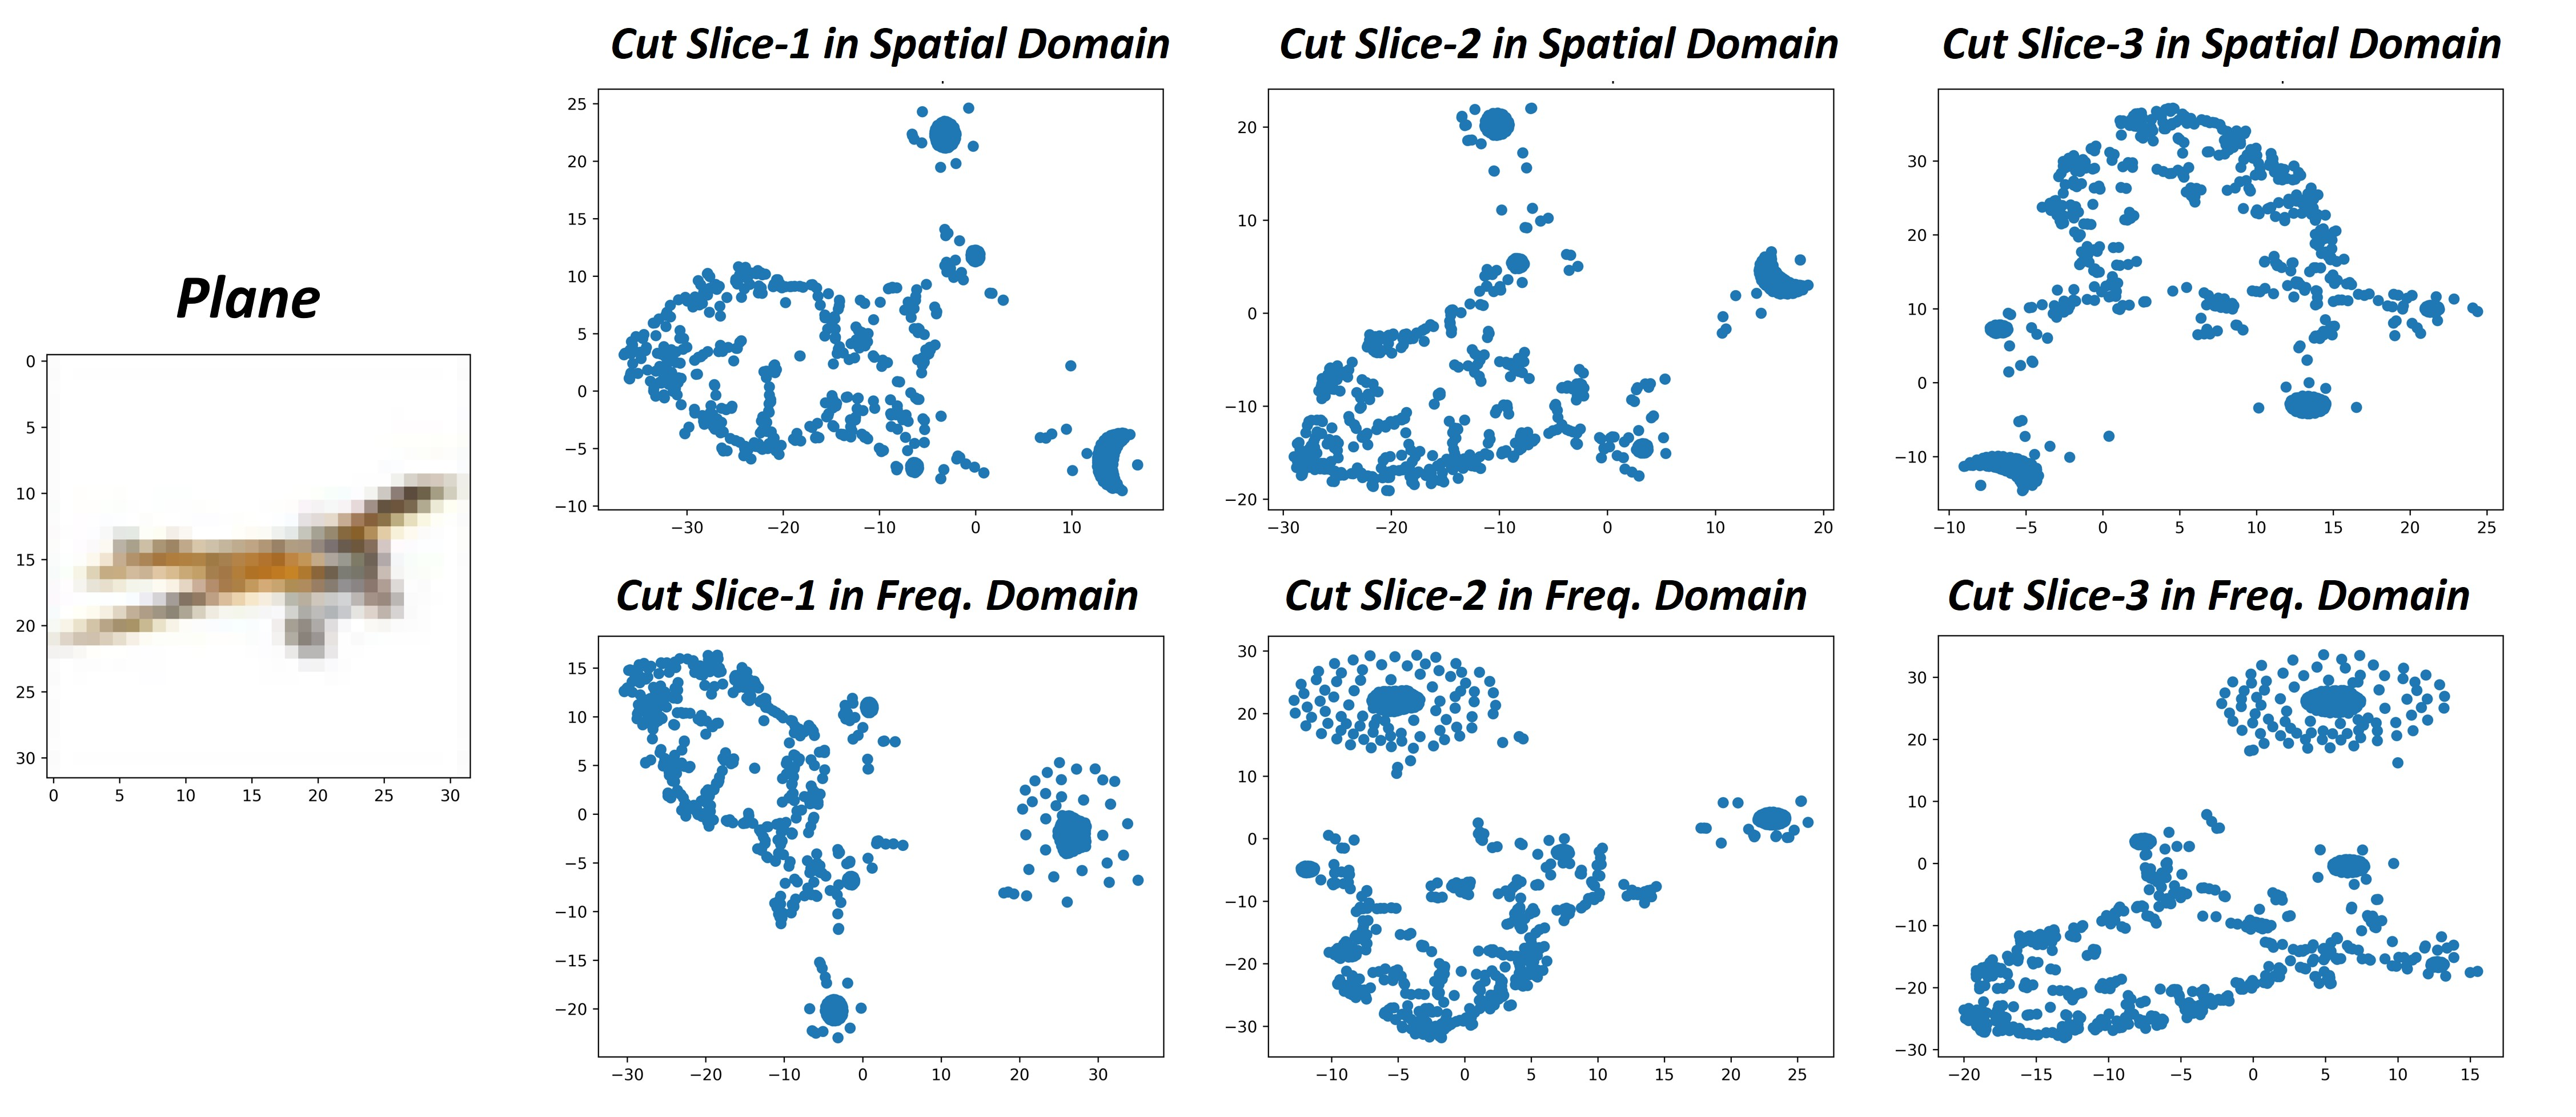}

\centering
\includegraphics[scale=0.45]{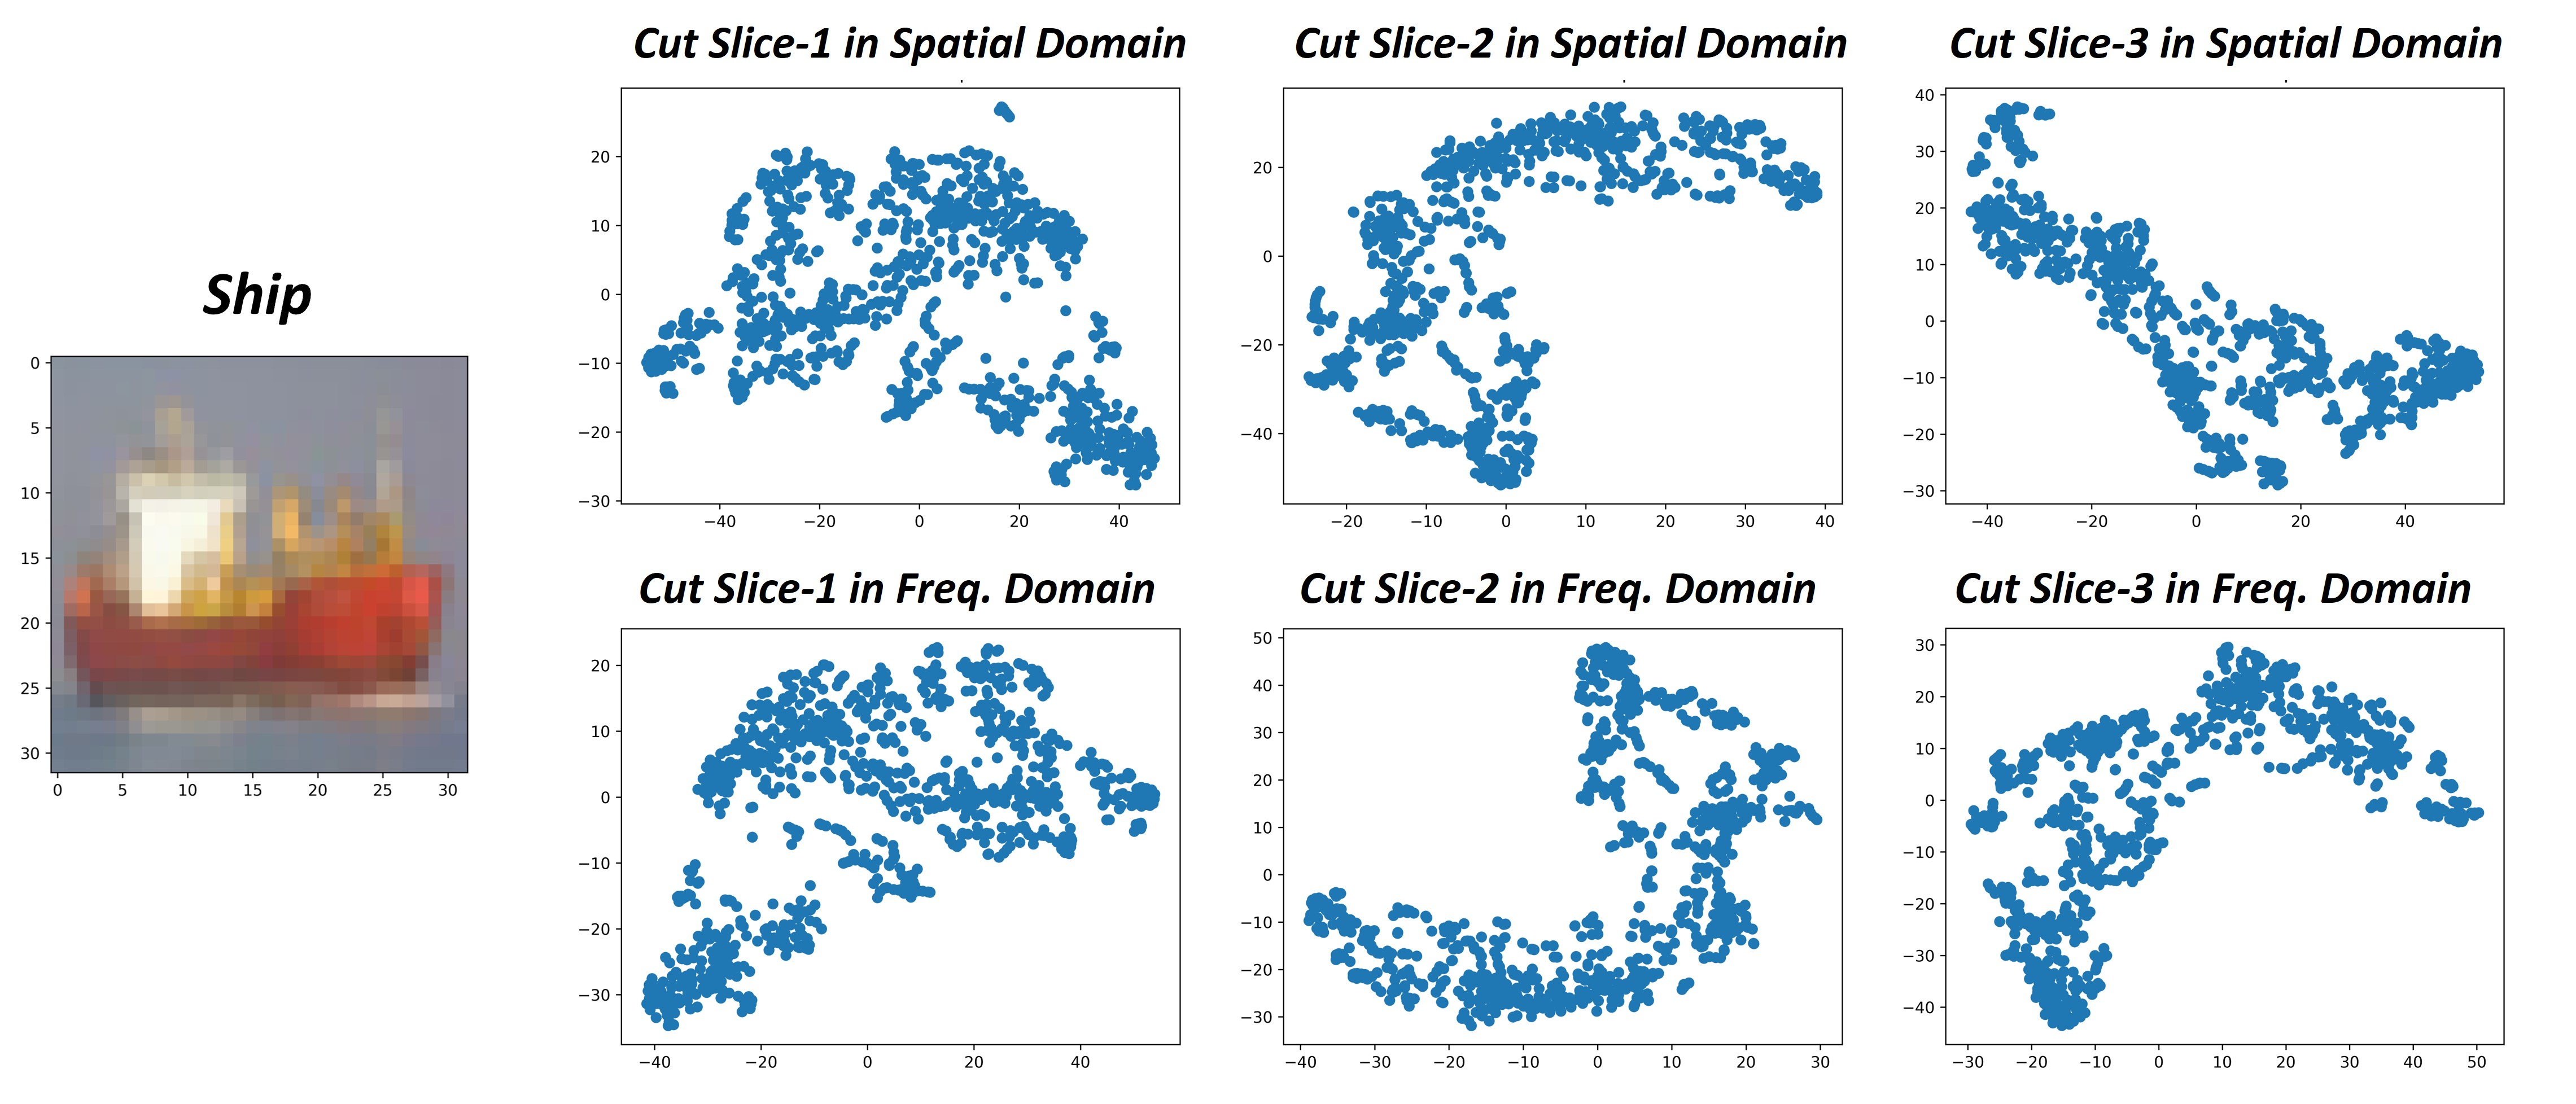}
\caption{Visualization results of the flattened input obtained by $\rm{im2col}$ operation. For each image, there are six sub-figures. The three sub-figures in the first row are flattened inputs of three input channels mapped by t-SNE, respectively. On the other hand, the three sub-figures in the second row show the flattened inputs of three input channels transformed by WHT first and mapped by t-SNE next.}
\label{fig:tsne}
\end{figure*}

Figure~\ref{fig:dog_spatial} and \ref{fig:dog_freq} visualize the comparison results in step 7.

\begin{figure*}
\centering
\includegraphics[scale=0.55]{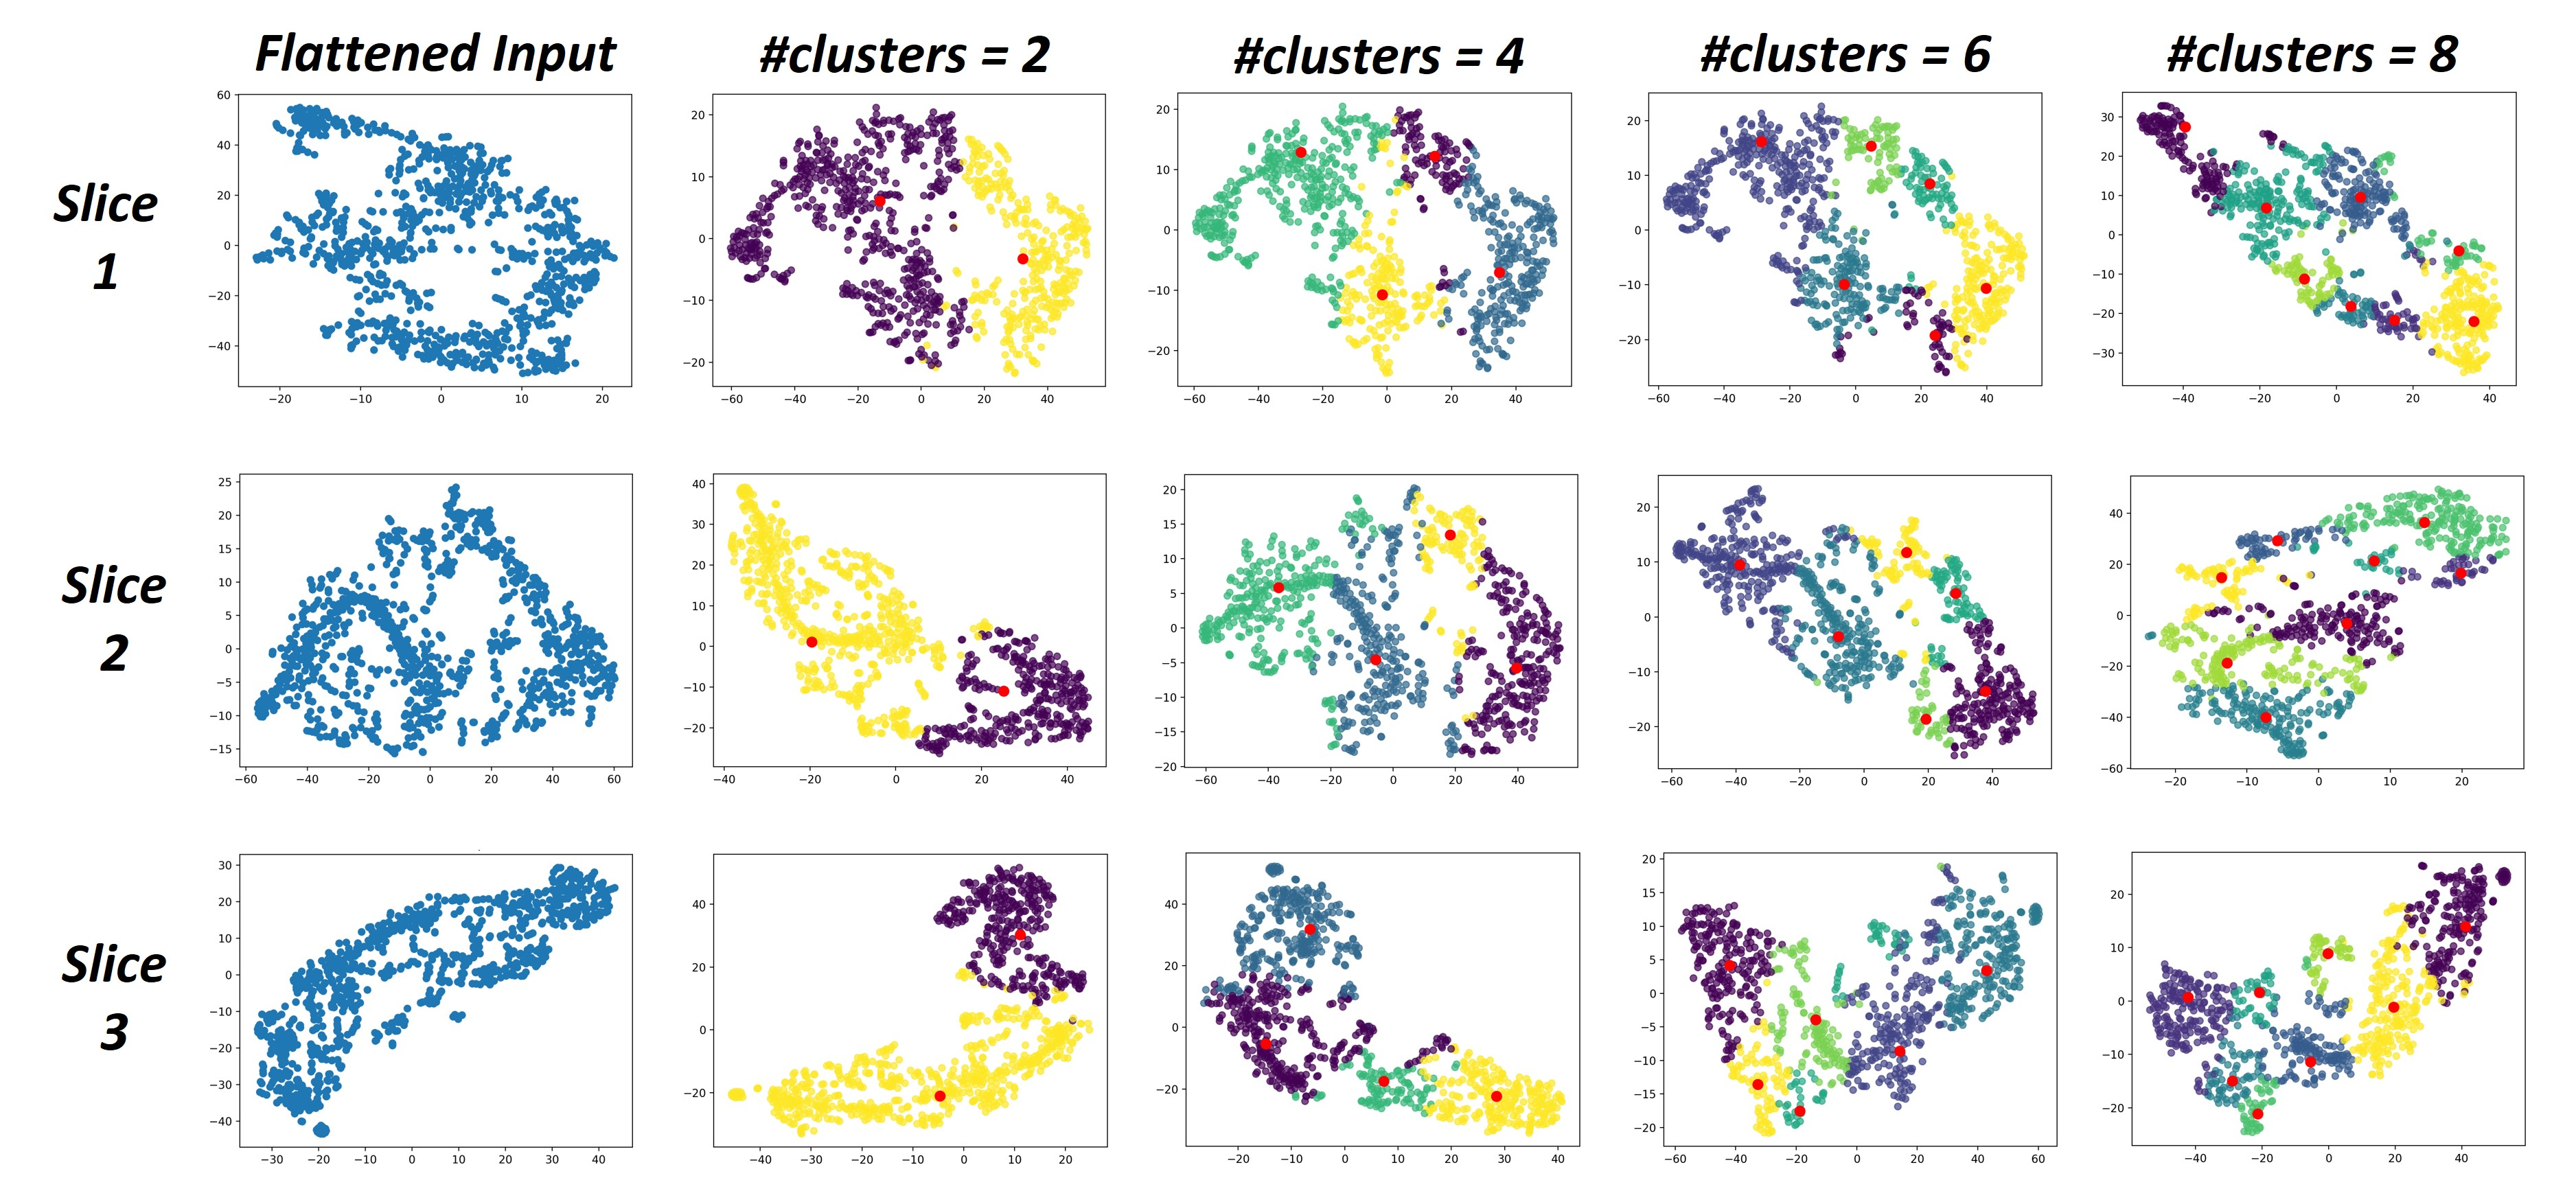}
\caption{Visualization results of three bands in the flattened input in the spatial domain. The three sub-figures in the first column are flattened input in the spatial domain visualized by t-SNE. To draw the sub-figures in the second column, we first fix the number of clusters to be two, and then use k-means to find out the centers and assign labels to each sample. Next, we use t-SNE to visualize all samples and the centers. The same color marks samples assigned to the same prototype, and the centers (prototypes) are marked in red. The approaches to draw the third to fifth columns are similar with the way to draw the second column, except the number of clusters varies.}
\label{fig:dog_spatial}

\centering
\includegraphics[scale=0.55]{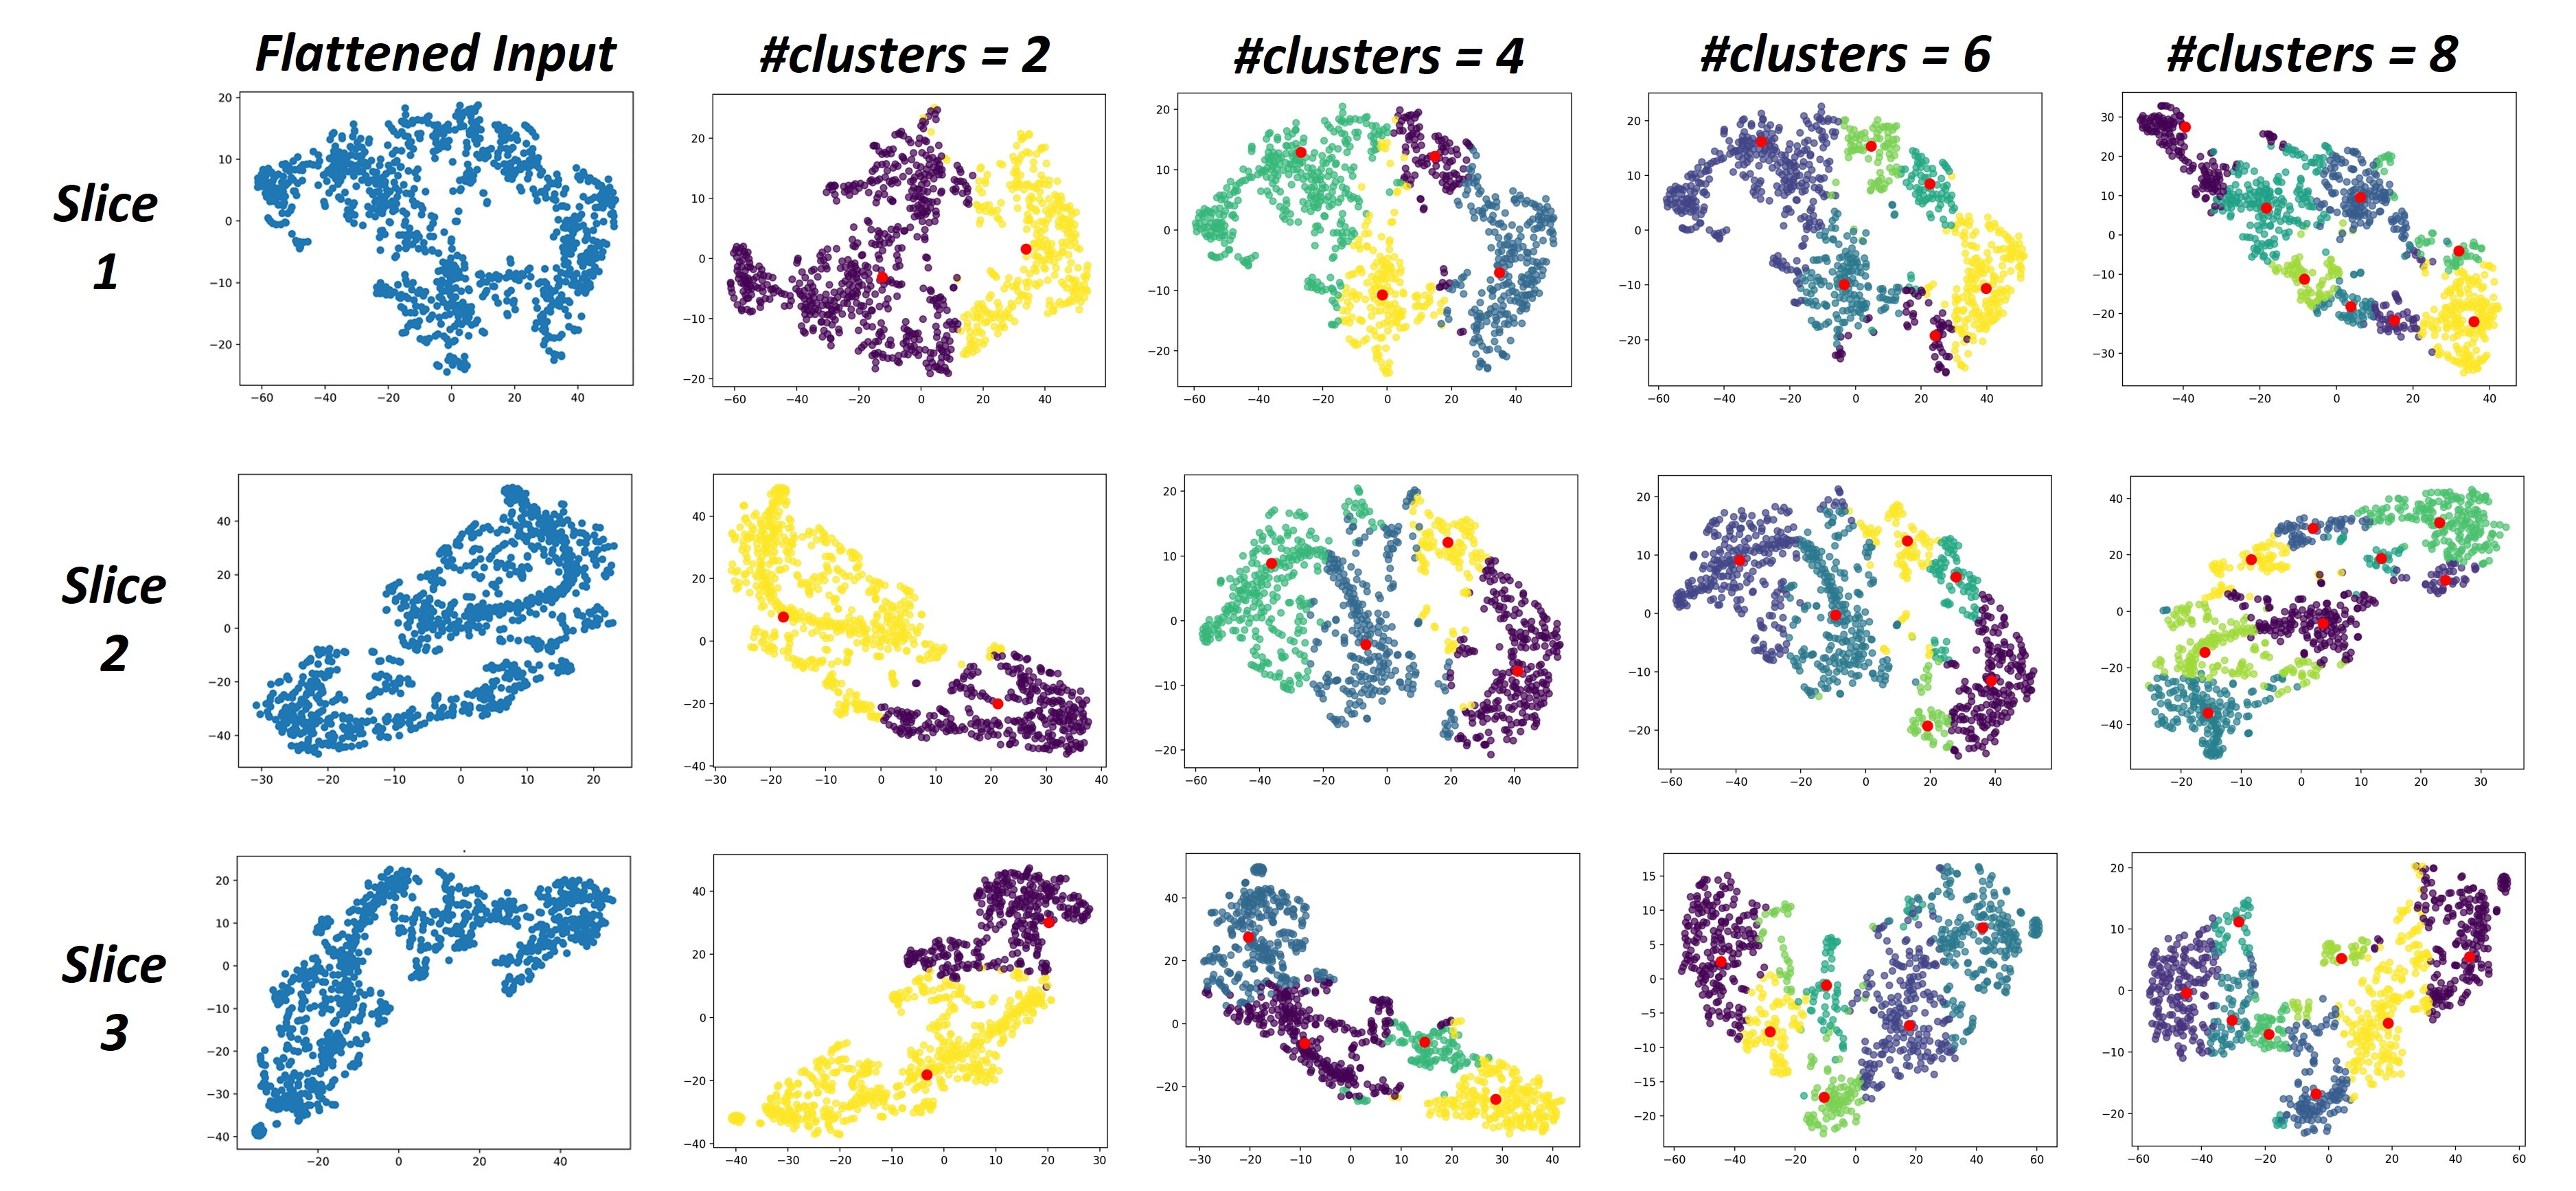}
\caption{Visualization results of three bands in the flattened input in the frequency domain mapped by WHT operation. The three sub-figures in the first column are flattened input in the frequency domain visualized by t-SNE. To draw the sub-figures in the second column, we first fix the number of clusters to be two, and then use k-means to find out the centers and assign labels to each sample. Next, we use t-SNE to visualize all samples and the centers. The same color marks samples assigned to the same prototype, and the centers (prototypes) are marked in red. The approaches to draw the third to fifth columns are similar with the way to draw the second column, except the number of clusters varies.}
\label{fig:dog_freq}
\end{figure*}

Figure~\ref{fig:l1_norm} verifies that l1-norm can be employed to assign prototypes (step 8).

\begin{figure*}
\centering
\includegraphics[scale=0.48]{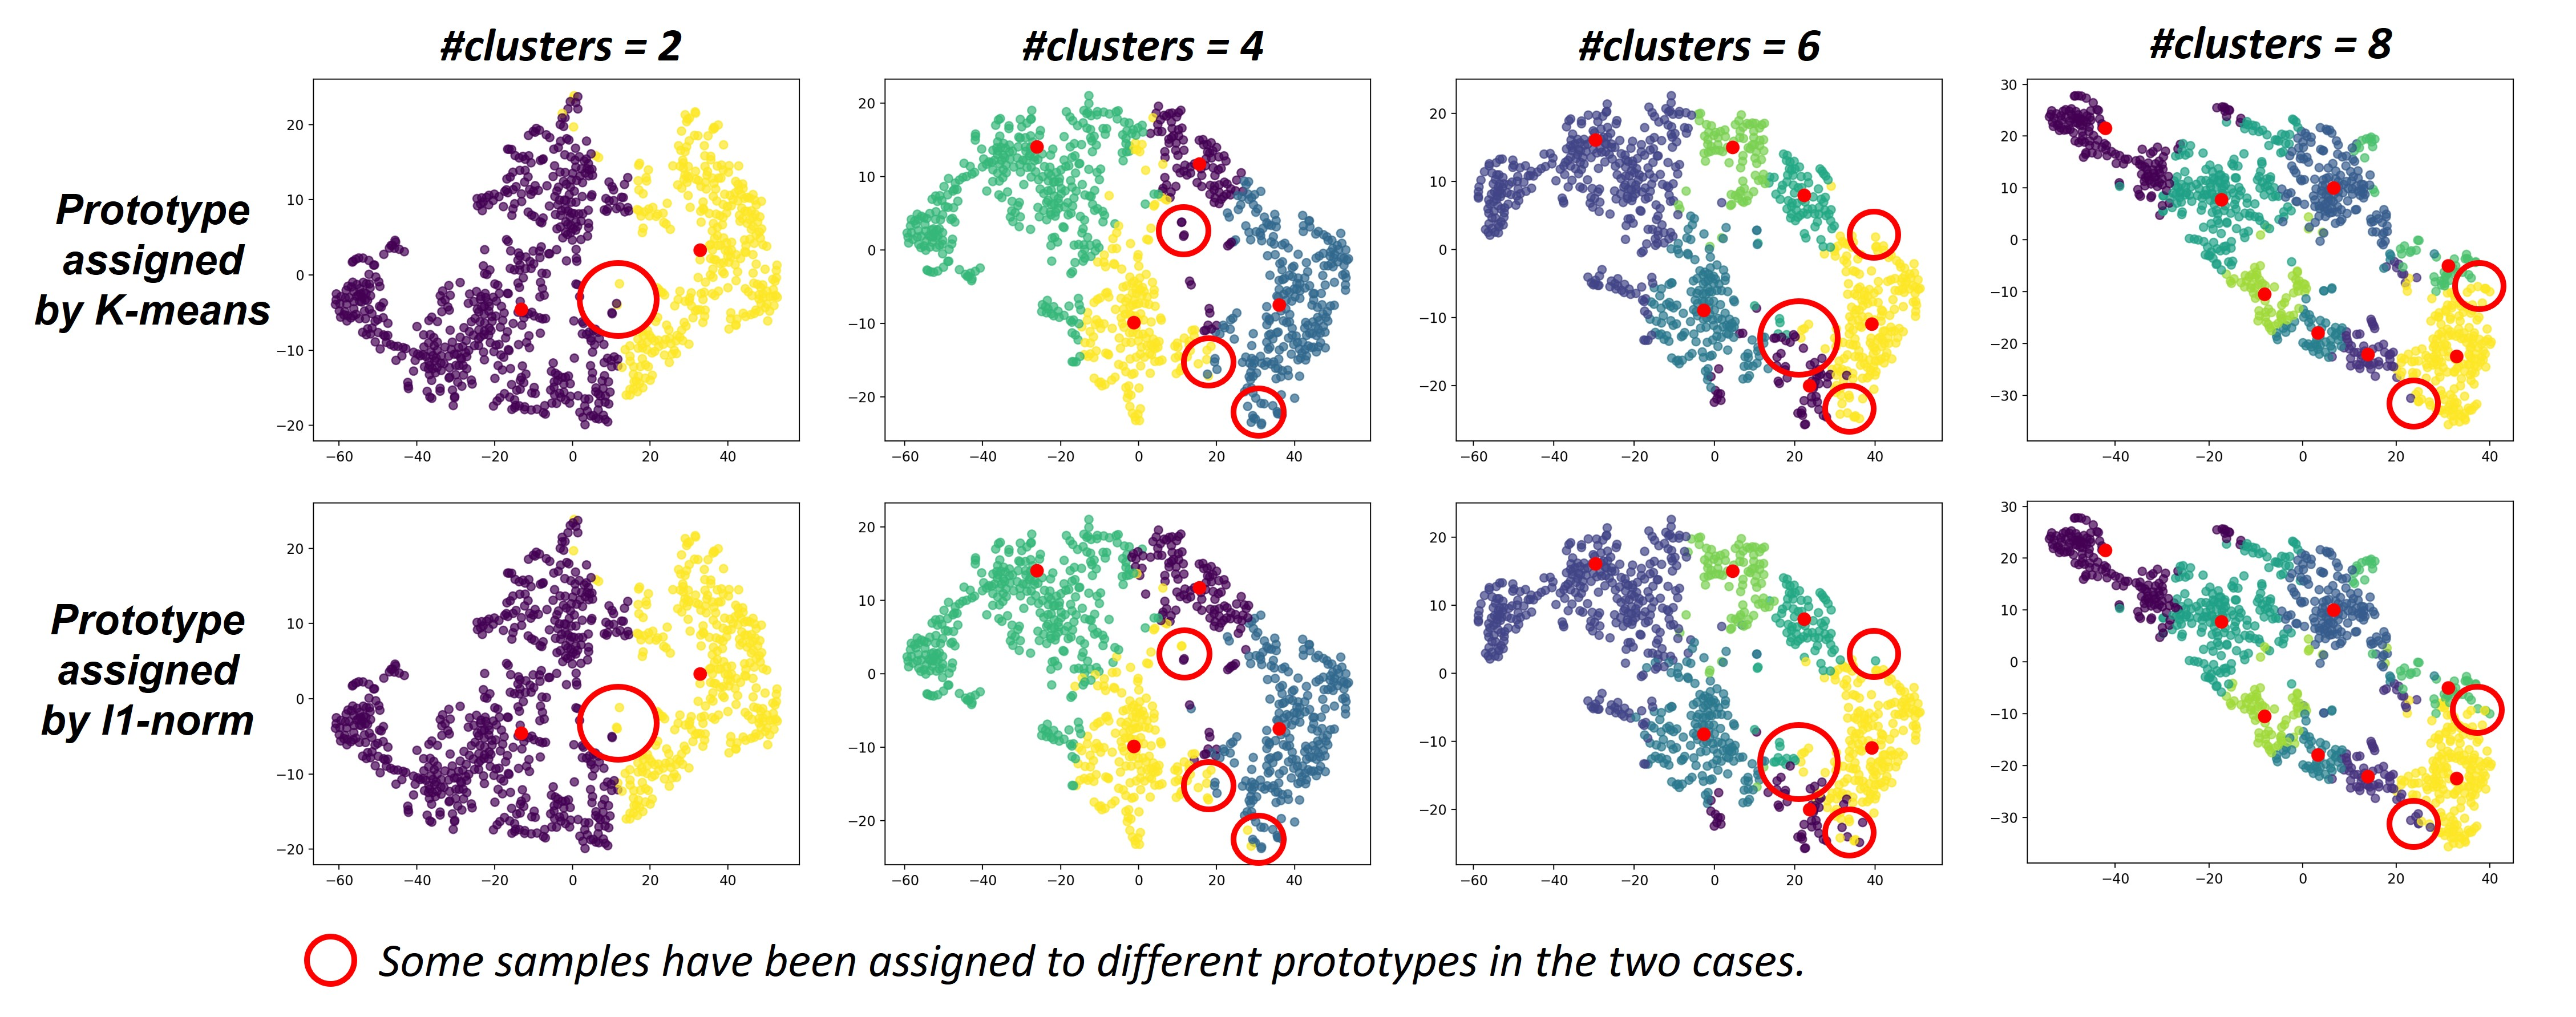}
\caption{Results of prototype assignments done by K-means and l1-norm, respectively. The red circles mark the samples have been assigned to different prototypes in the two cases.}
\label{fig:l1_norm}
\end{figure*}

%%%% WHT experiments %%%%
\section{L1-Norm based prototype assignment Verification}
{\color{red}{\textbf{Date: 2021.09.16 Thursday \& 2021.09.17 Friday}}}

% l2 and l1 norm
\textbf{L2 and L1 Norm in the Spatial and Spectral Domain}


\begin{align}
||H(x - y)||_2^2 & = \sum_{i=1}^{n}\left(h_{i,:}  (x-y)\right)^2 \\ &= \sum_{i=1}^n(x-y)^T \cdot h_{i,:}^T \cdot h_{i,:} \cdot (x-y), \\ &h_{i,:}^T \cdot h_{i,:} = 1
\label{eq:l2_1}
\end{align}


\begin{equation}
||H(x-y)||_2 = ||x-y||_2
\label{eq:l2_2}
\end{equation}

\begin{align}
 ||H(x-y)||_1^2 & = \sum_{i=1}^n |h_{i,:} (x-y)| \\  \sum_{i=1}^n |\sum_{j=1}^m h_{ij} (x_j - y_j)| &\leq \sum_{i=1}^n \sum_{j=1}^m |h_{ij} (x_j - y_j)|, \\ h_{ij} & =1 \text{ or } -1
\label{eq:l1_1}
\end{align}

\begin{equation}
||H(x-y)||_1 \leq ||x-y||_1
\label{eq:l1_2}
\end{equation}

According to equation~\ref{eq:l2_1} to \ref{eq:l1_2}, if there are two given vectors in the spatial domain, their l2 distances in the spatial and spectral domain are equivalent when Hadamard matrix is employed to do the mapping. On the other hand, their l1 distances in the two domains varies.

The results shown in Section~\ref{sec:WHT_preliminary} are obtained by a single image selected in CIFAR-10. To get more solid conclusion, we increase the batch size to 10. Therefore, the size of each band changes from $[9, 900]$ to $[9, 9000]$.

%%%%%%%%%% part 1 %%%%%%%%%%
\textbf{Different Prototype Assignments Rates}

Table~\ref{tab:l1_mismatching} displays the mismatching rate when the prototypes are assigned by L2-norm and L1-norm, respectively.

\setlength{\tabcolsep}{5mm}{
\begin{table*}[htbp]
\scriptsize
\centering
\begin{tabular}{ccccccccc}
\toprule
\#Clusters & 2 & 4 & 6 & 8 & 10 & 12 & 14 & 16 \\
\midrule
Slice 1 & $0.61\%$ & $0.77\%$ & $6.79\%$ & $7.86\%$ & $8.46\%$ & $8.22\%$ & $6.92\%$ & $7.38\%$ \\
Slice 2 & $0.67\%$ & $0.70\%$ & $5.64\%$ & $6.42\%$ & $7.33\%$ & $7.59\%$ & $6.91\%$ & $7.38\%$ \\
Slice 3 & $0.64\%$ & $0.79\%$ & $1.86\%$ & $5.53\%$ & $5.93\%$ & $6.60\%$ & $6.96\%$ & $6.78\%$ \\
\midrule
Avg. Mismatching Rate & $0.65\%$ & $0.72\%$ & $5.36\%$ & $6.90\%$ & $7.71\%$ & $7.80\%$ & $6.91\%$ & $7.38\%$ \\
\bottomrule
\end{tabular}
\caption{We compare the prototypes assigned by \textbf{L1-norm} and \textbf{L2-norm}, respectively. The table shows the mismatching rates for samples in each slice (band) under different numbers of clusters when employing K-means to find the prototypes. The bottom row is the average mismatching rate under different cases.}
\label{tab:l1_mismatching}
\end{table*}}

%%%%%%%%%% part 2 %%%%%%%%%%
\textbf{Histogram of Centers and Selected Neighbor Samples}

Figure~\ref{fig:slice1_l1} to Figure~\ref{fig:slice3_l2_spatial} display histograms of the centers (prototypes) of different clusters decided by K-means $(K=8)$ and we also show the histograms of three selected neighbor samples of each center. Table~\ref{tab:histo_info} summarizes the information of the figures. Figure~\ref{fig:slice1_l1} to \ref{fig:slice3_l1} show the histograms of eight prototypes and their neighbors in band 1 to 3, respectively. The bands are transformed by WHT in the spectral domain, and the prototypes are assigned by L1-norm distance. In Figure~\ref{fig:slice1_l2_spectral} to \ref{fig:slice3_l2_spectral}, the bands are in the spectral domain as well, but the prototypes are assigned by L2-norm distance instead. In Figure~\ref{fig:slice1_l2_spatial} to Figure~\ref{fig:slice3_l2_spatial}, the bands are in the spatial domain, and the prototypes are assigned by L2-norm distance, which is a regular approach employed in most Product Quantization (PQ).

Remarks:
\begin{enumerate}
\item Group 1/2/3: Prototypes and and their neighbors have similar histograms.
\item Group 1/2/3: Prototypes in different clusters have distinct histograms.
\item Compare Group 1 with Group 2: Both L1-distance and L2-distance can assign prototypes properly to the given samples in the spectral domain.
\item Compare Group 1 with Group 3: Using L1-distance in the spectral domain is comparable with using L2-distance in the spatial domain to assign prototypes.
\end{enumerate}

\setlength{\tabcolsep}{1mm}{
\begin{table}[ht]
\scriptsize
\centering
\begin{tabular}{ccccccccc}
\toprule
Group & Figure & Band No. & \#Clusters & \#Neighbors & WHT & L1-norm & L2-norm \\
\midrule
\multirow{3}{*}{1} & \ref{fig:slice1_l1} & 1 & 8 & 3 & \checkmark & \checkmark & ~ \\
~ & \ref{fig:slice2_l1} & 2 & 8 & 3 & \checkmark & \checkmark & ~ \\
~ & \ref{fig:slice3_l1} & 3 & 8 & 3 & \checkmark & \checkmark & ~ \\
\midrule
\multirow{3}{*}{2} & \ref{fig:slice1_l2_spectral} & 1 & 8 & 3 & \checkmark & ~ & \checkmark \\
~ & \ref{fig:slice2_l2_spectral} & 2 & 8 & 3 & \checkmark & ~ & \checkmark \\
~ & \ref{fig:slice3_l2_spectral} & 3 & 8 & 3 & \checkmark & ~ & \checkmark \\
\midrule
\multirow{3}{*}{3} & \ref{fig:slice1_l2_spatial} & 1 & 8 & 3 & ~ & ~ & \checkmark \\
~ & \ref{fig:slice2_l2_spatial} & 2 & 8 & 3 & ~ & ~ & \checkmark \\
~ & \ref{fig:slice3_l2_spatial} & 3 & 8 & 3 & ~ & ~ & \checkmark \\
\bottomrule
\end{tabular}
\caption{Summary of different histogram figures.}
\label{tab:histo_info}
\end{table}}

%%%% L1 spectral
% slice 1
\begin{figure*}[h]
\centering
\includegraphics[scale=0.48]{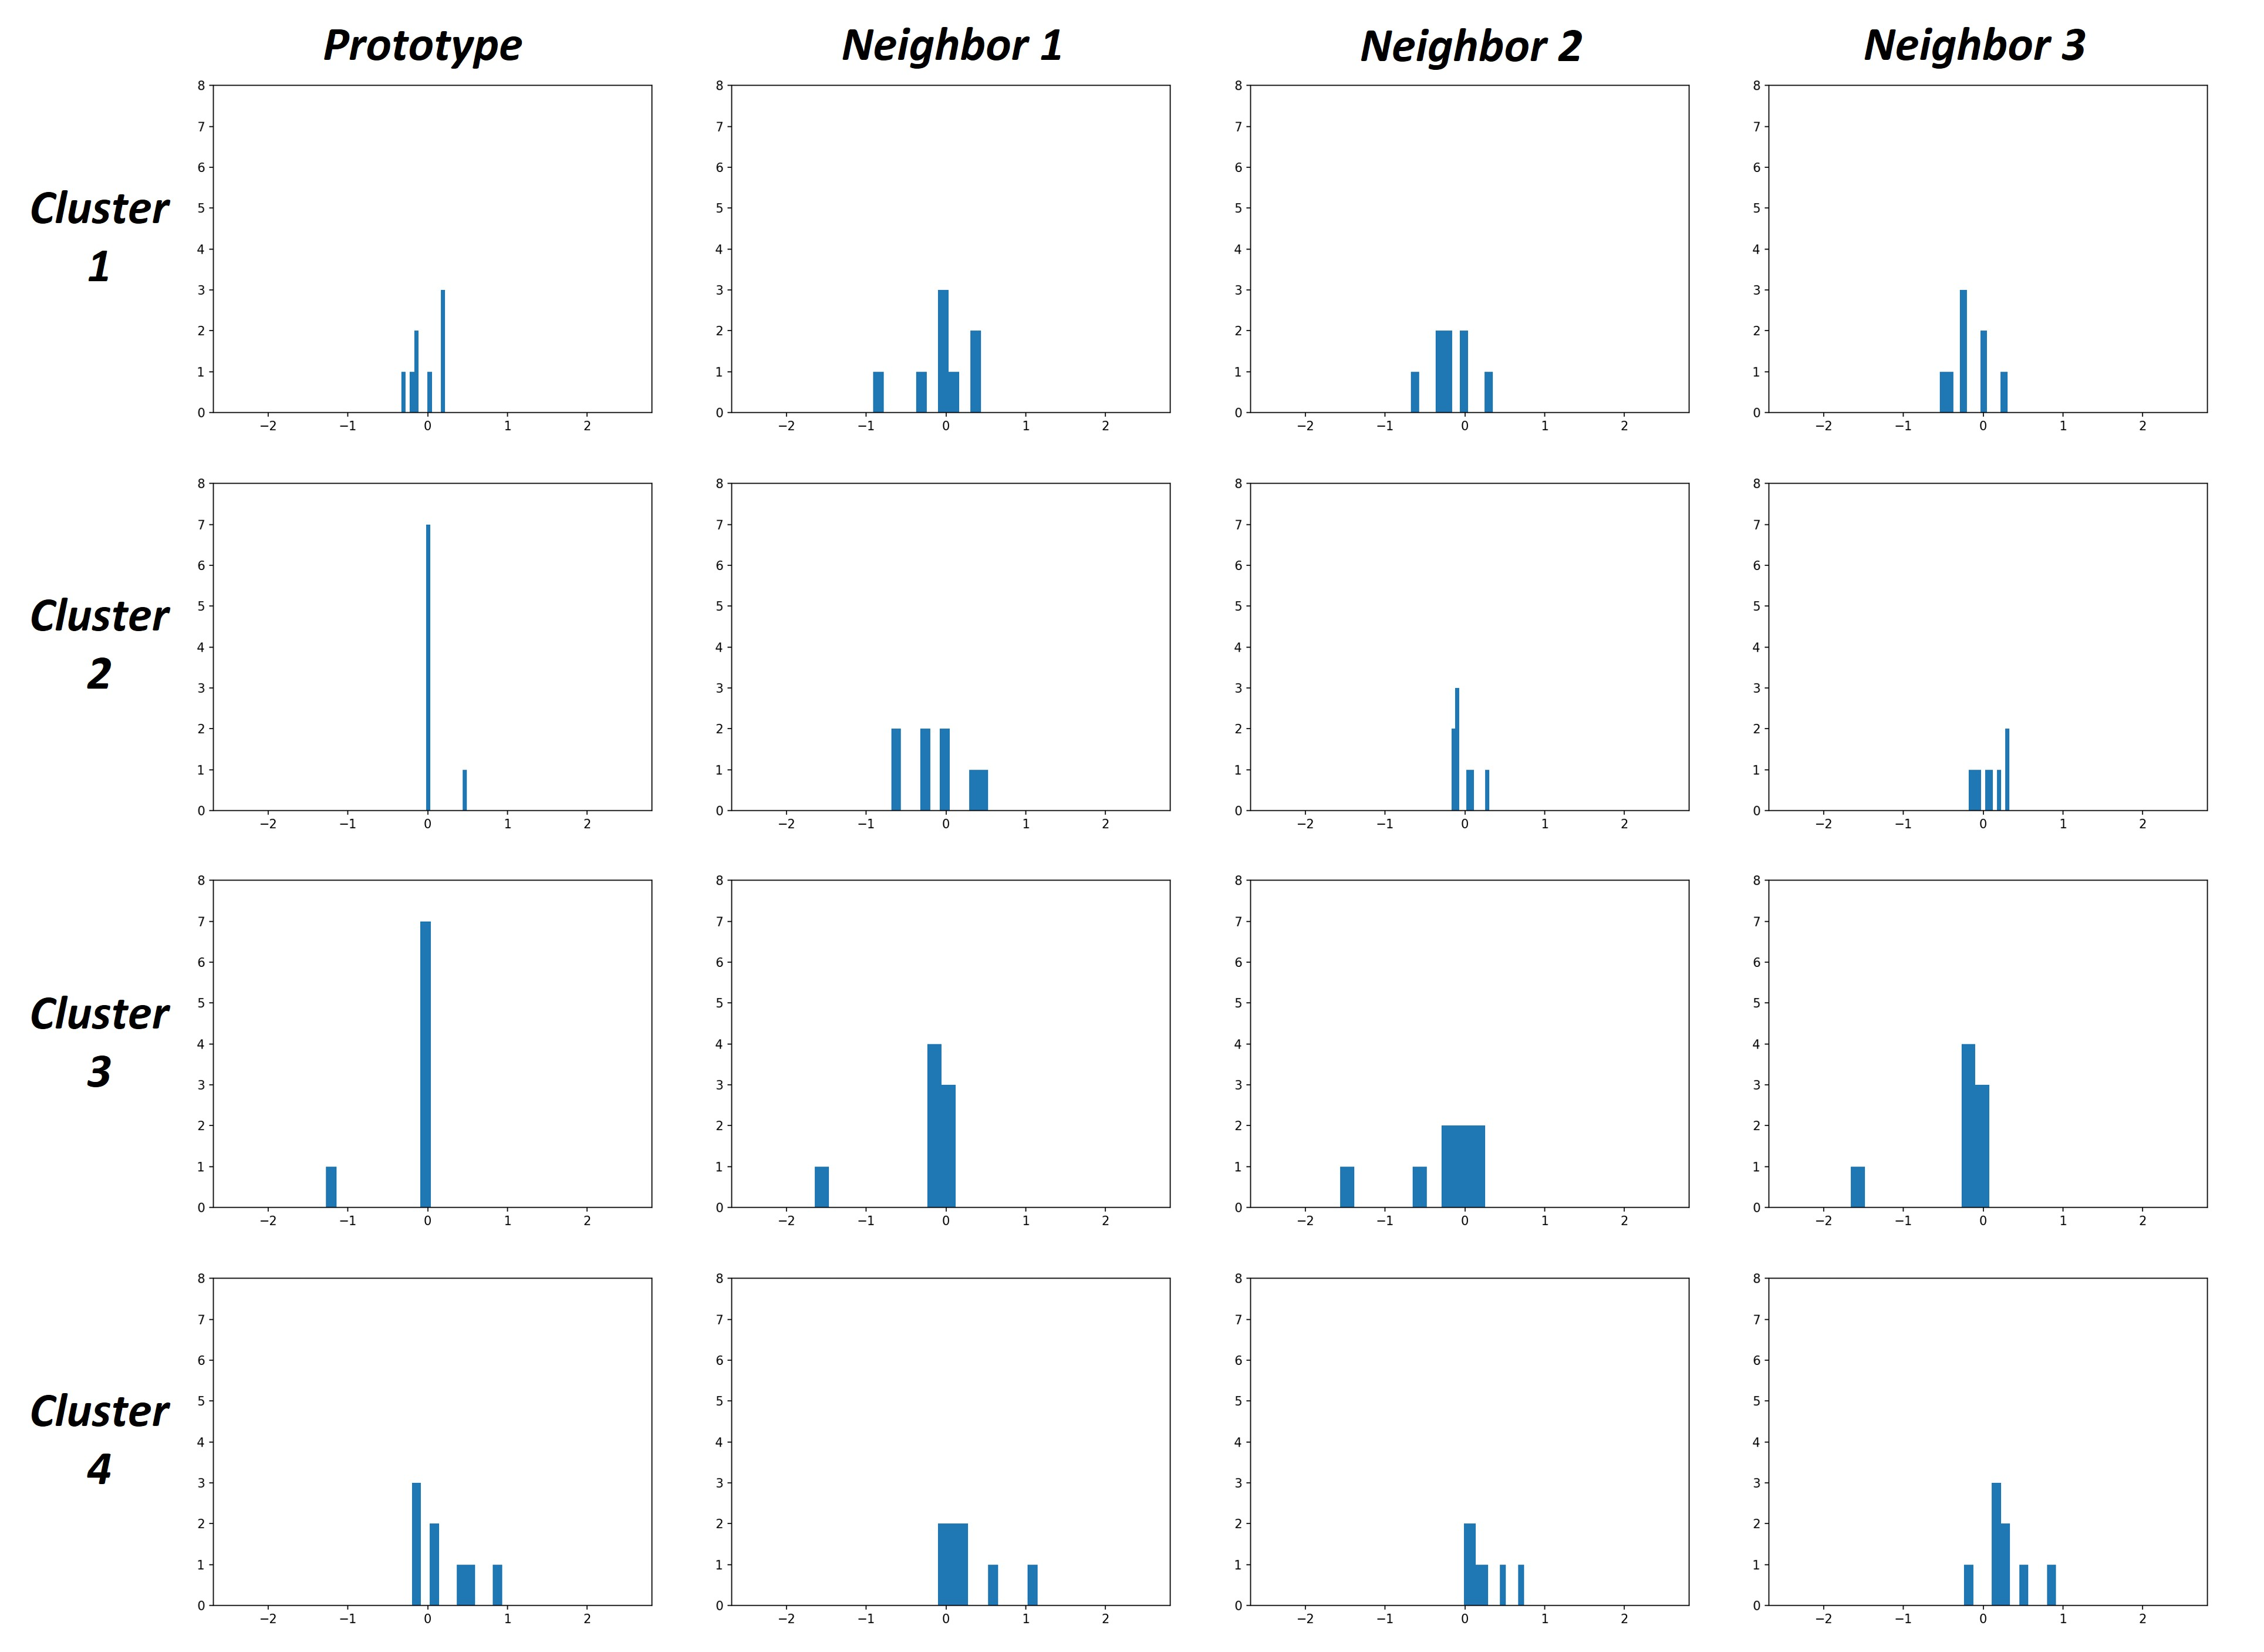}
\centering
\includegraphics[scale=0.48]{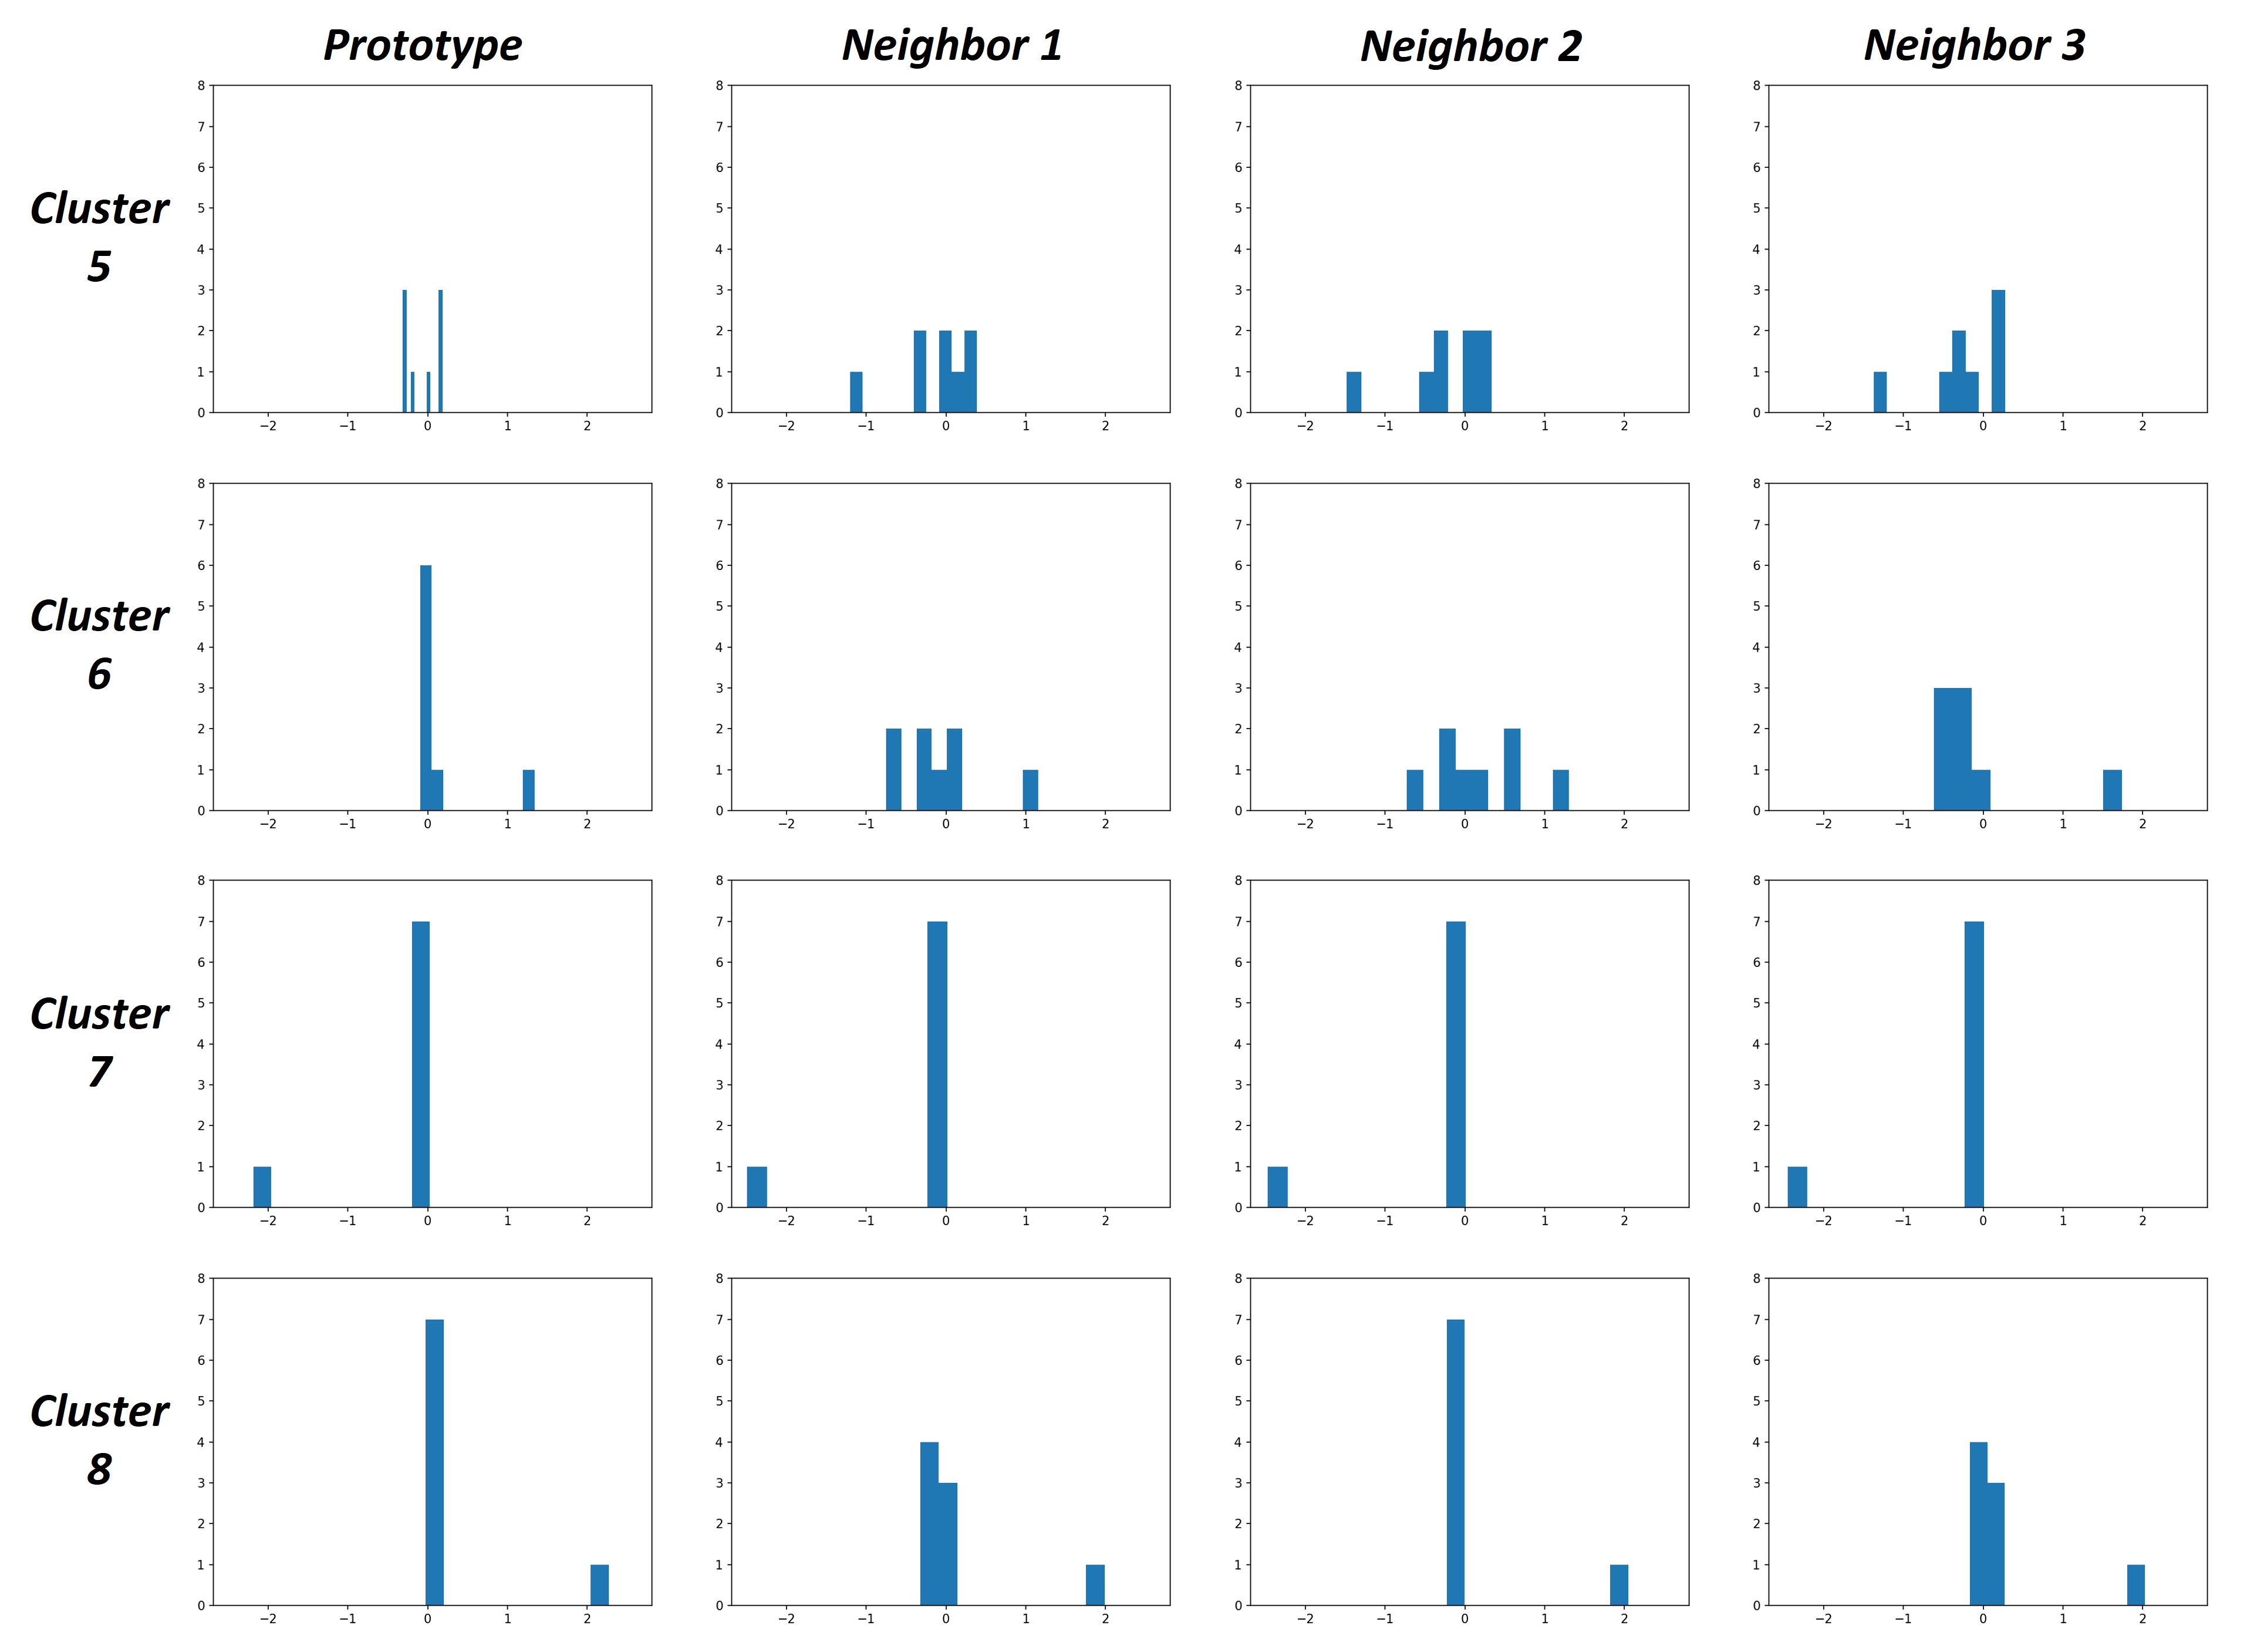}
\caption{The histogram of the eight centers (prototypes) and their neighbors in the \textbf{fist band} of the flattened input. The band is in the \textbf{spectral domain} mapped by WHT, and the prototypes are assigned according to the \textbf{L1-norm distance}.}
\label{fig:slice1_l1}
\end{figure*}

% slice 2
\begin{figure*}[h]
\centering
\includegraphics[scale=0.48]{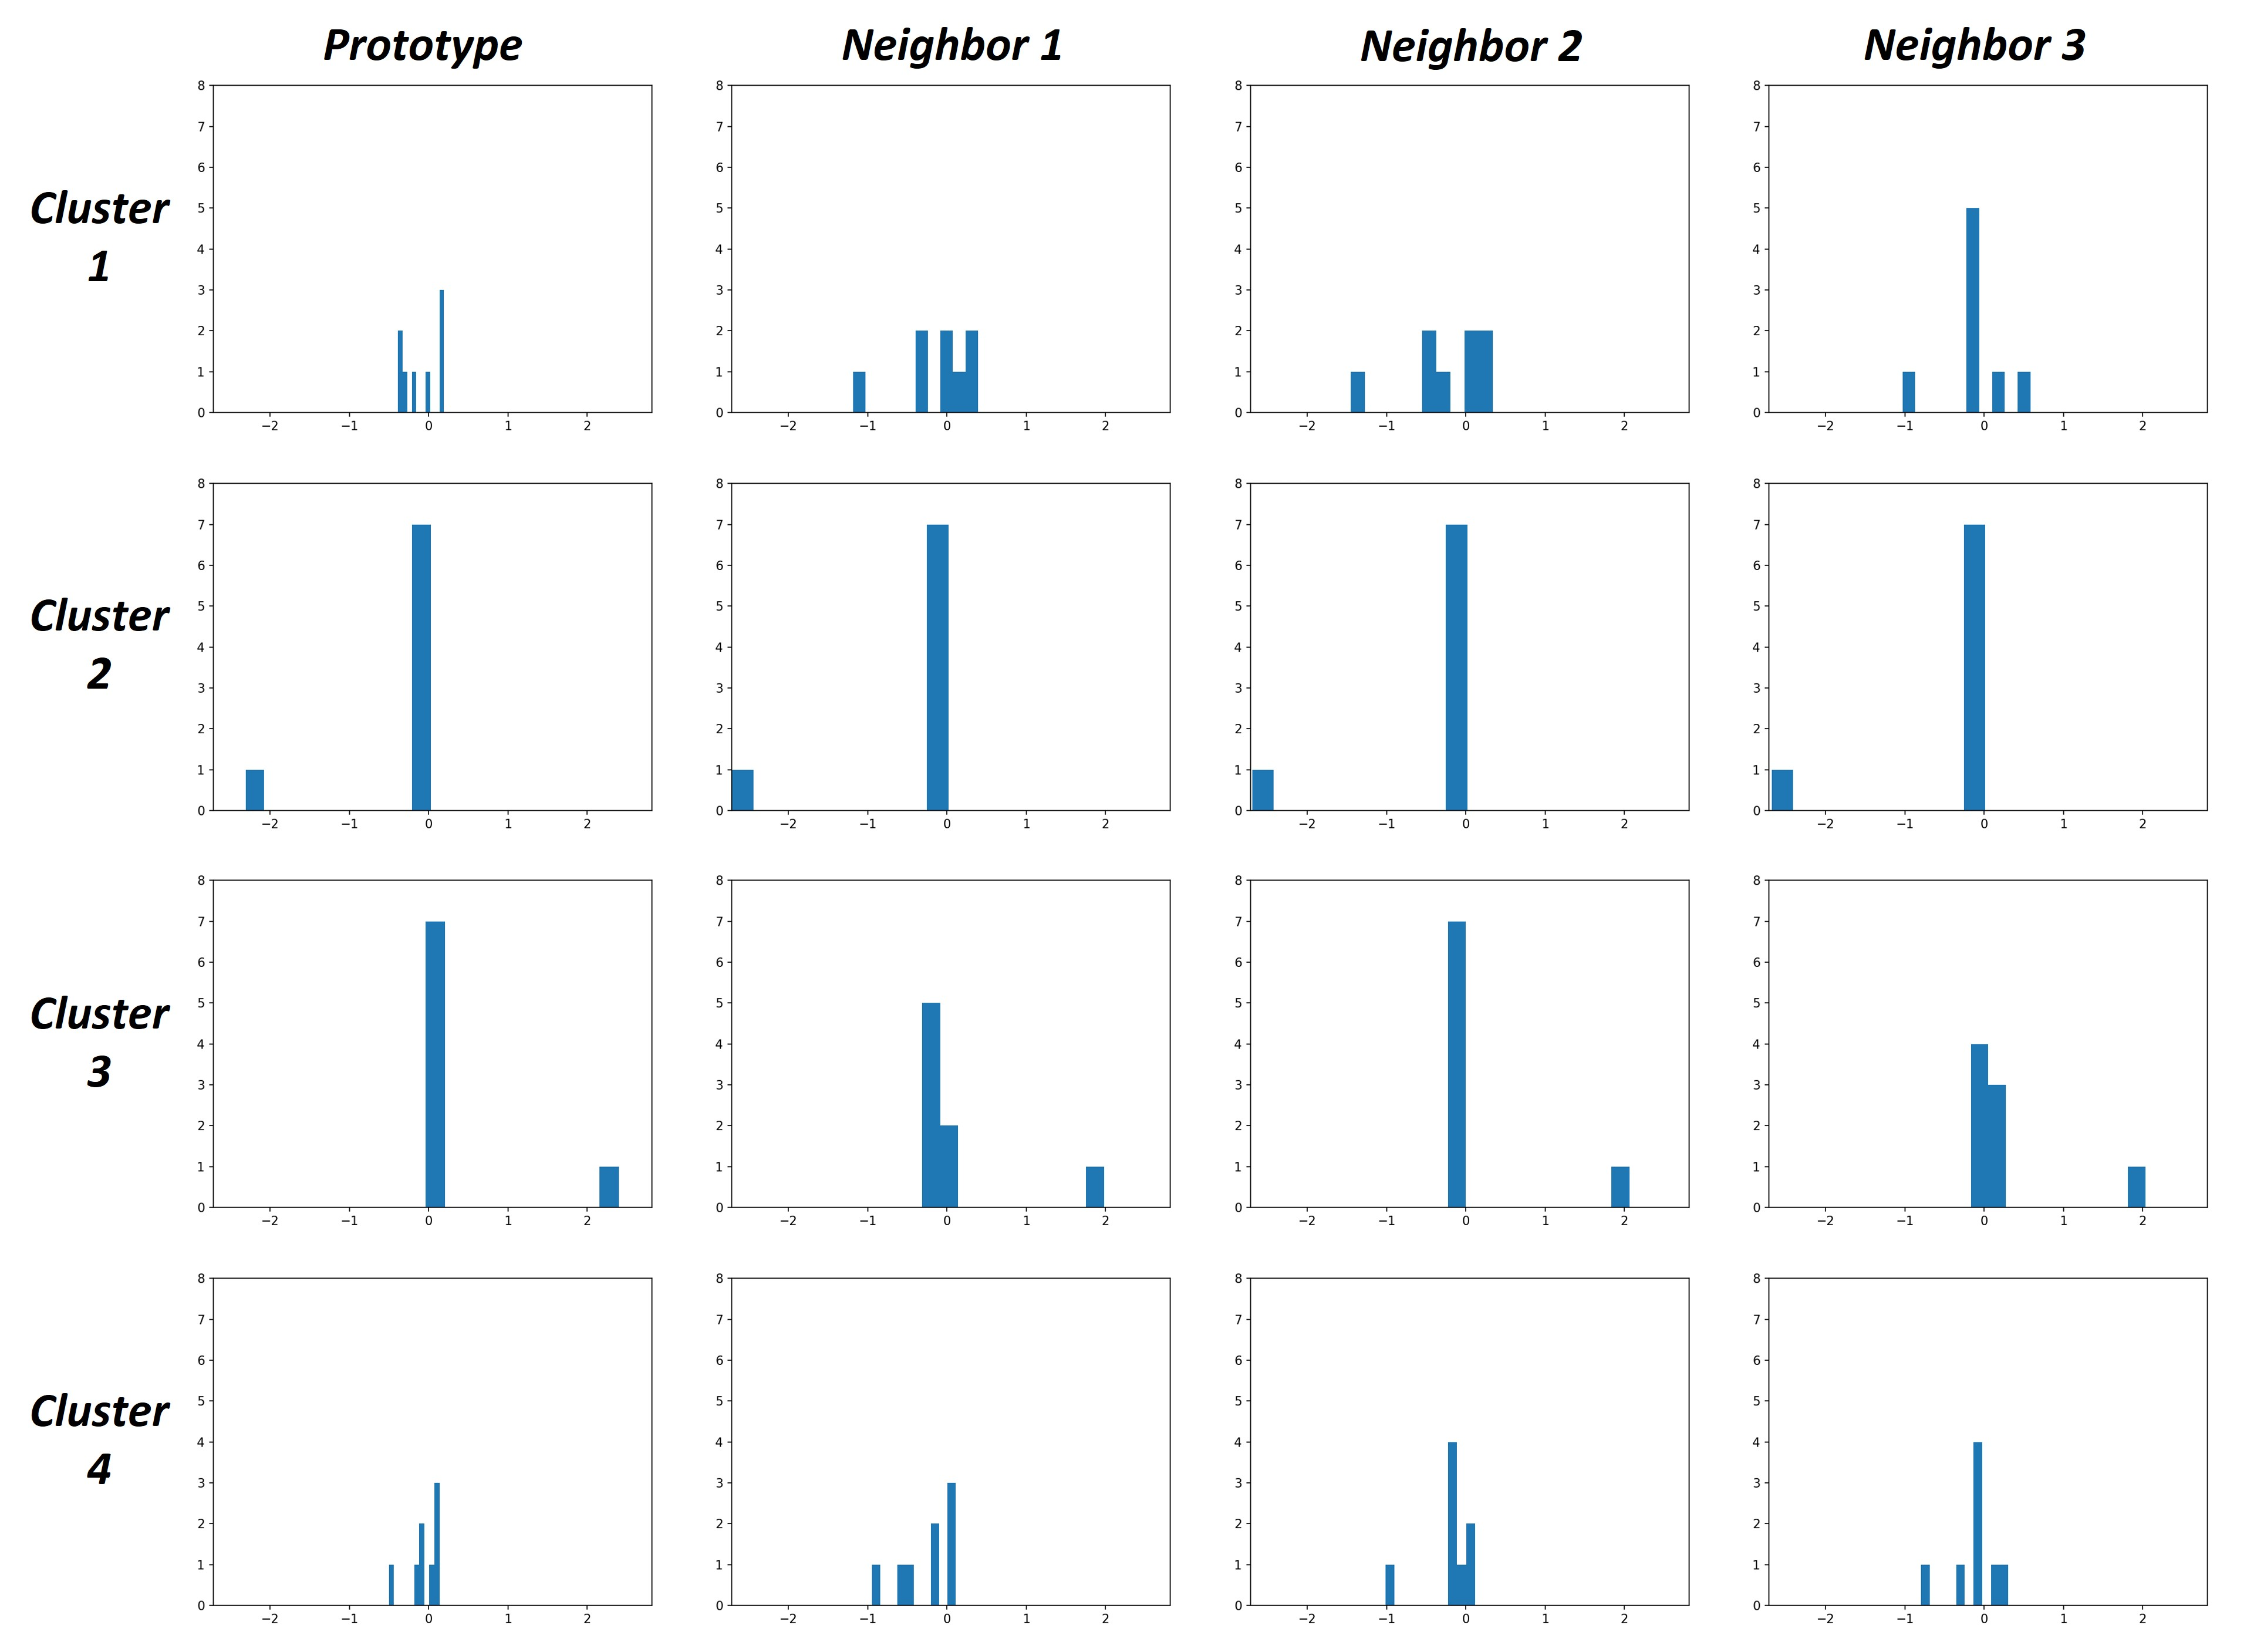}
\centering
\includegraphics[scale=0.48]{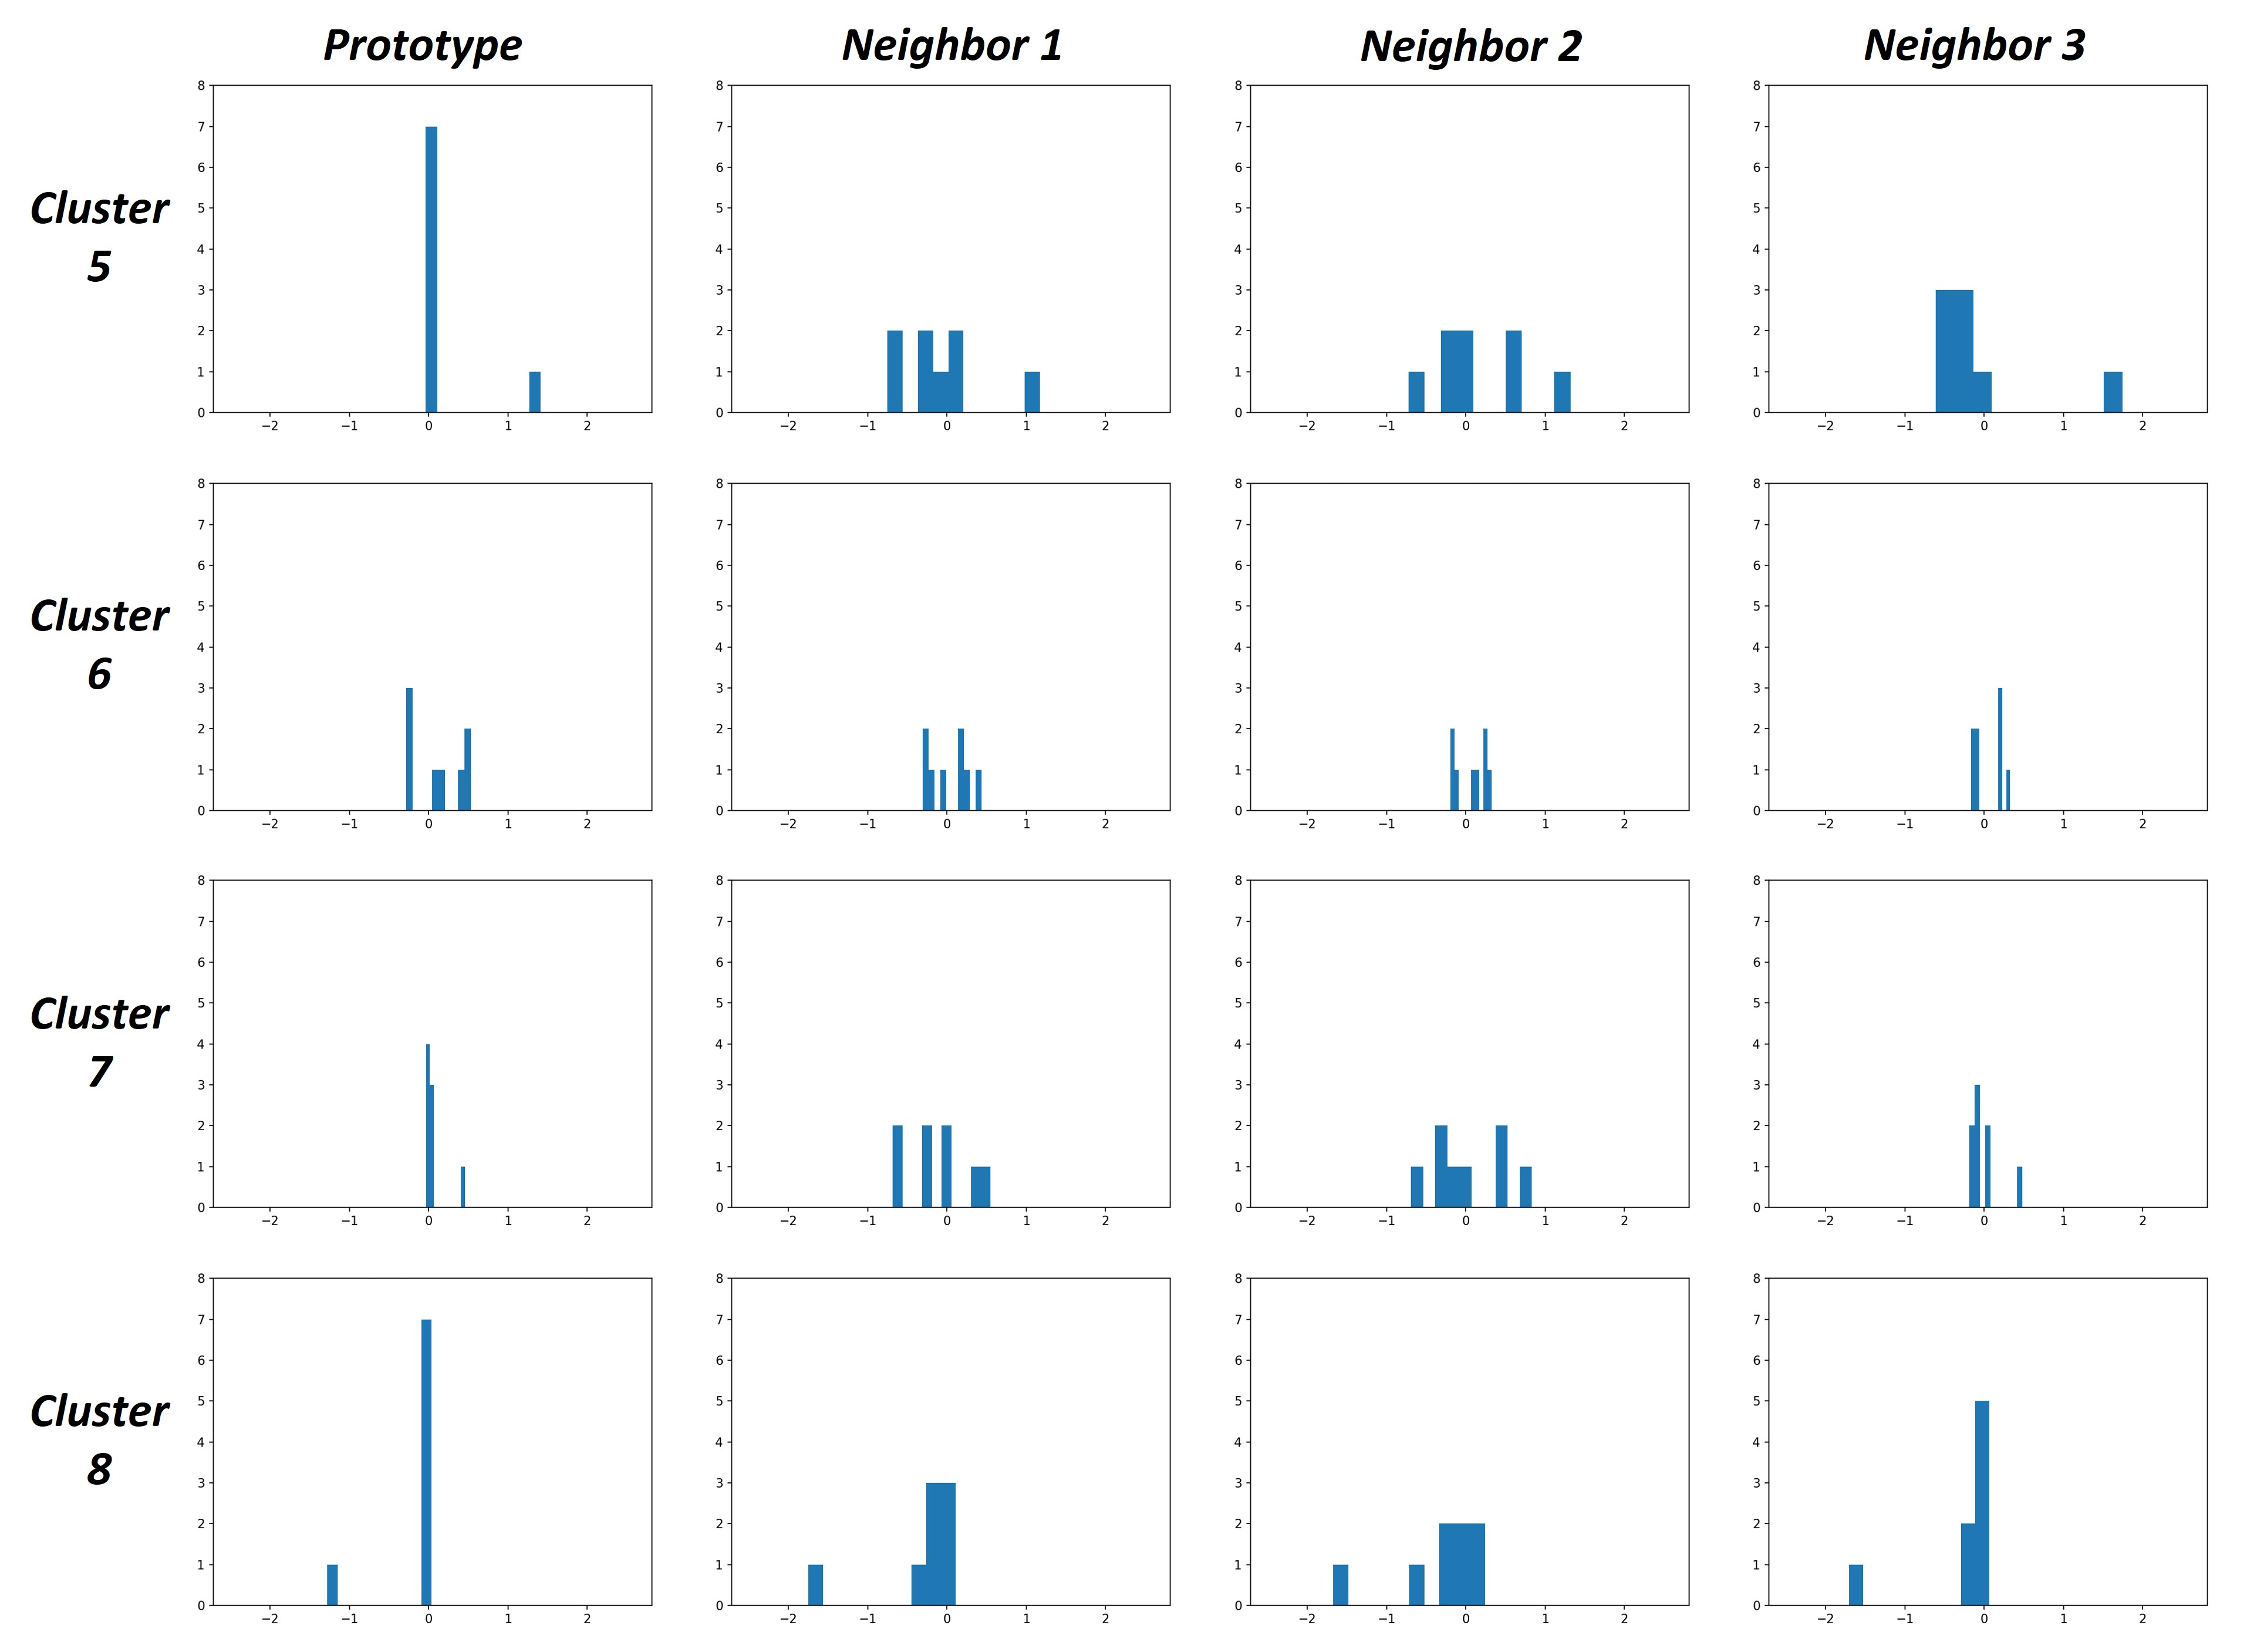}
\caption{The histogram of the eight centers (prototypes) and their neighbors in the \textbf{second band} of the flattened input. The band is in the \textbf{spectral domain} mapped by WHT, and the prototypes are assigned according to the \textbf{L1-norm distance}.}
\label{fig:slice2_l1}
\end{figure*}

% slice 3
\begin{figure*}[h]
\centering
\includegraphics[scale=0.48]{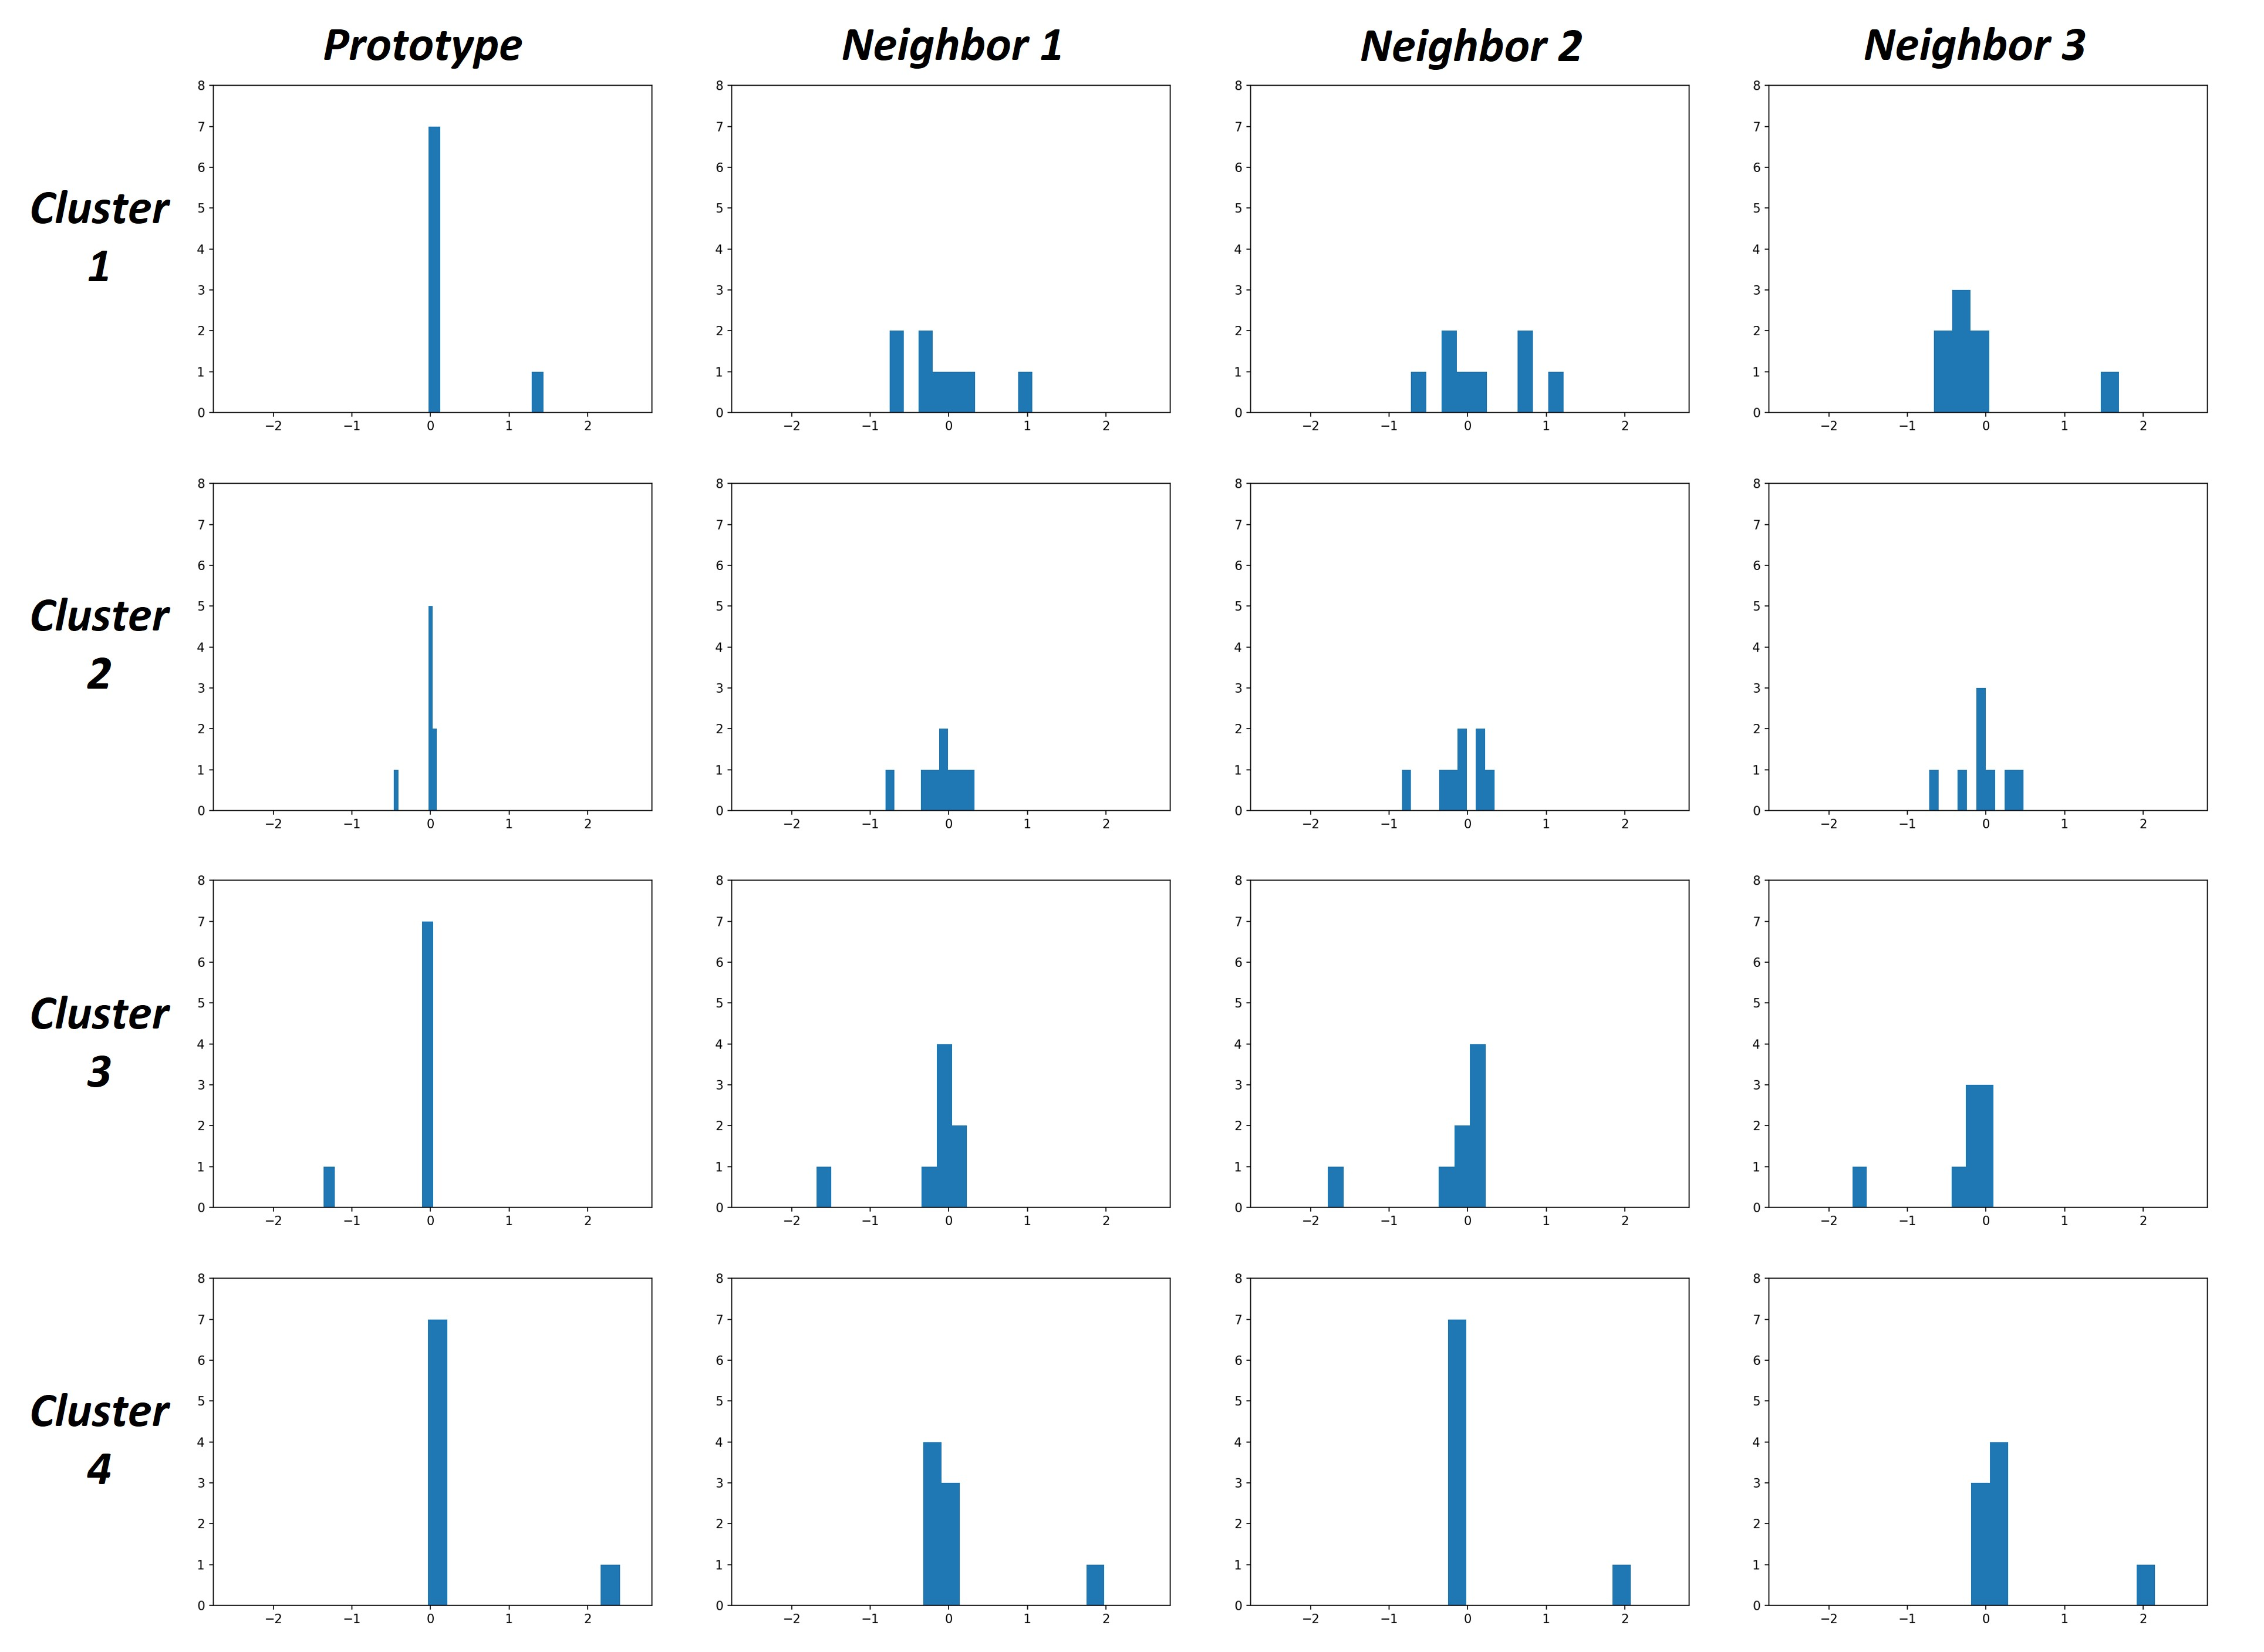}
\centering
\includegraphics[scale=0.48]{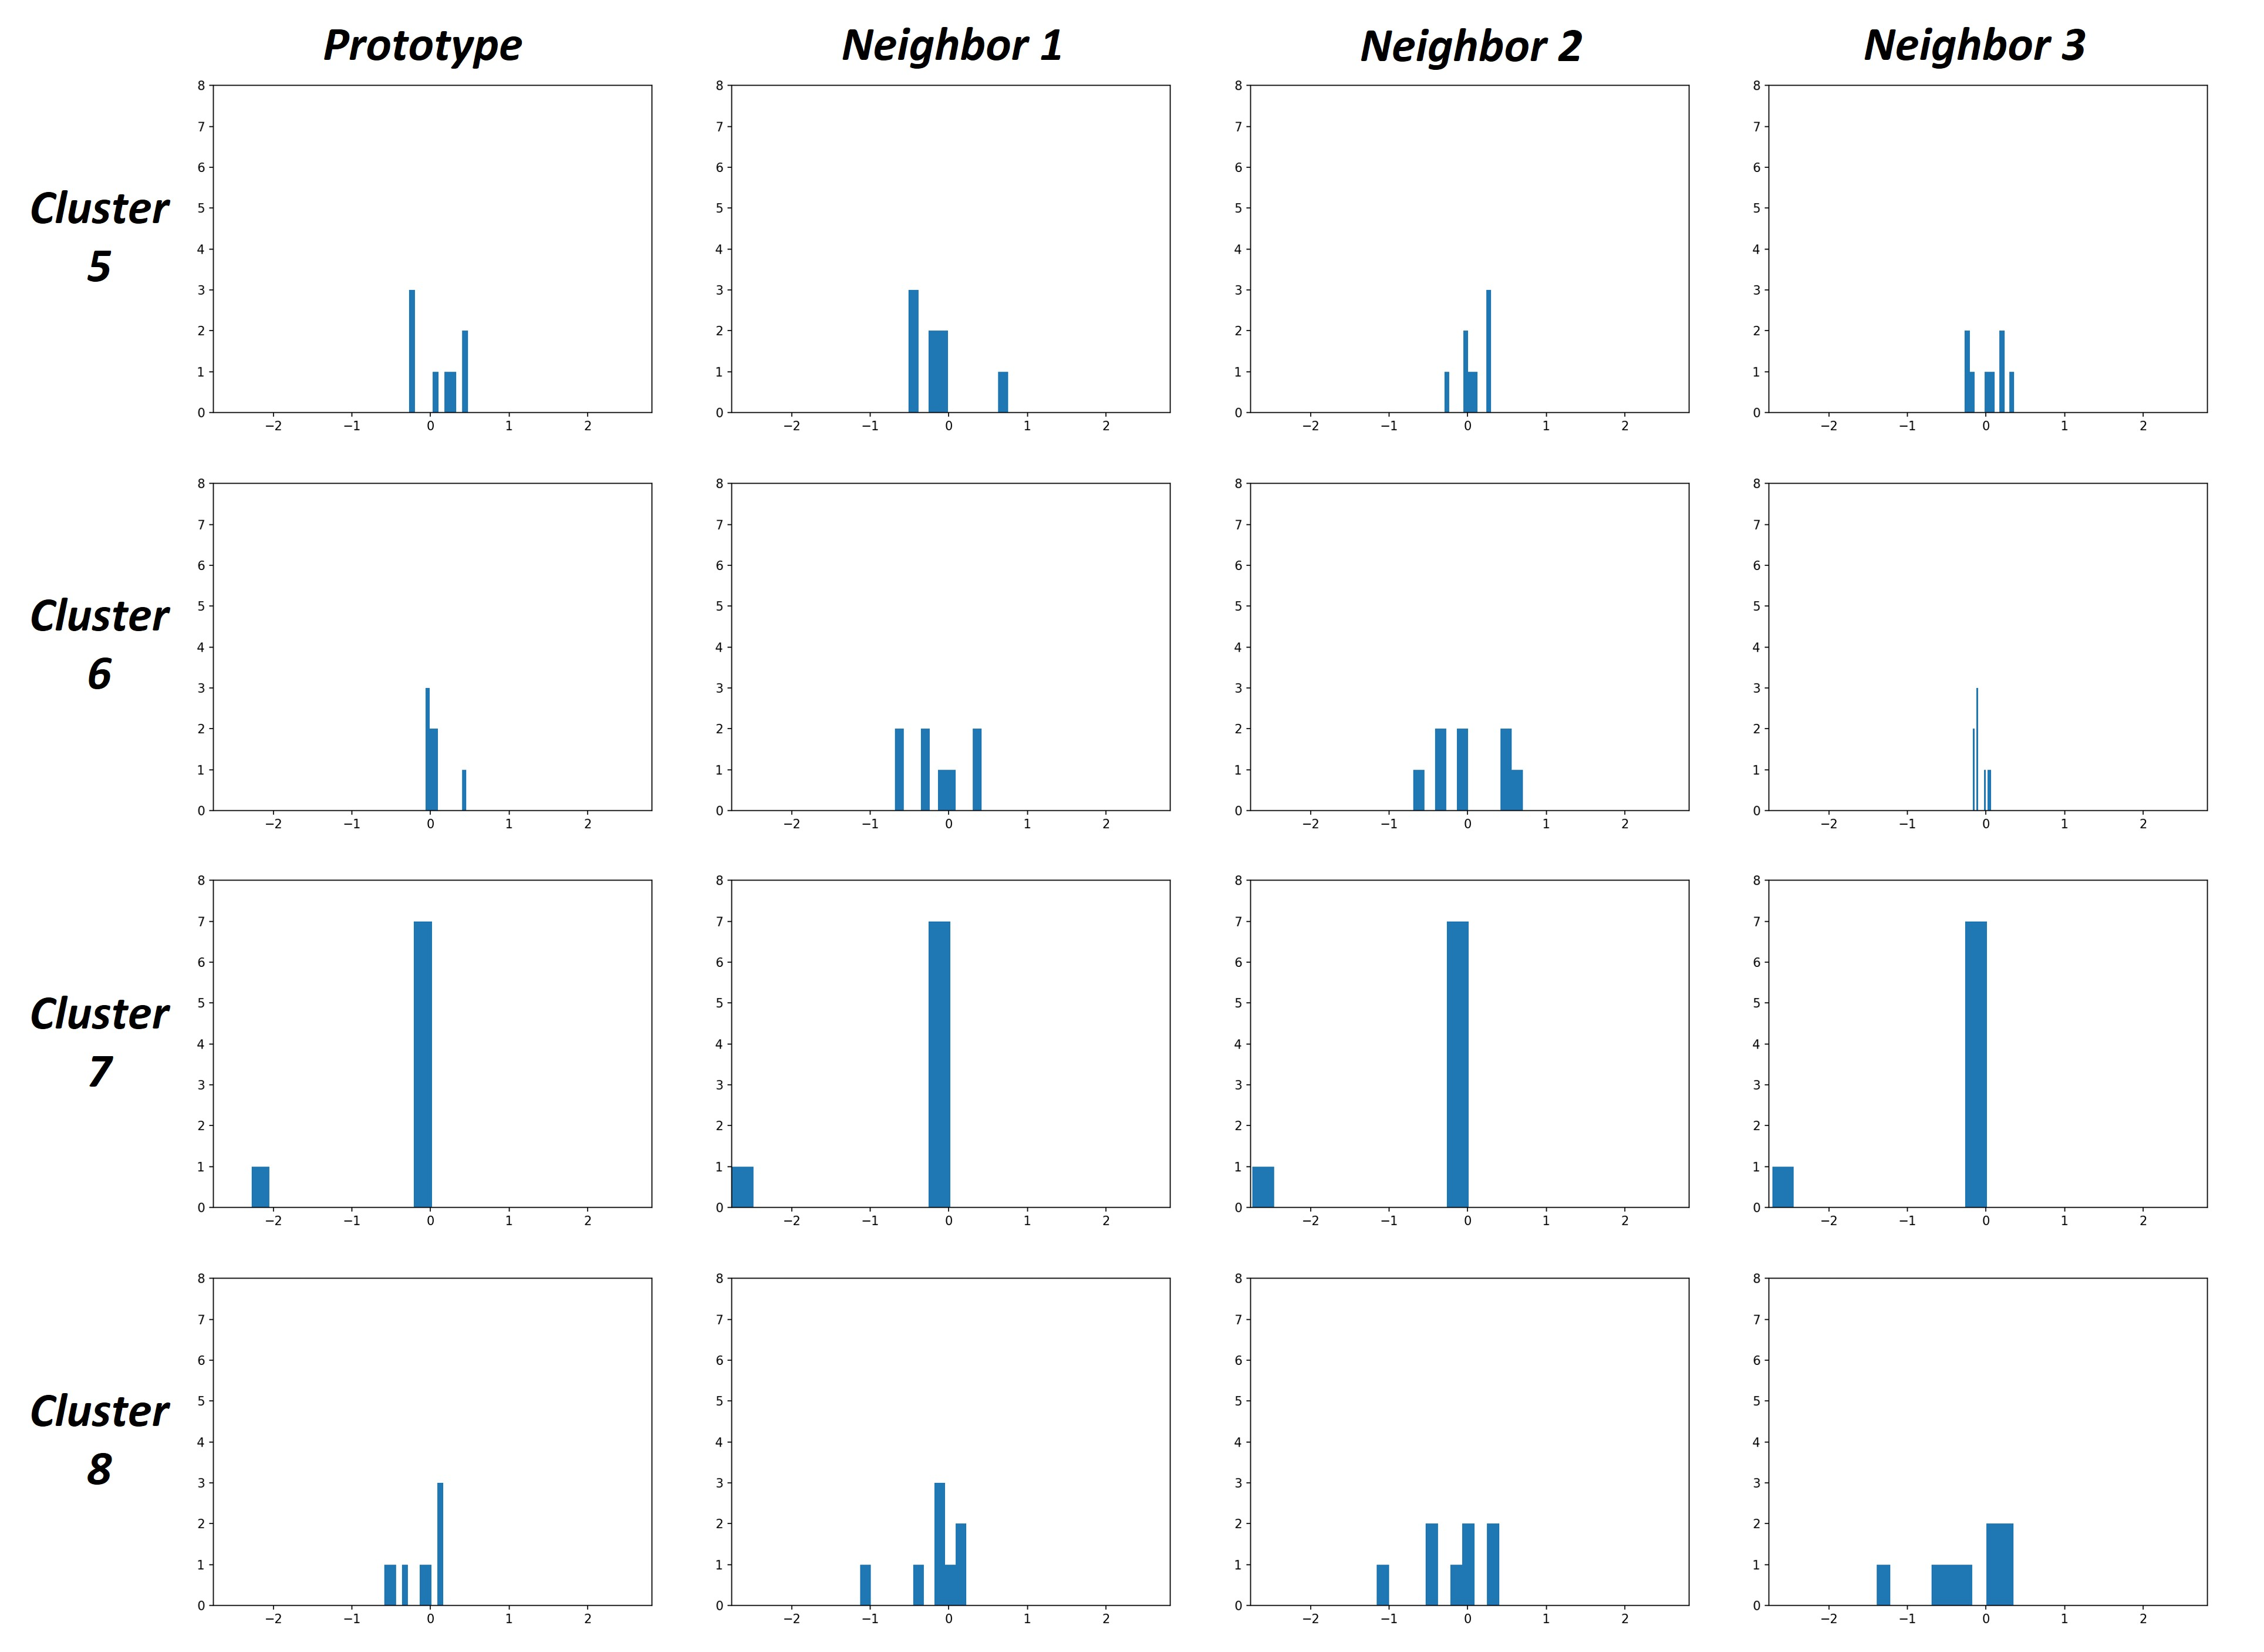}
\caption{The histogram of the eight centers (prototypes) and their neighbors in the \textbf{third band} of the flattened input. The band is in the \textbf{spectral domain} mapped by WHT, and the prototypes are assigned according to the \textbf{L1-norm distance}.}
\label{fig:slice3_l1}
\end{figure*}

%%%% L2 spectral
% slice 1
\begin{figure*}[h]
\centering
\includegraphics[scale=0.48]{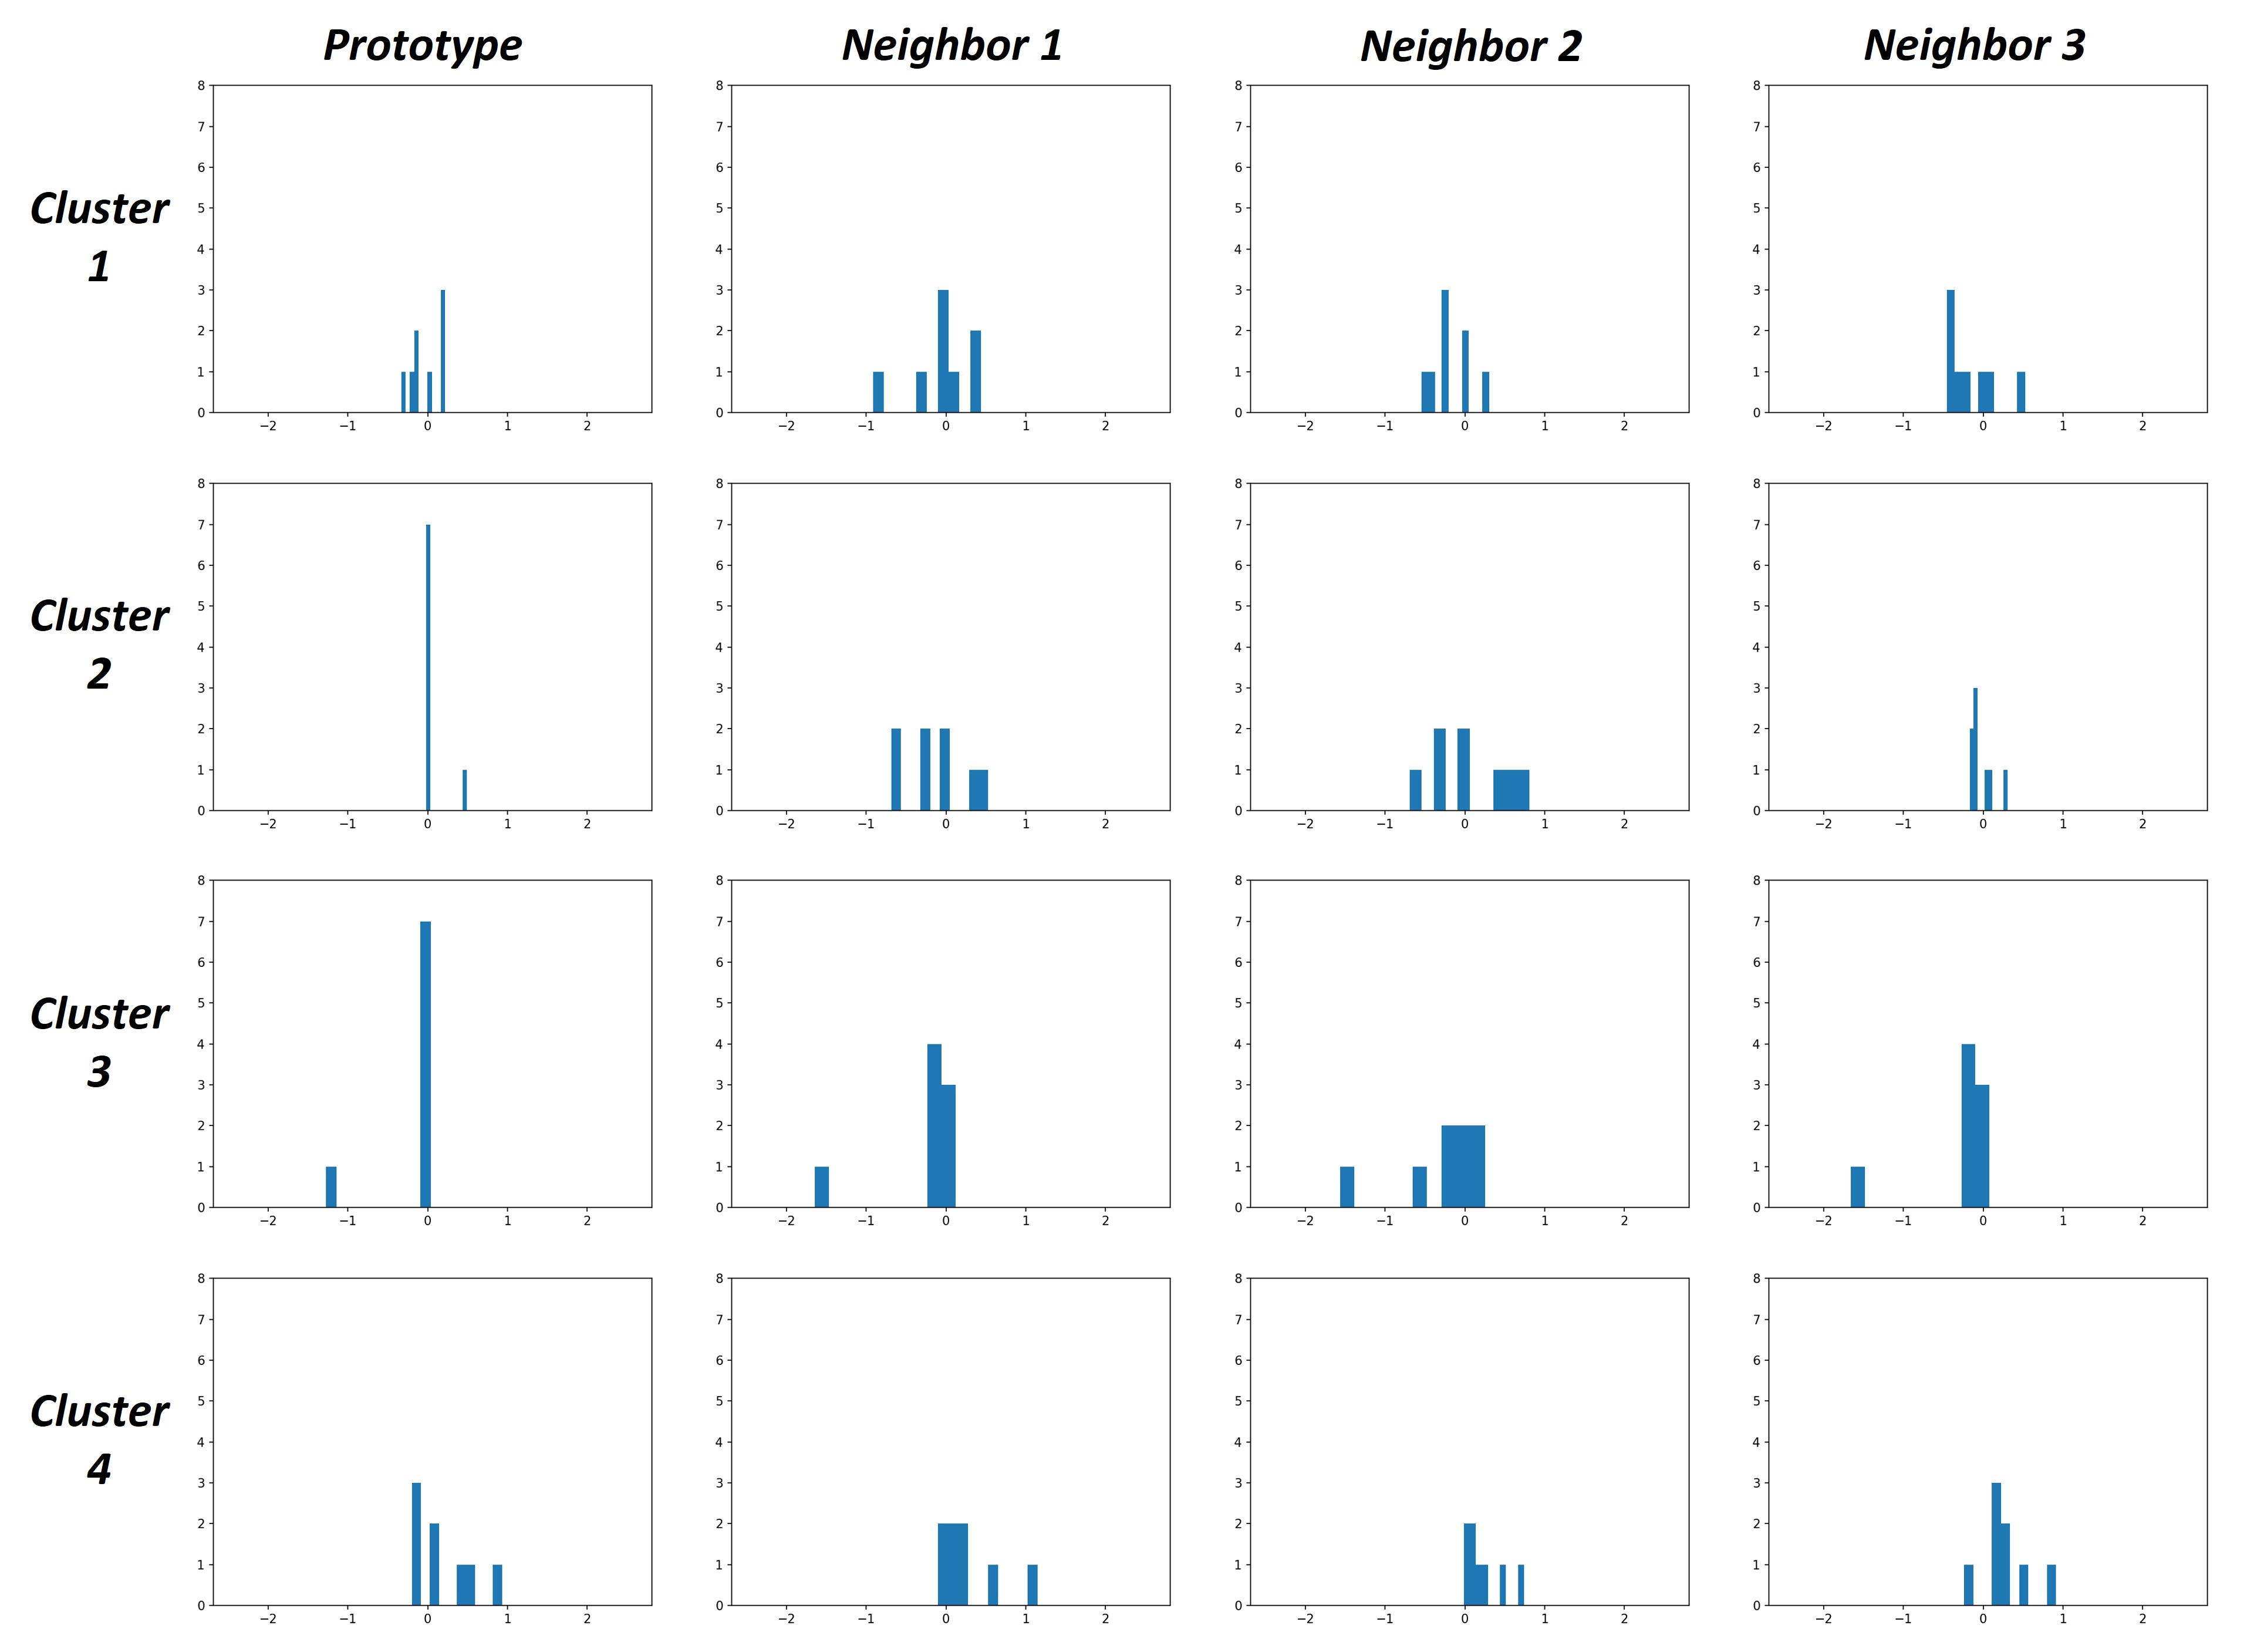}
\centering
\includegraphics[scale=0.48]{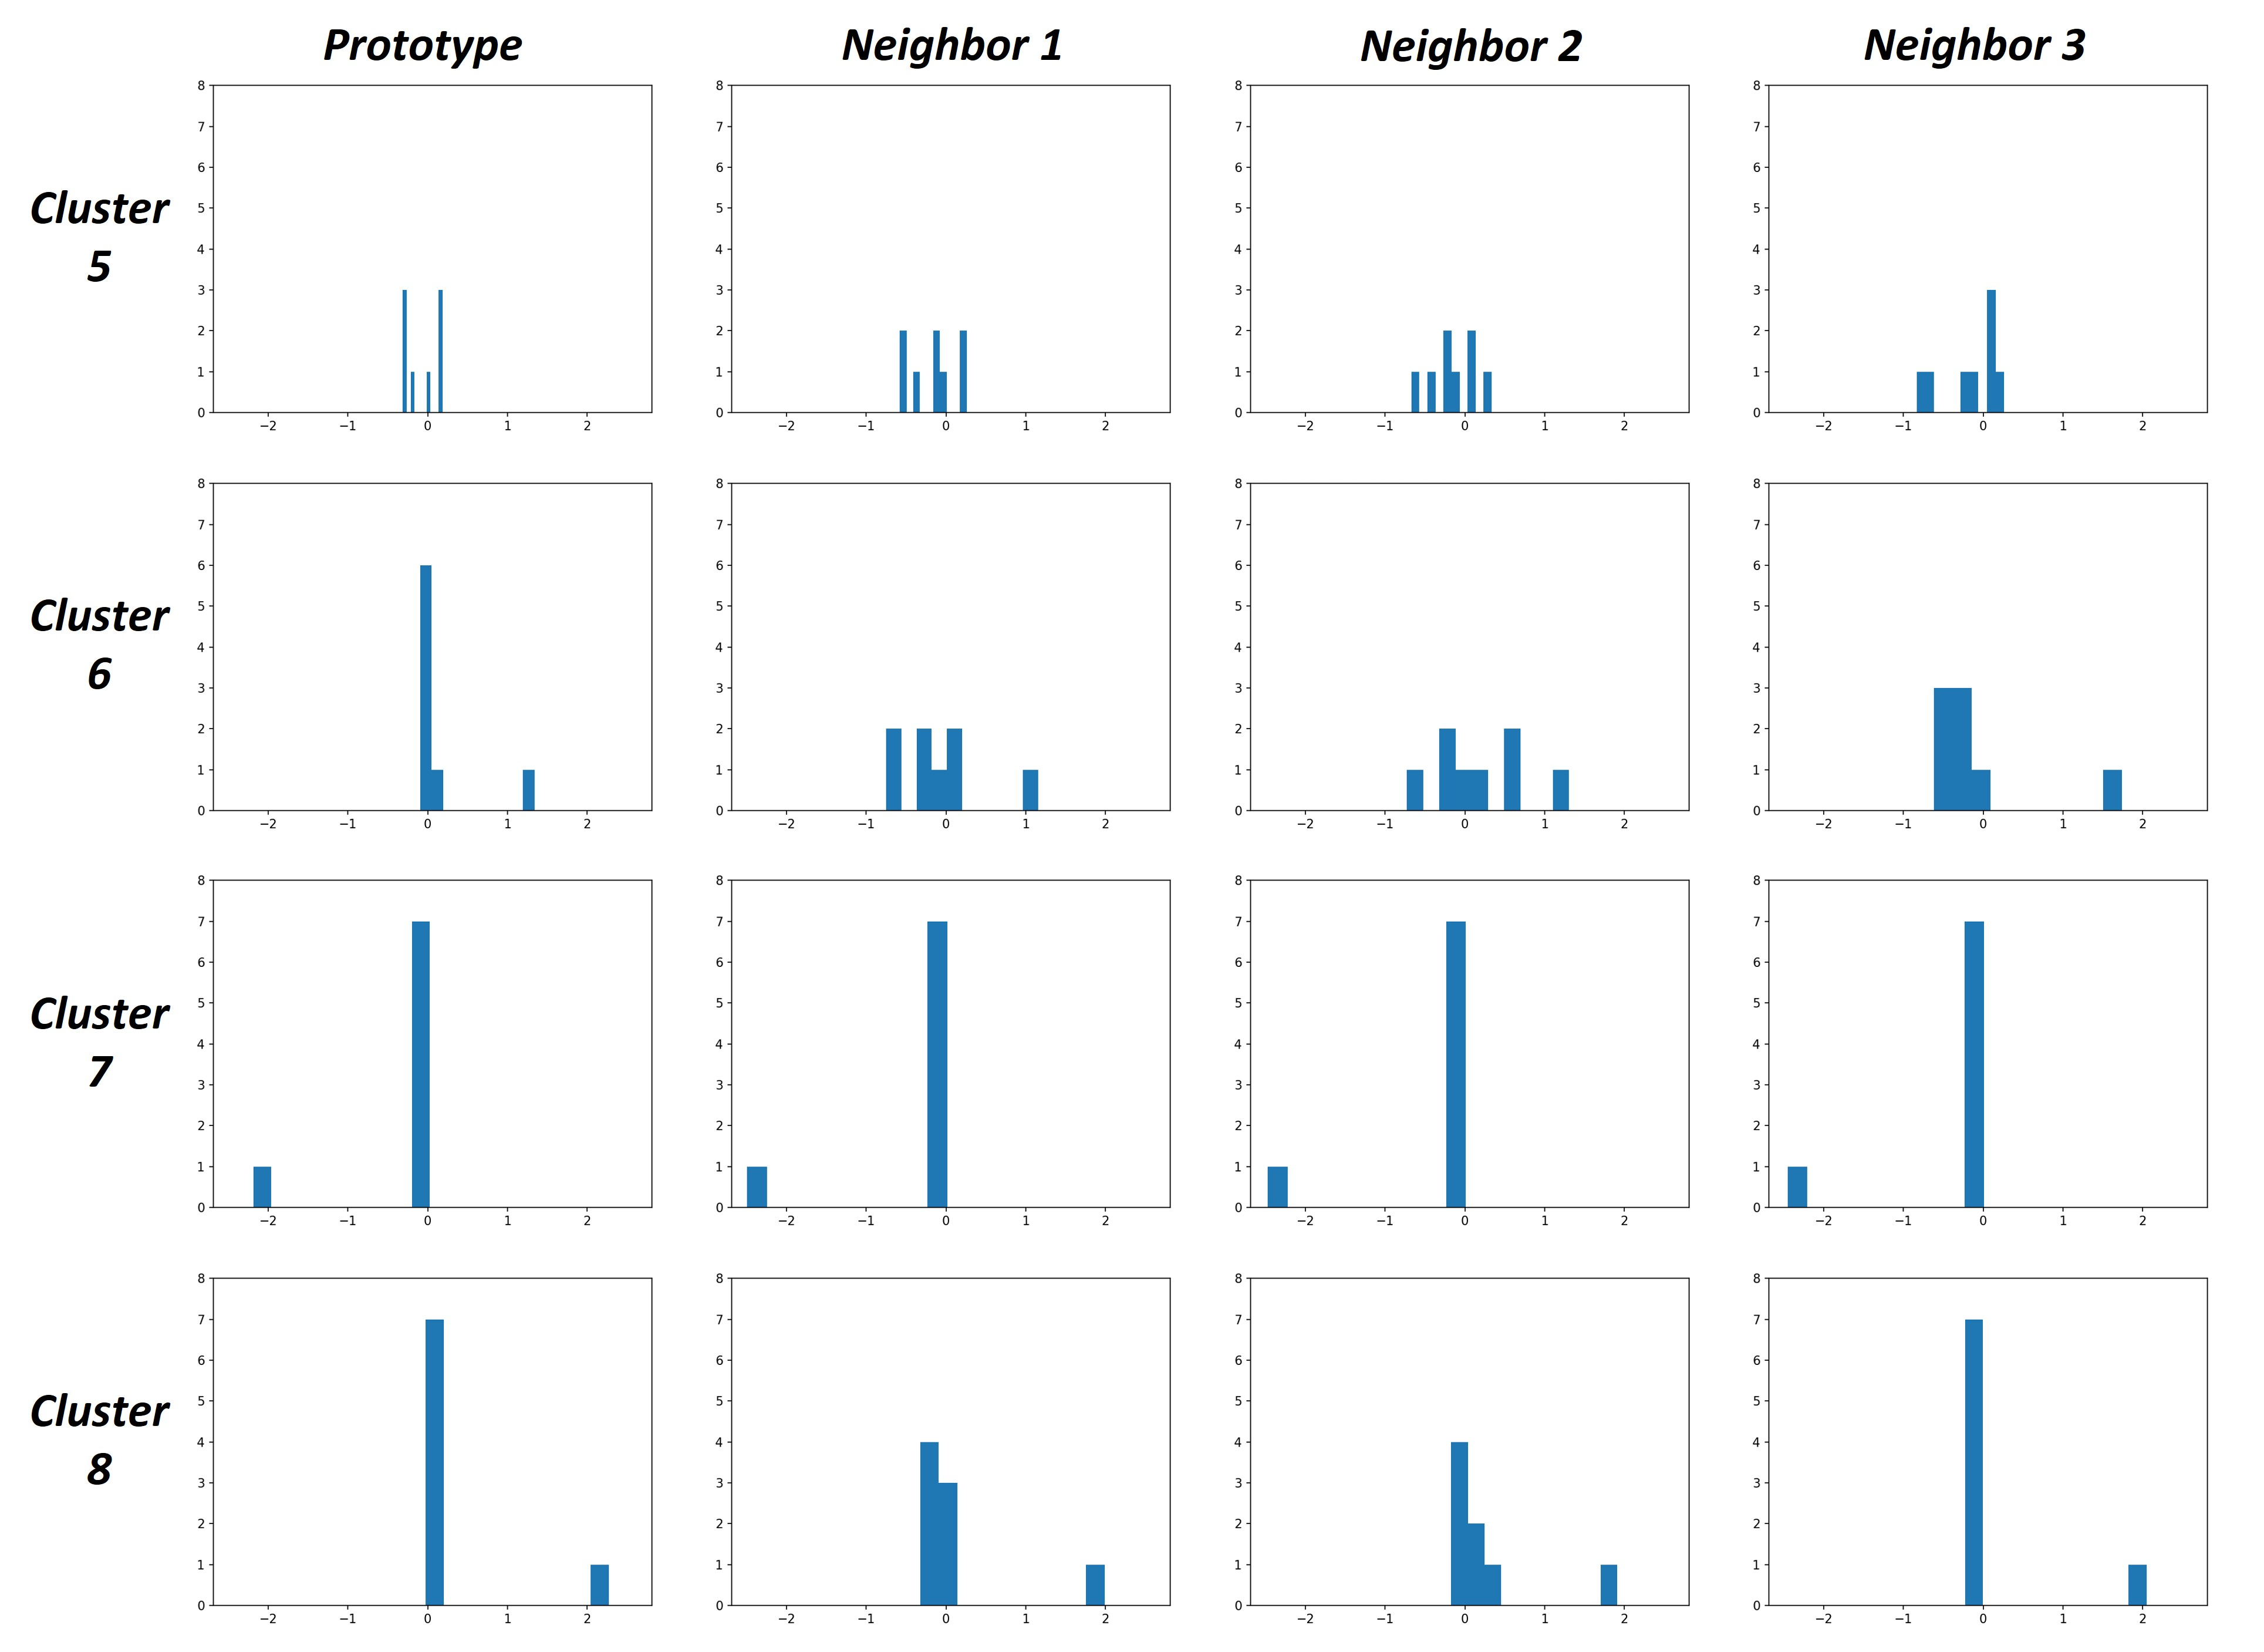}
\caption{The histogram of the eight centers (prototypes) and their neighbors in the \textbf{first band} of the flattened input. The band is in the \textbf{spectral domain} mapped by WHT, and the prototypes are assigned according to the \textbf{L2-norm distance}.}
\label{fig:slice1_l2_spectral}
\end{figure*}

% slice 2
\begin{figure*}[h]
\centering
\includegraphics[scale=0.48]{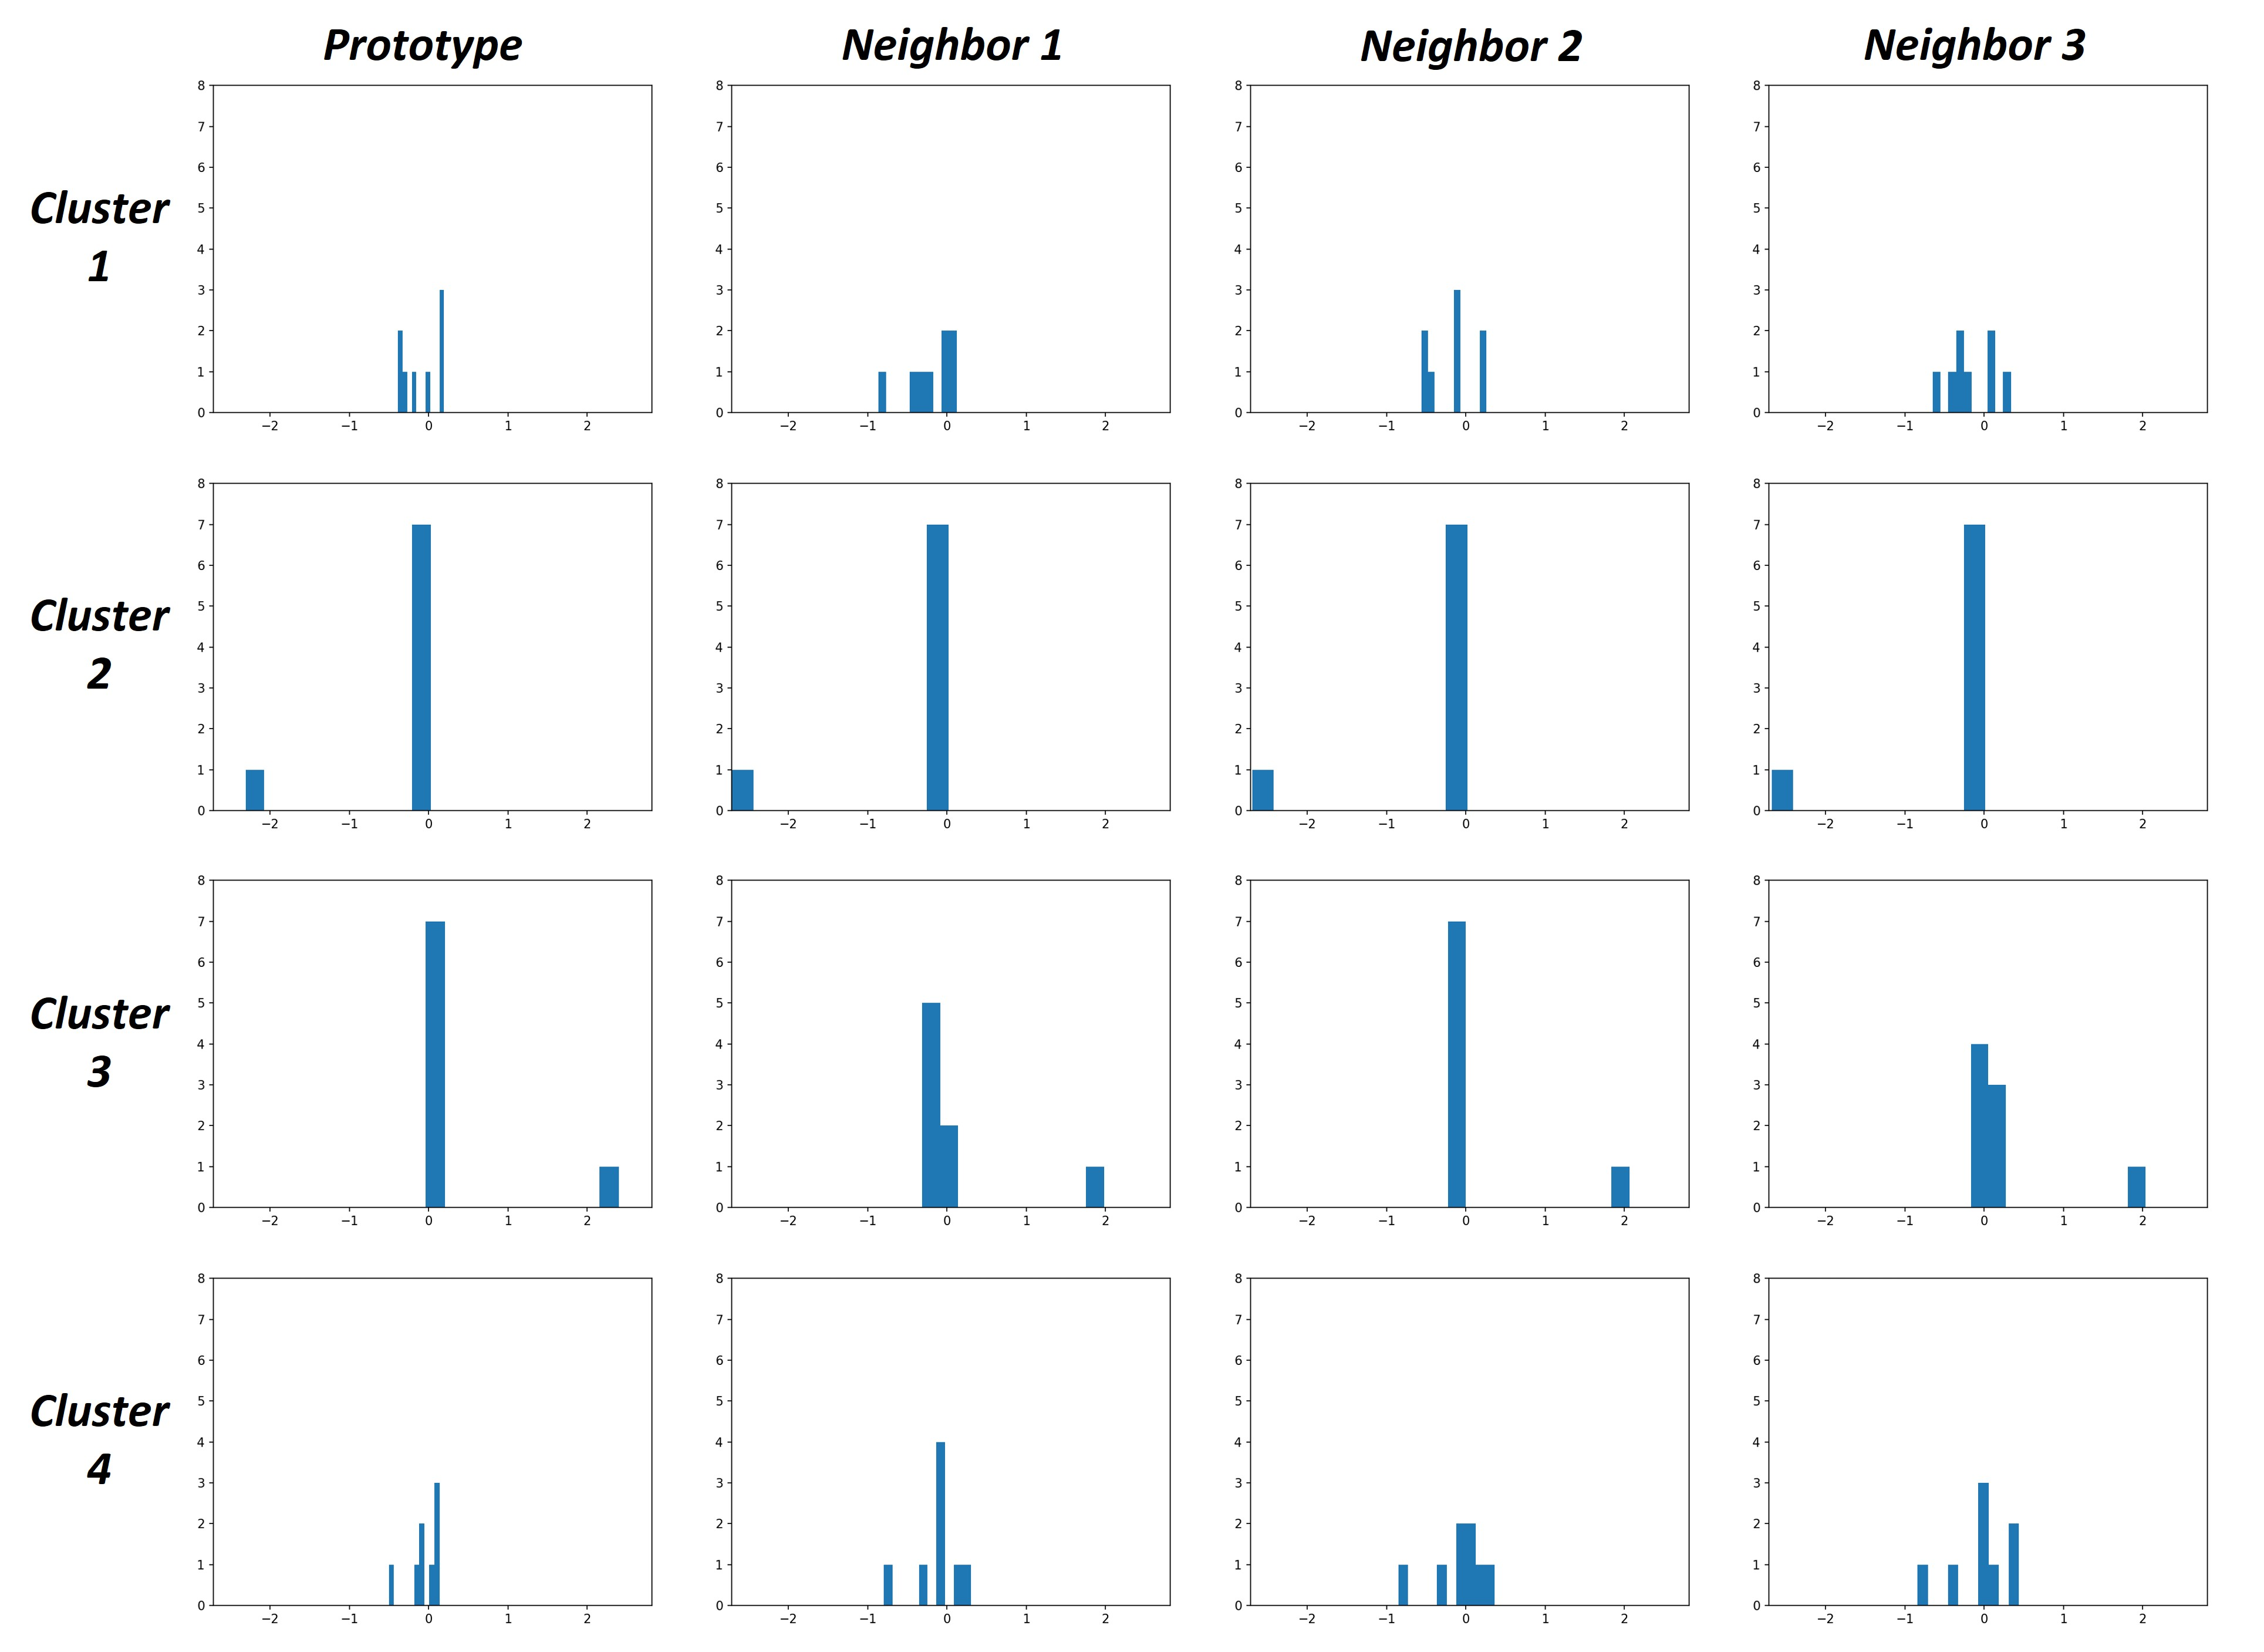}
\centering
\includegraphics[scale=0.48]{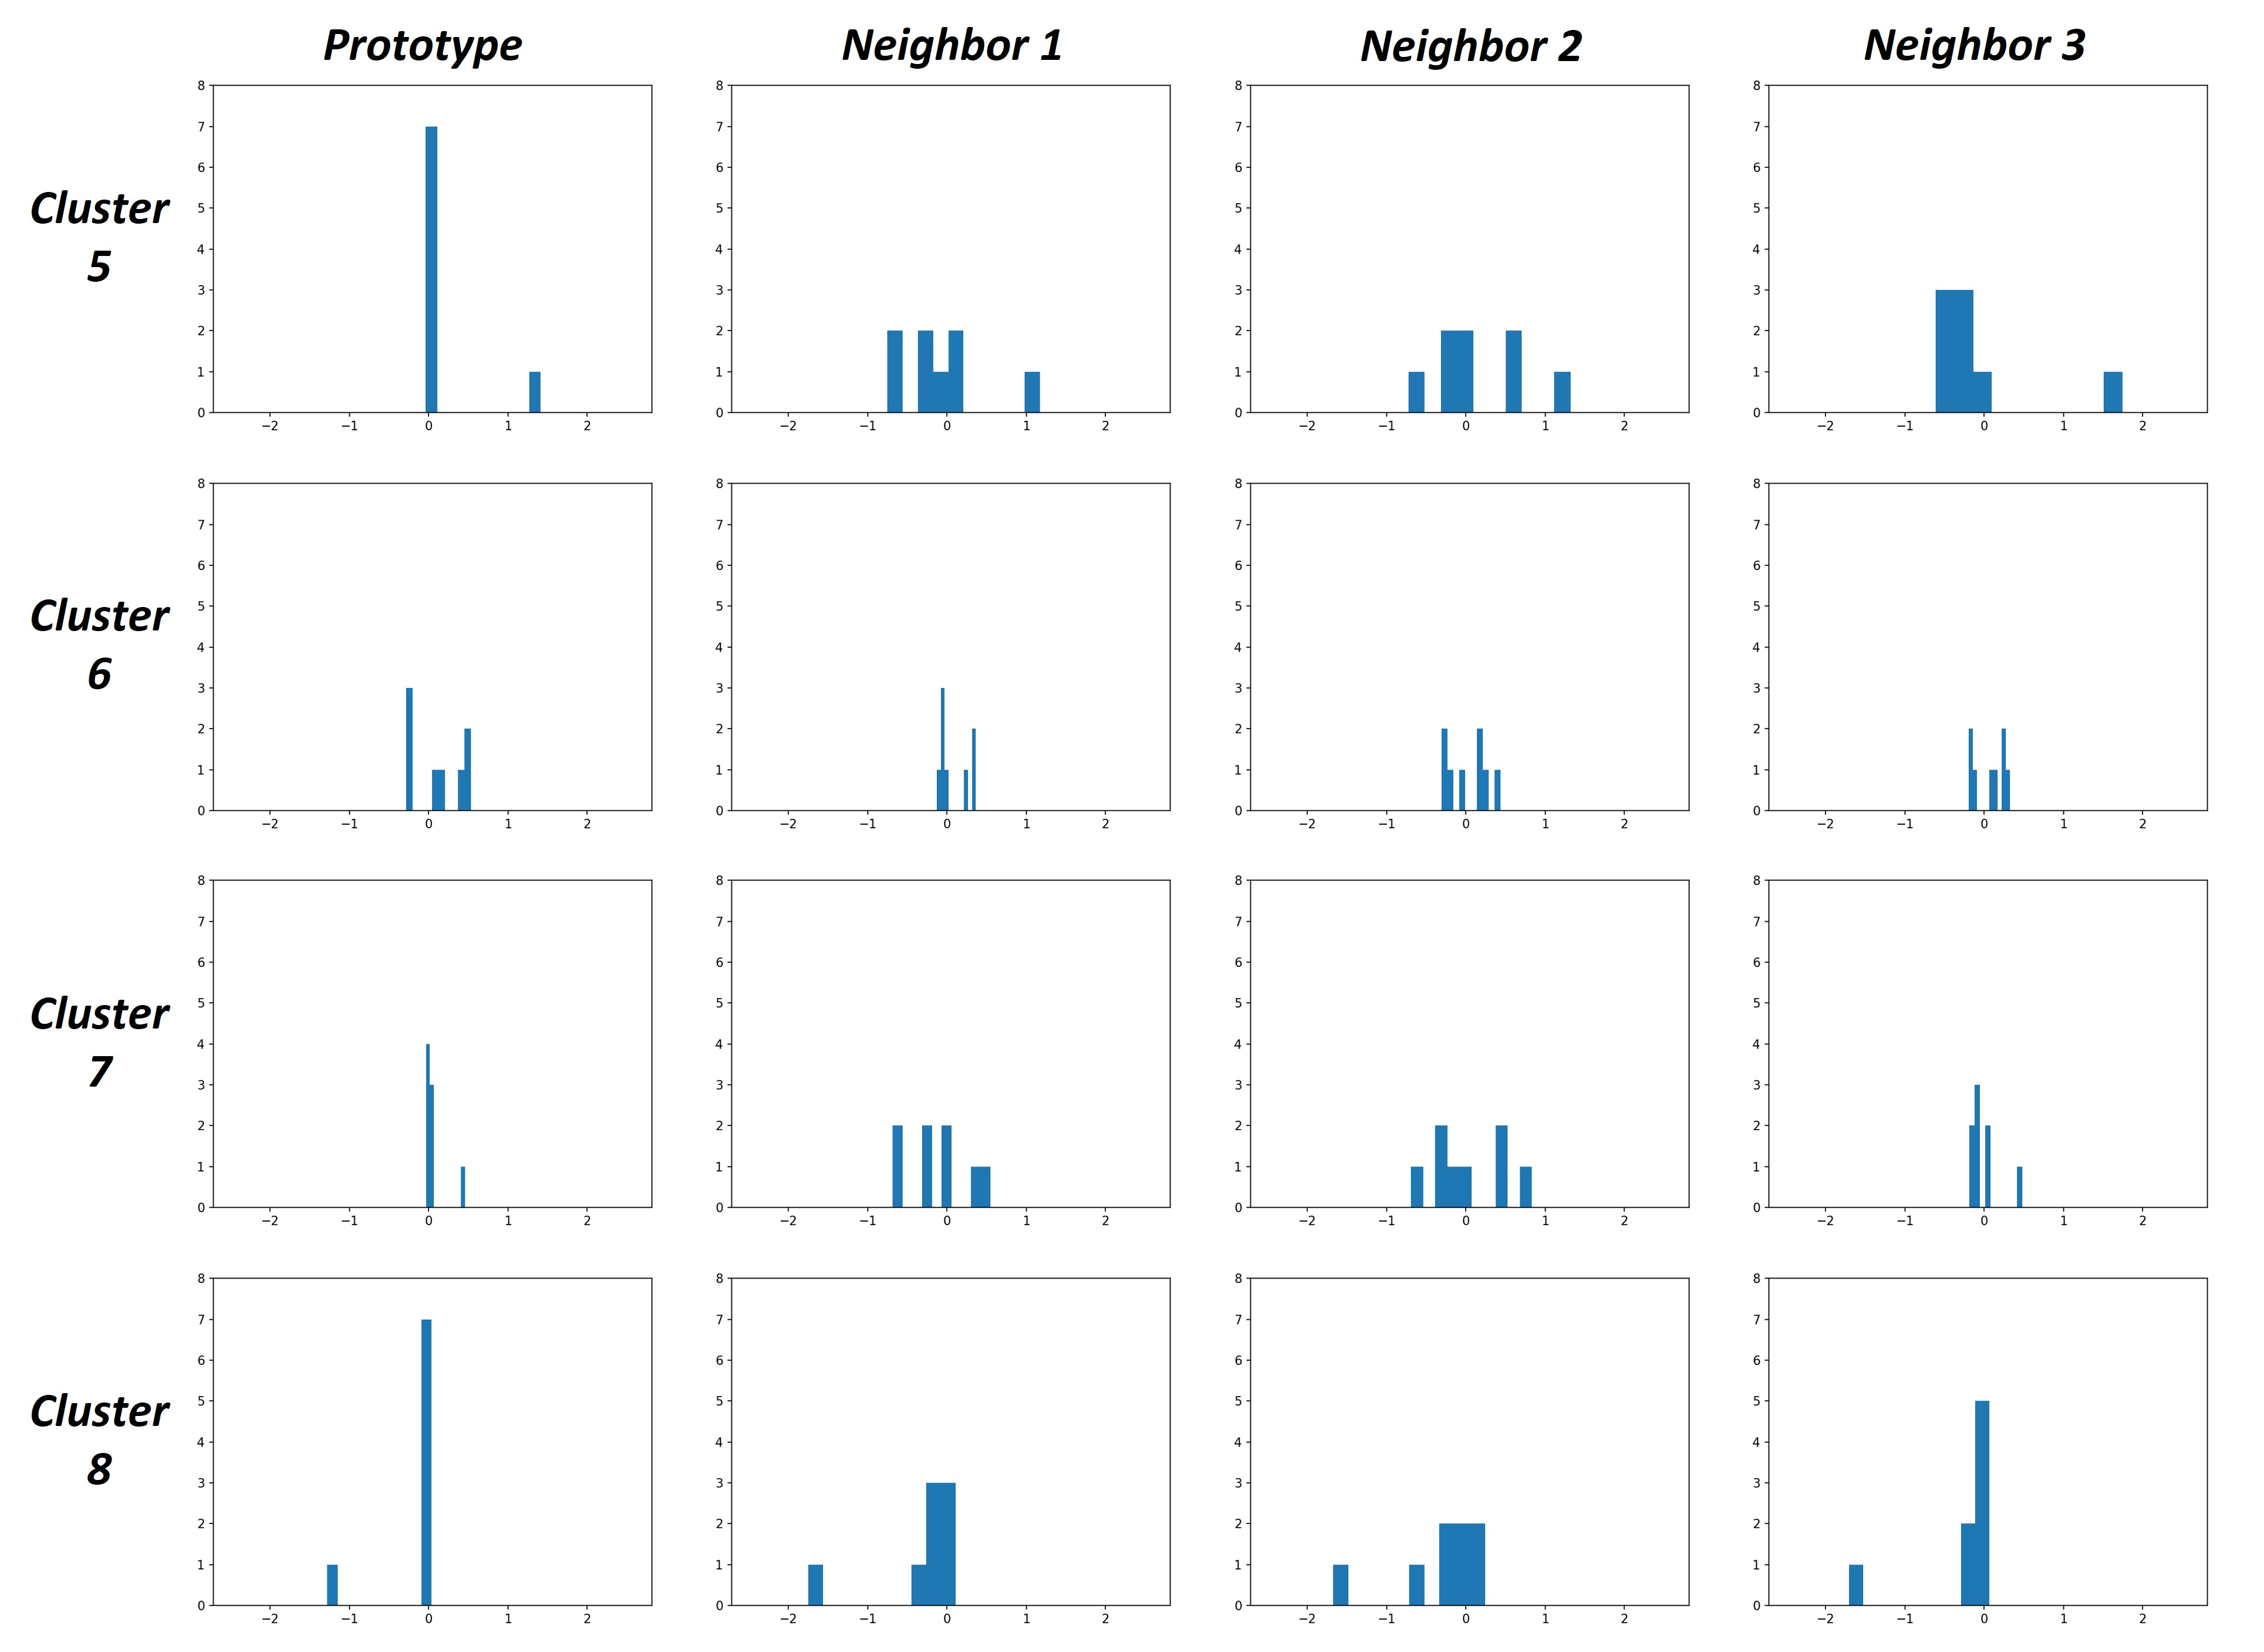}
\caption{The histogram of the eight centers (prototypes) and their neighbors in the \textbf{second band} of the flattened input. The band is in the \textbf{spectral domain} mapped by WHT, and the prototypes are assigned according to the \textbf{L2-norm distance}.}
\label{fig:slice2_l2_spectral}
\end{figure*}

% slice 3
\begin{figure*}[h]
\centering
\includegraphics[scale=0.48]{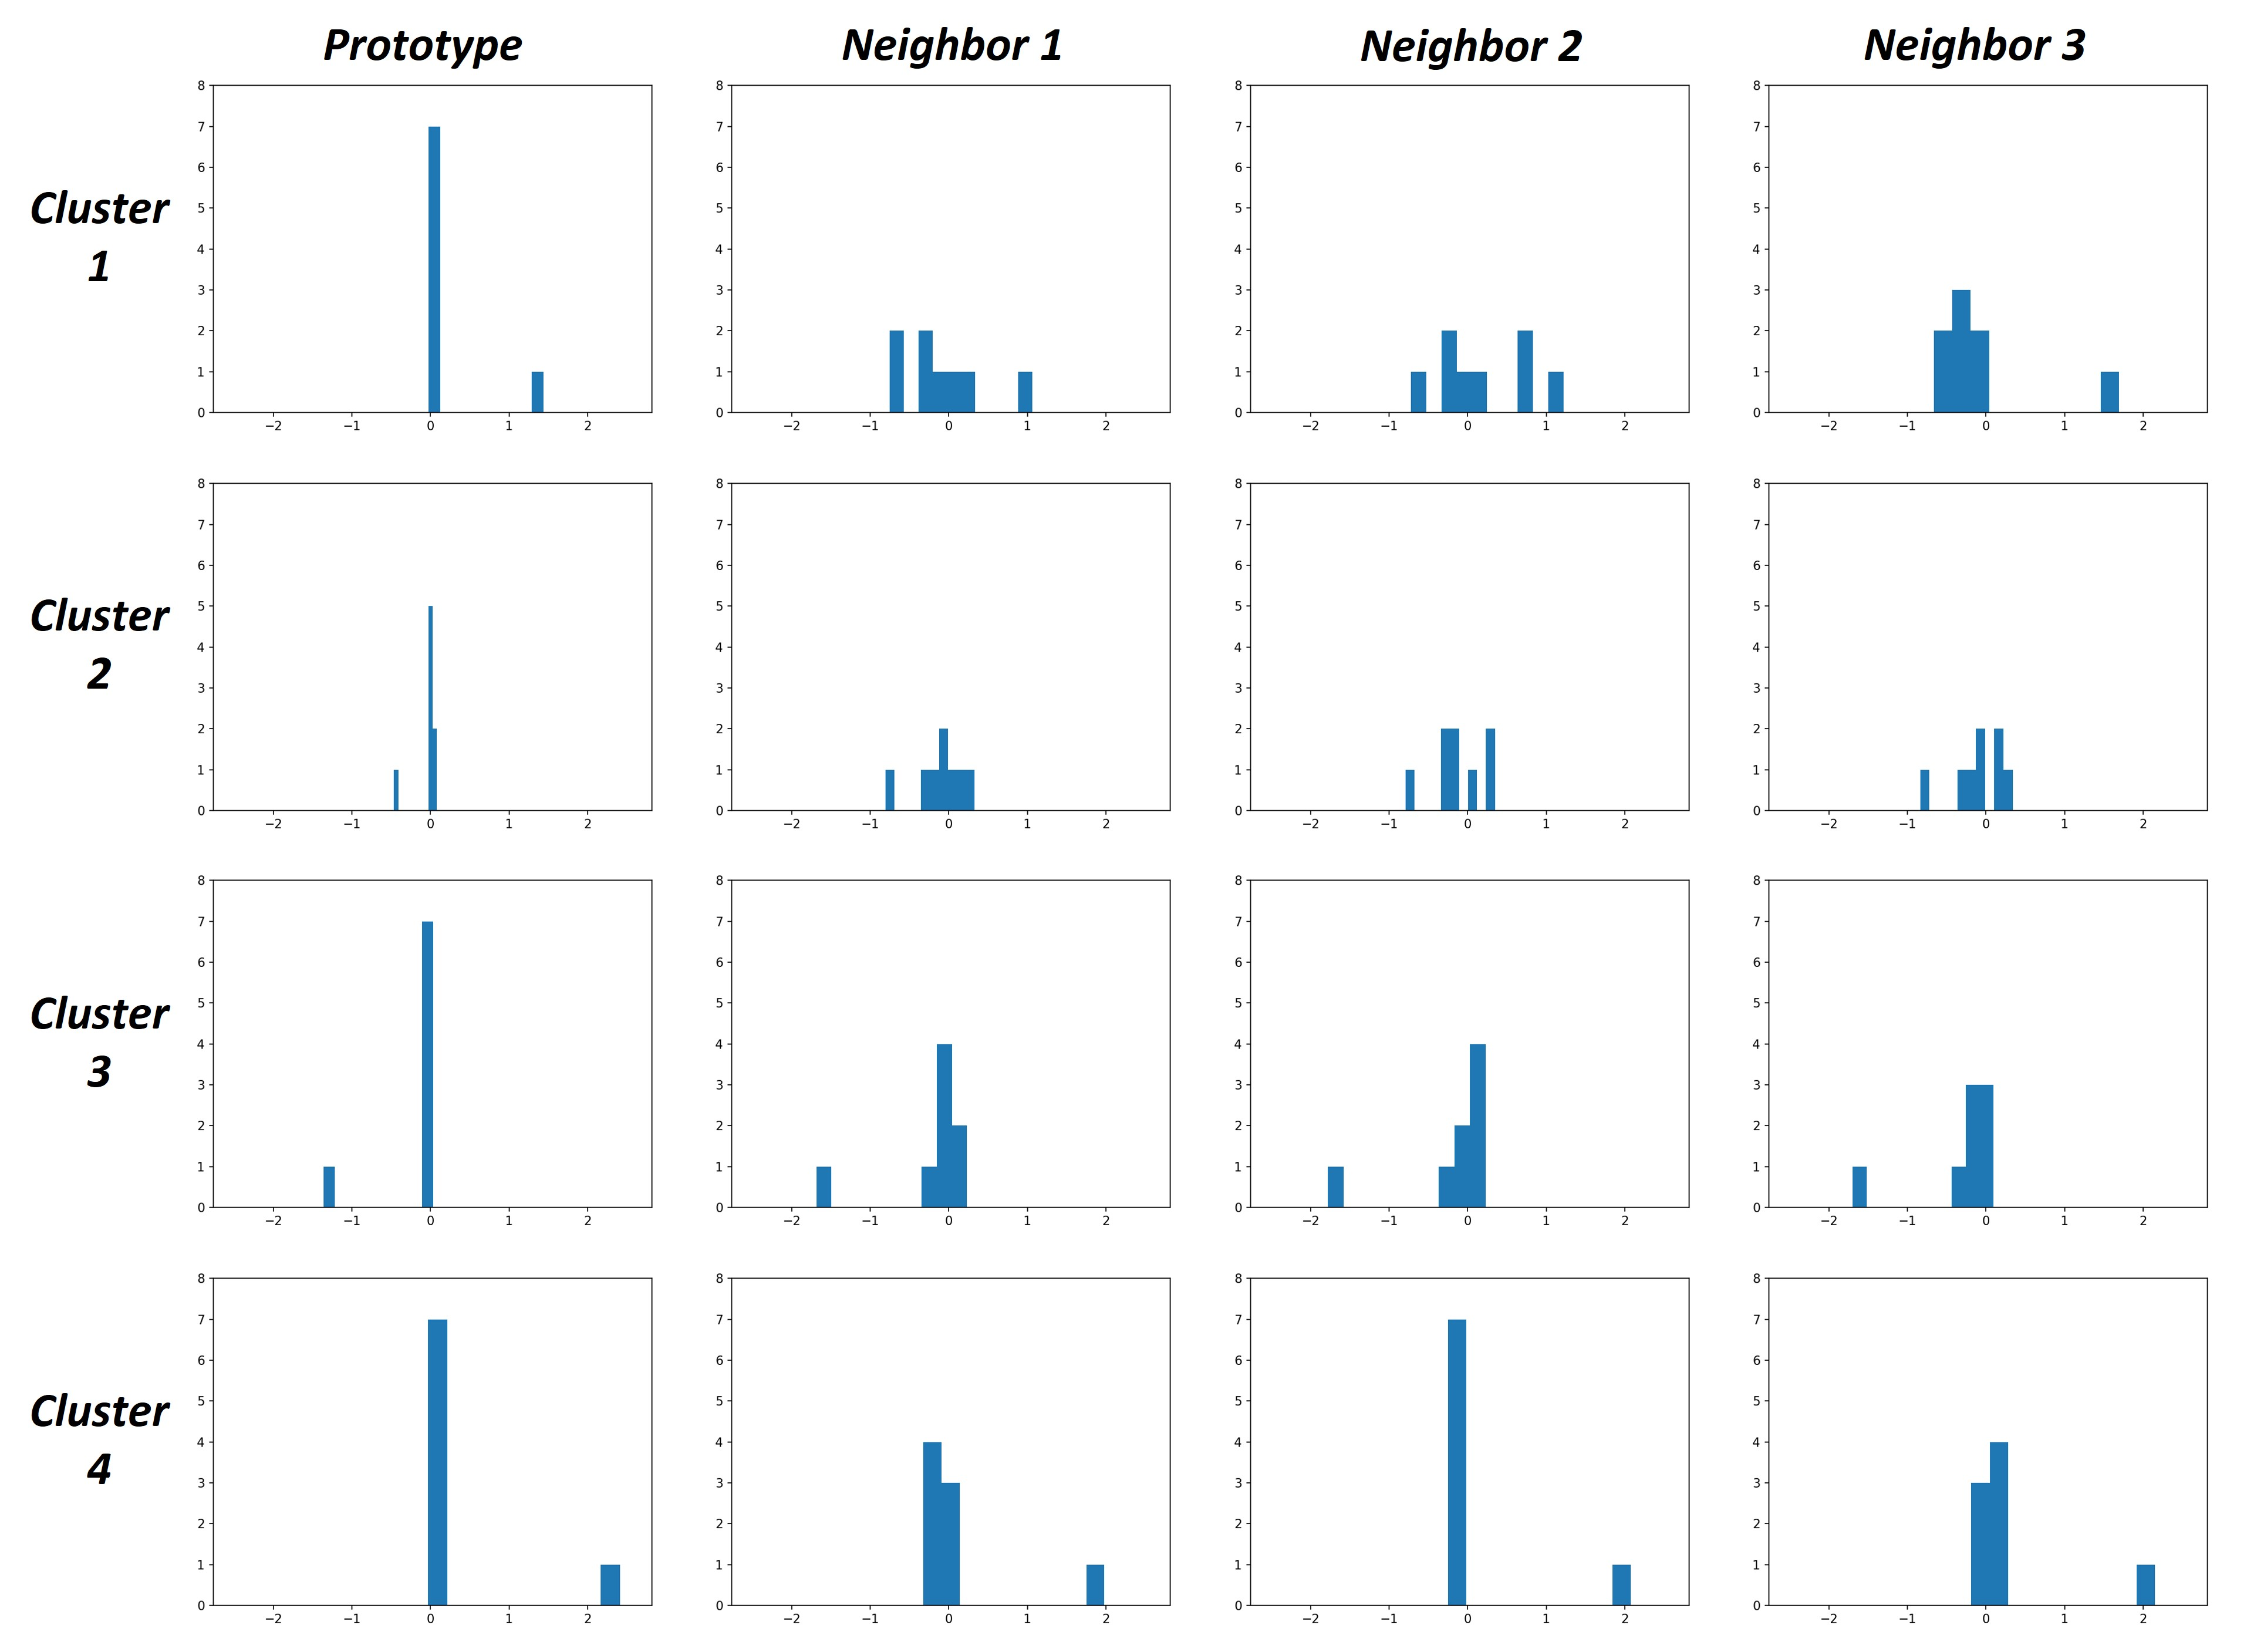}
\centering
\includegraphics[scale=0.48]{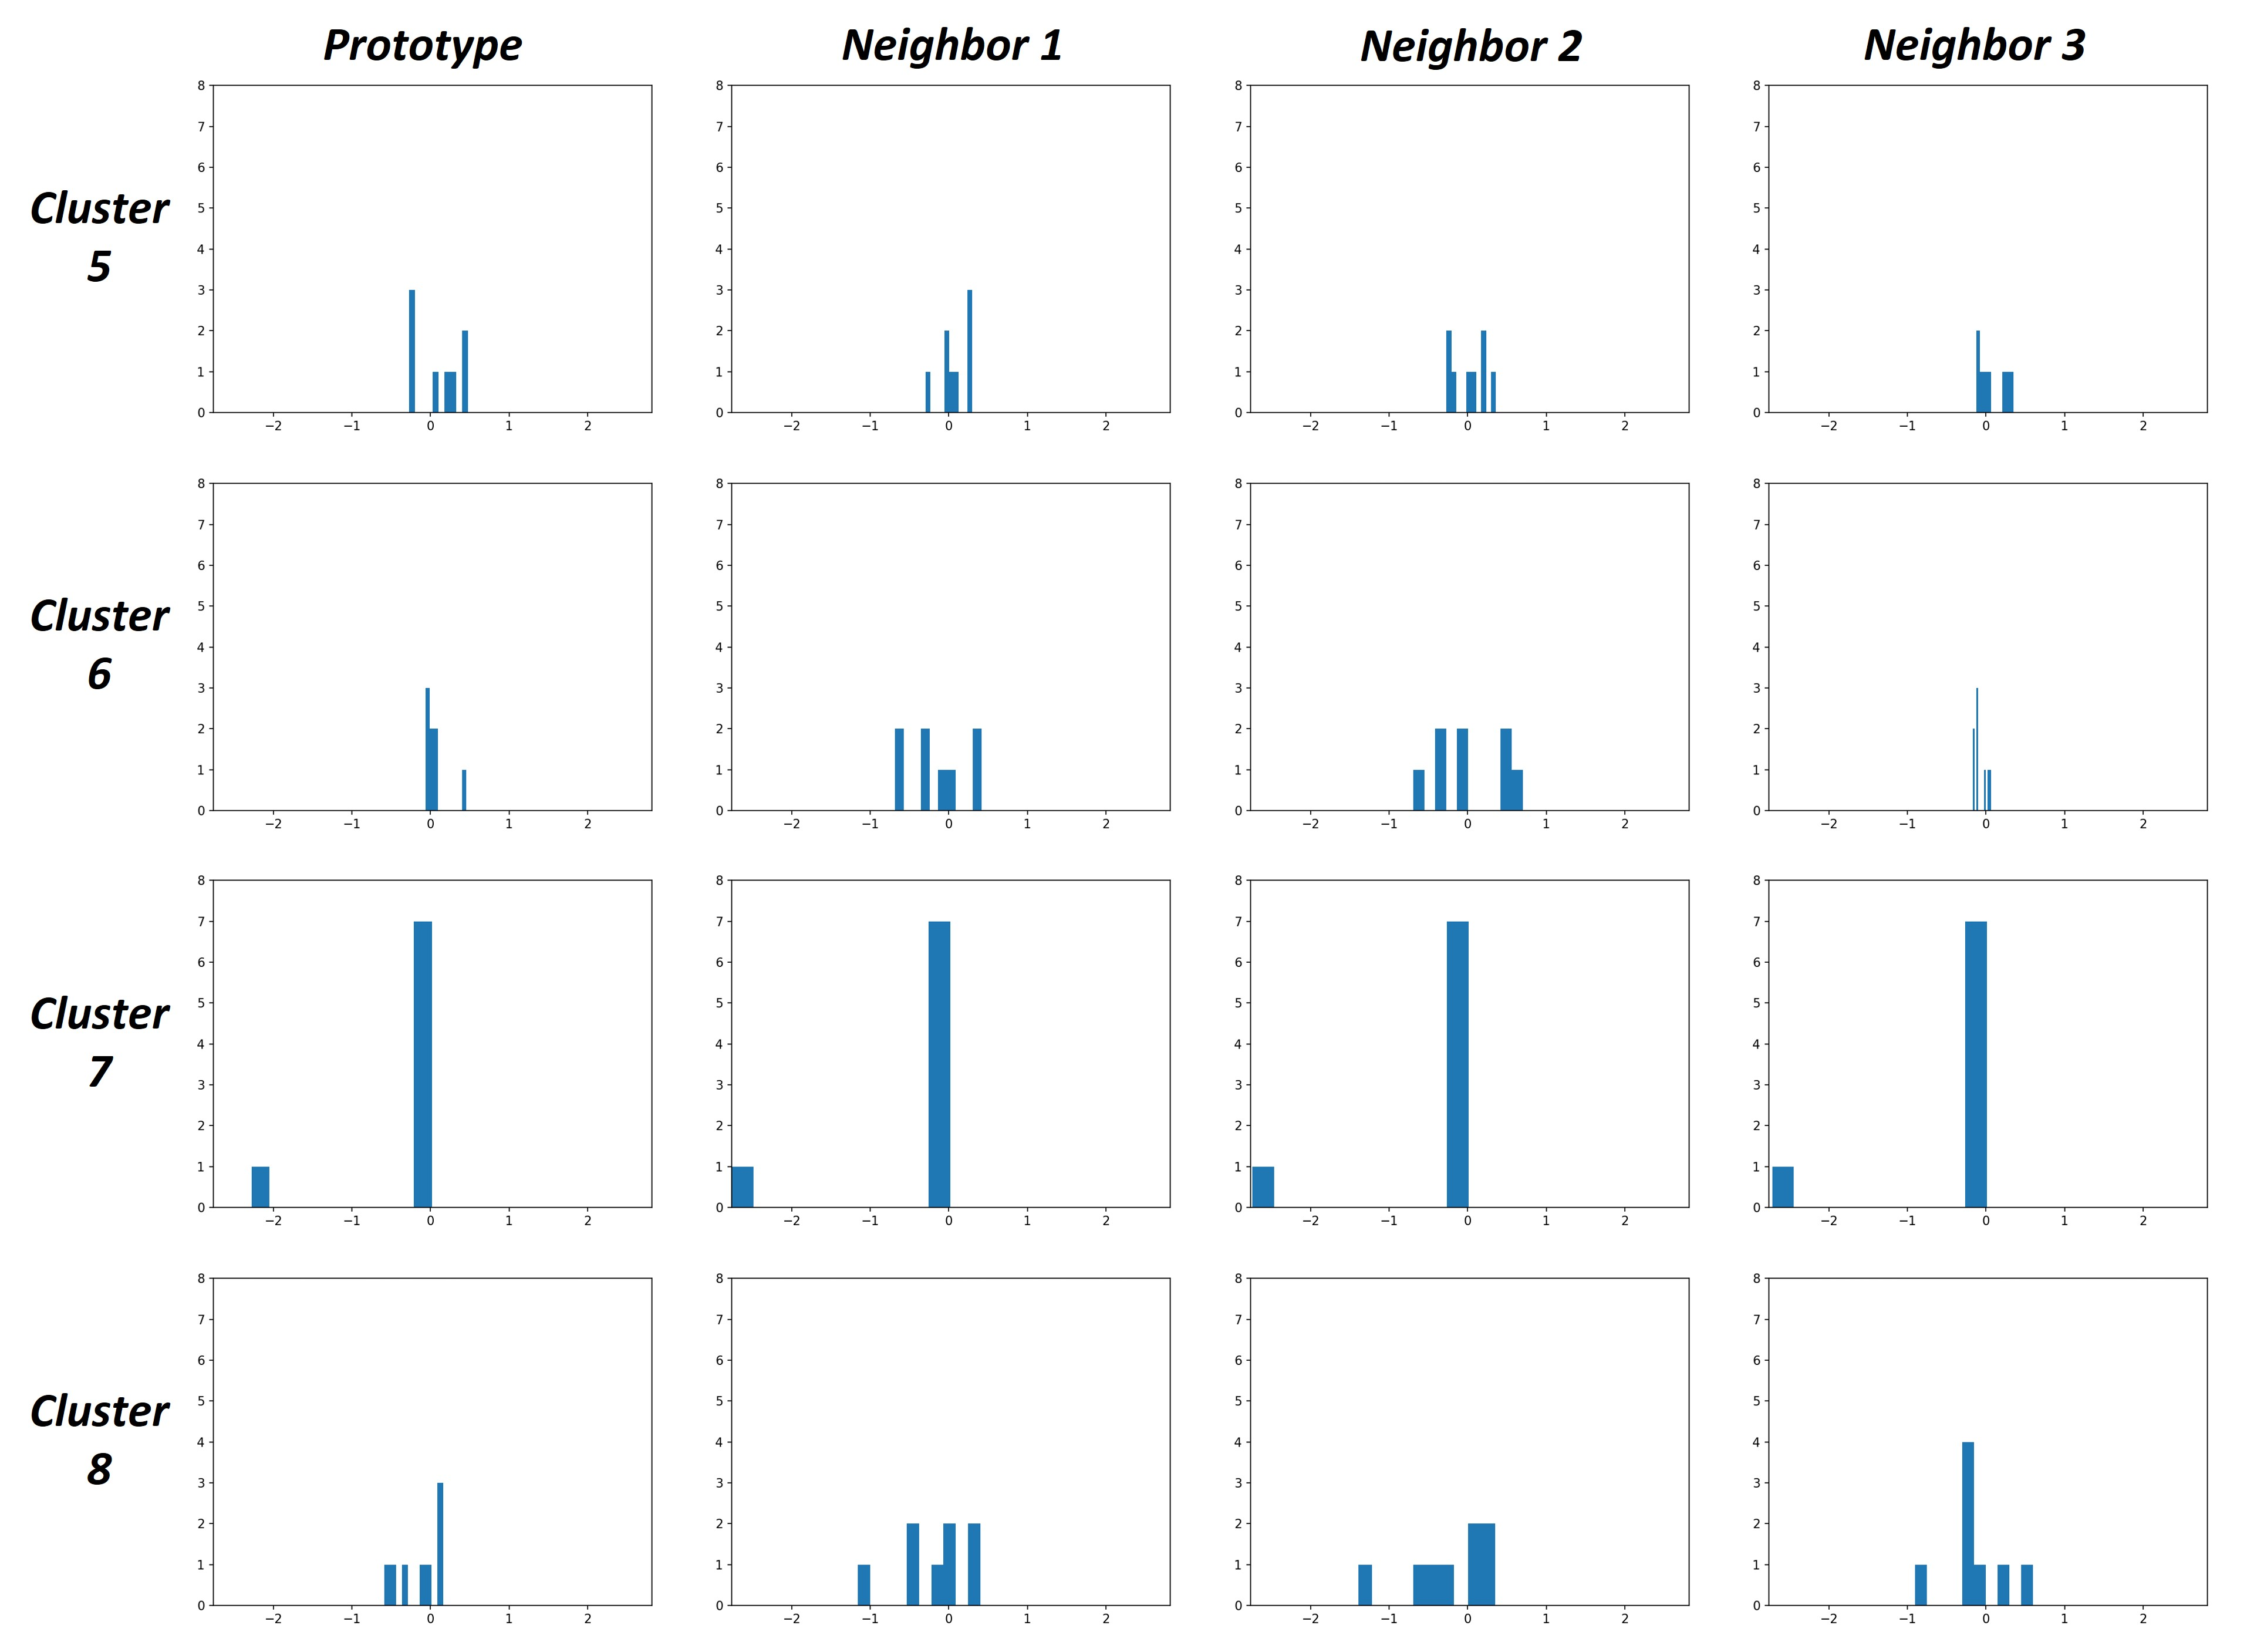}
\caption{The histogram of the eight centers (prototypes) and their neighbors in the \textbf{third band} of the flattened input. The band is in the \textbf{spectral domain} mapped by WHT, and the prototypes are assigned according to the \textbf{L2-norm distance}.}
\label{fig:slice3_l2_spectral}
\end{figure*}

%%%% L2 spatial
% slice 1
\begin{figure*}[h]
\centering
\includegraphics[scale=0.48]{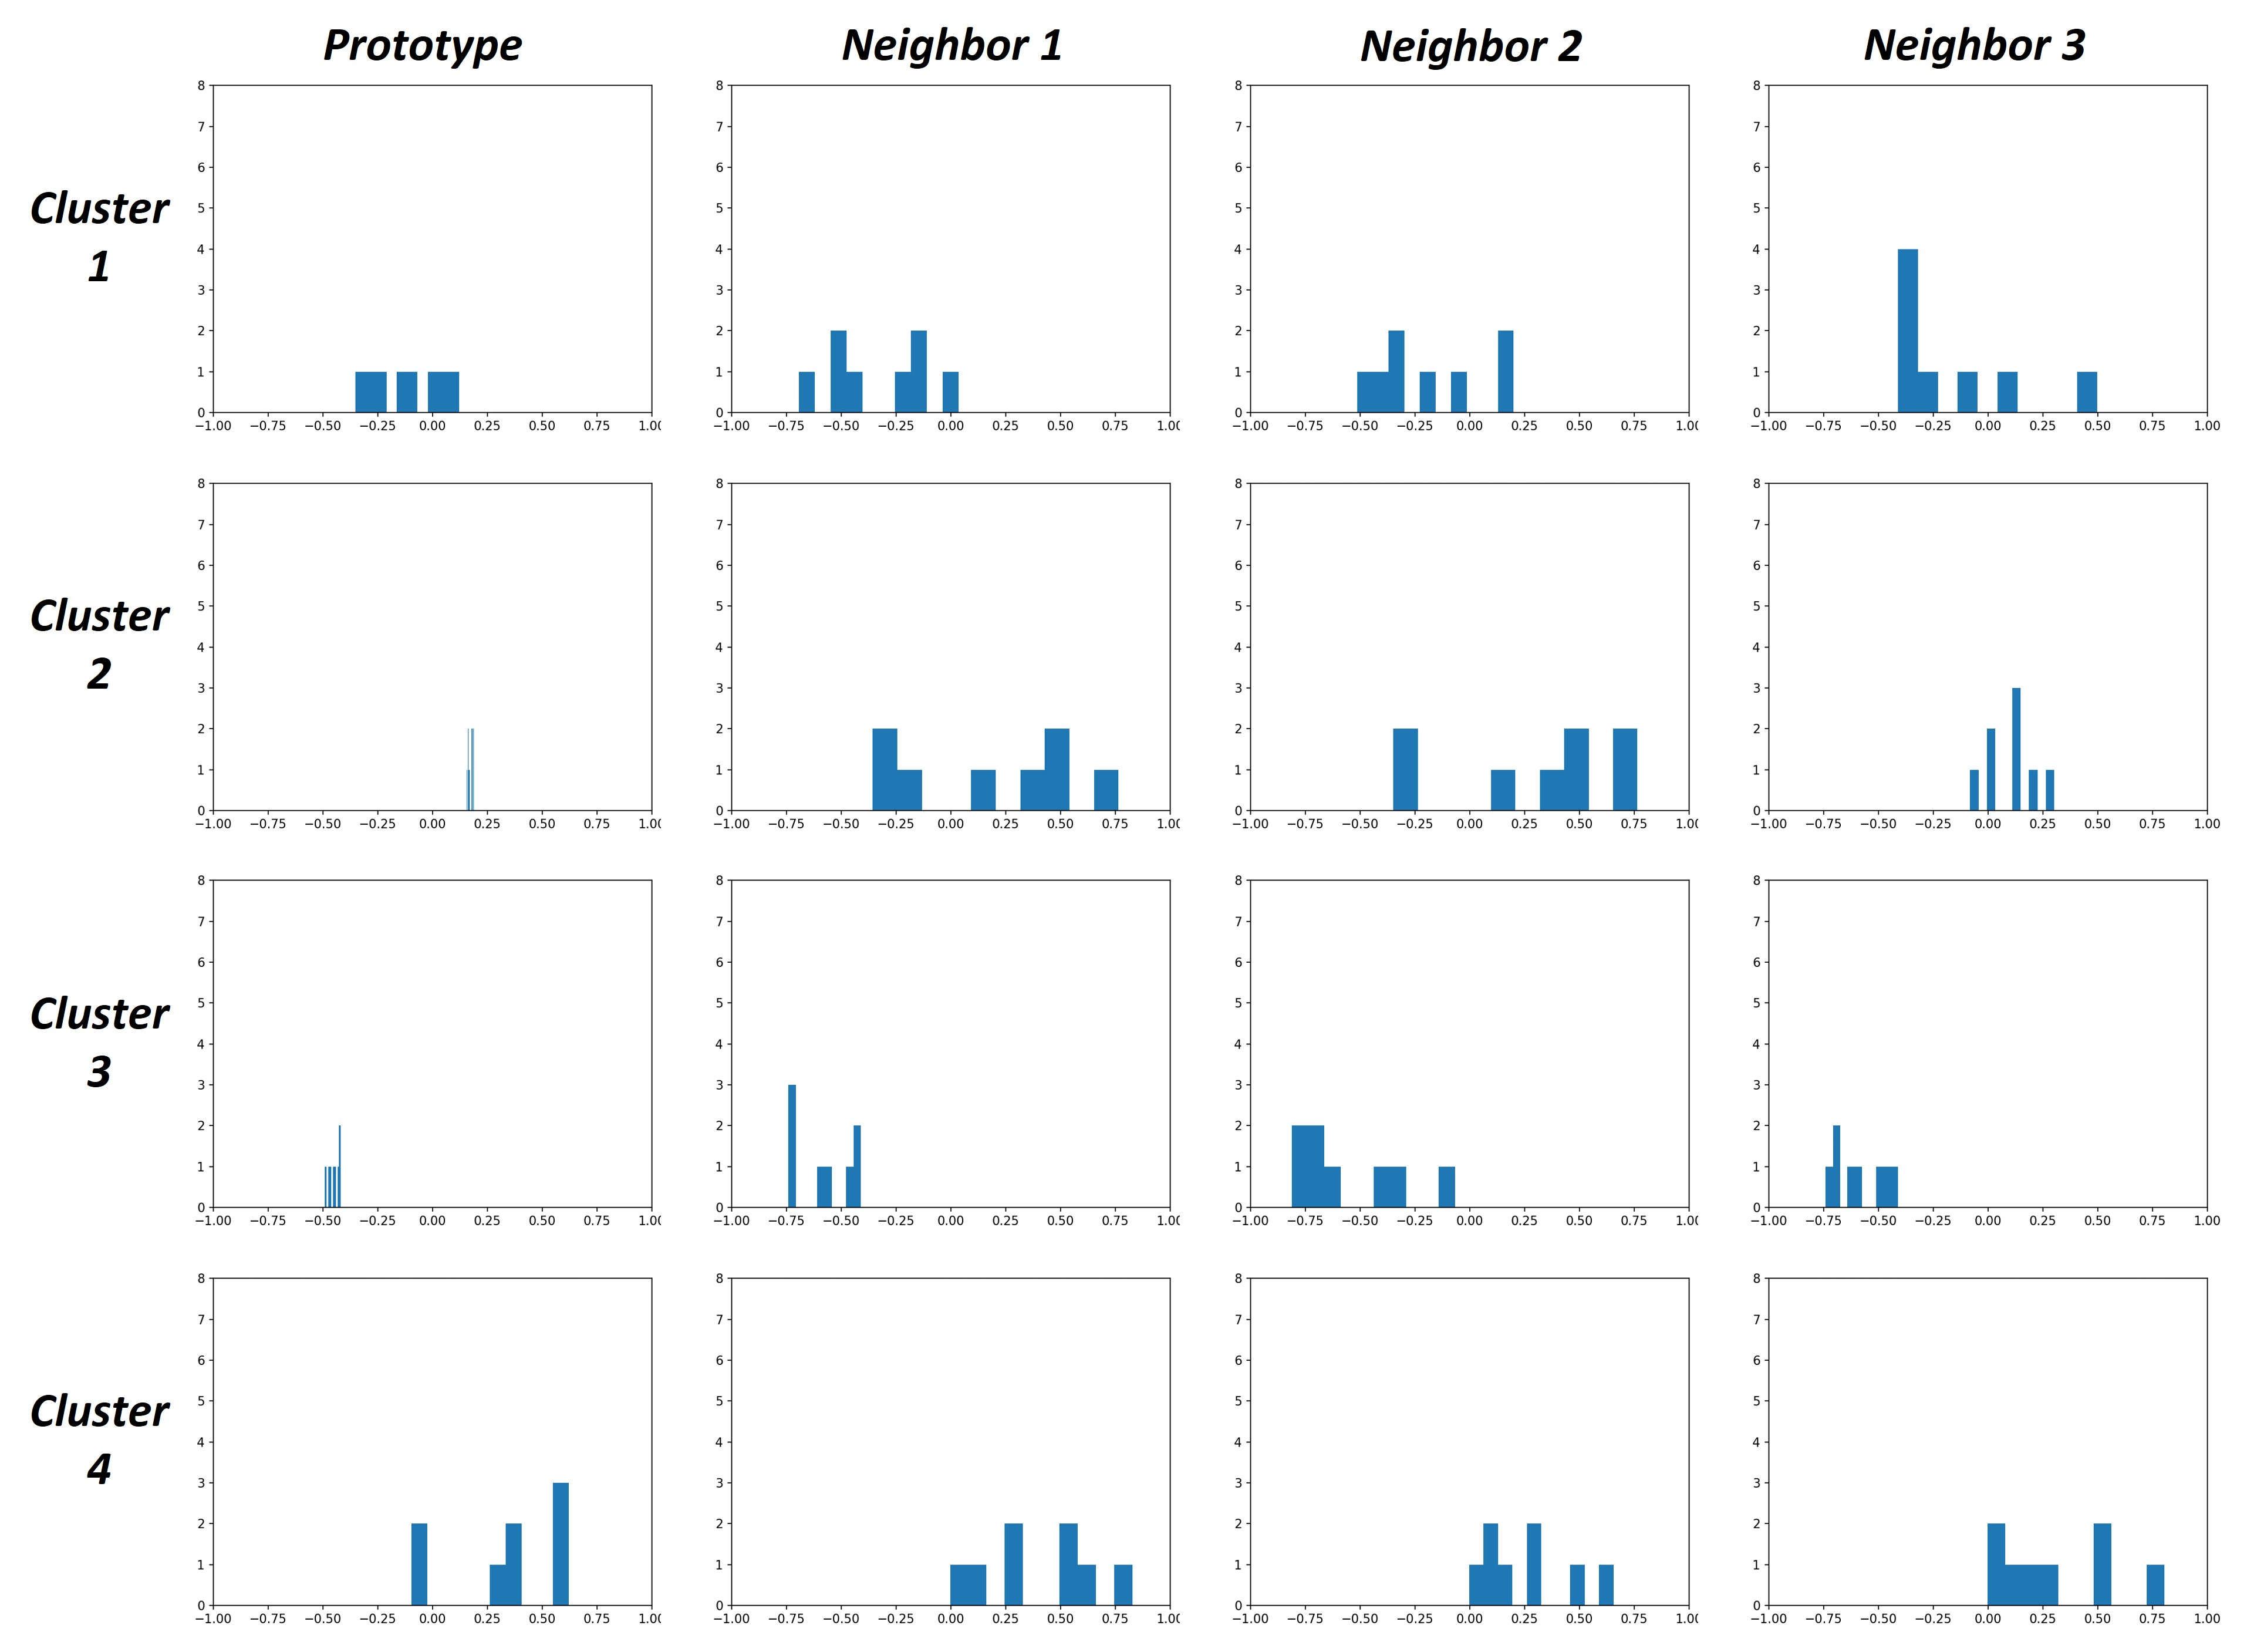}
\centering
\includegraphics[scale=0.48]{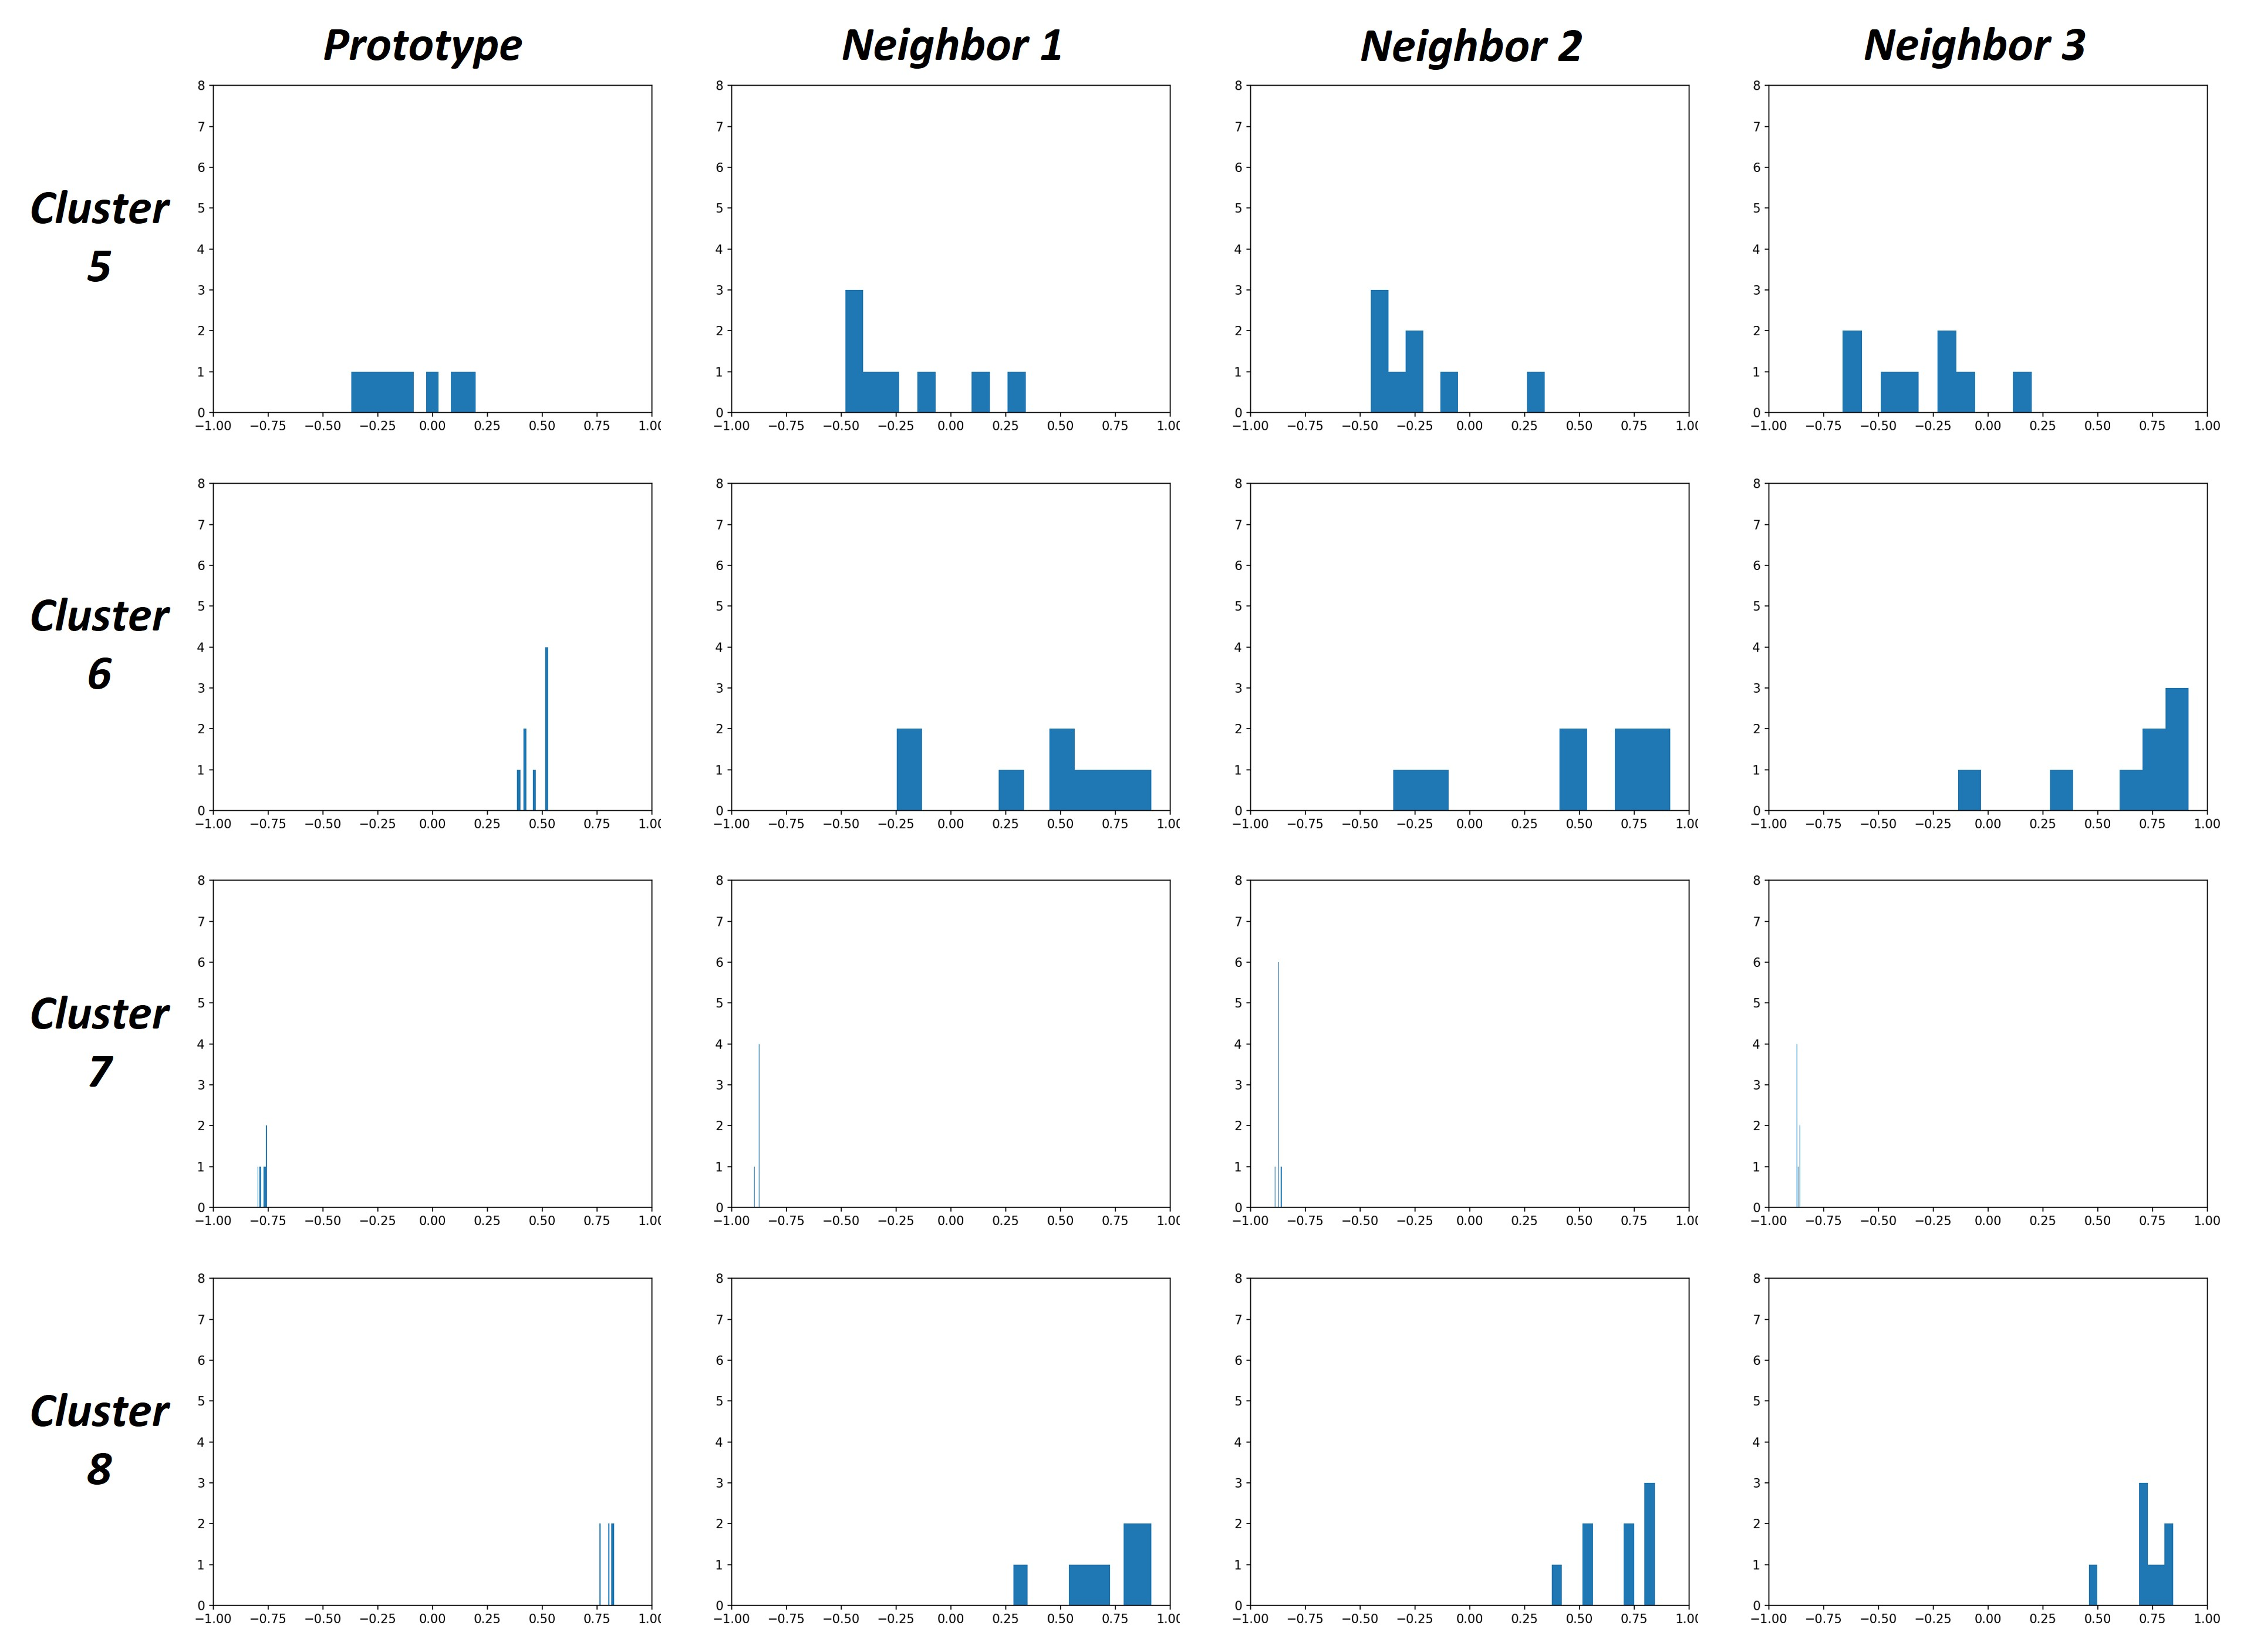}
\caption{The histogram of the eight centers (prototypes) and their neighbors in the \textbf{first band} of the flattened input. The band is in the \textbf{spatial domain}, and the prototypes are assigned according to the \textbf{L2-norm distance}.}
\label{fig:slice1_l2_spatial}
\end{figure*}

% slice 2
\begin{figure*}[h]
\centering
\includegraphics[scale=0.48]{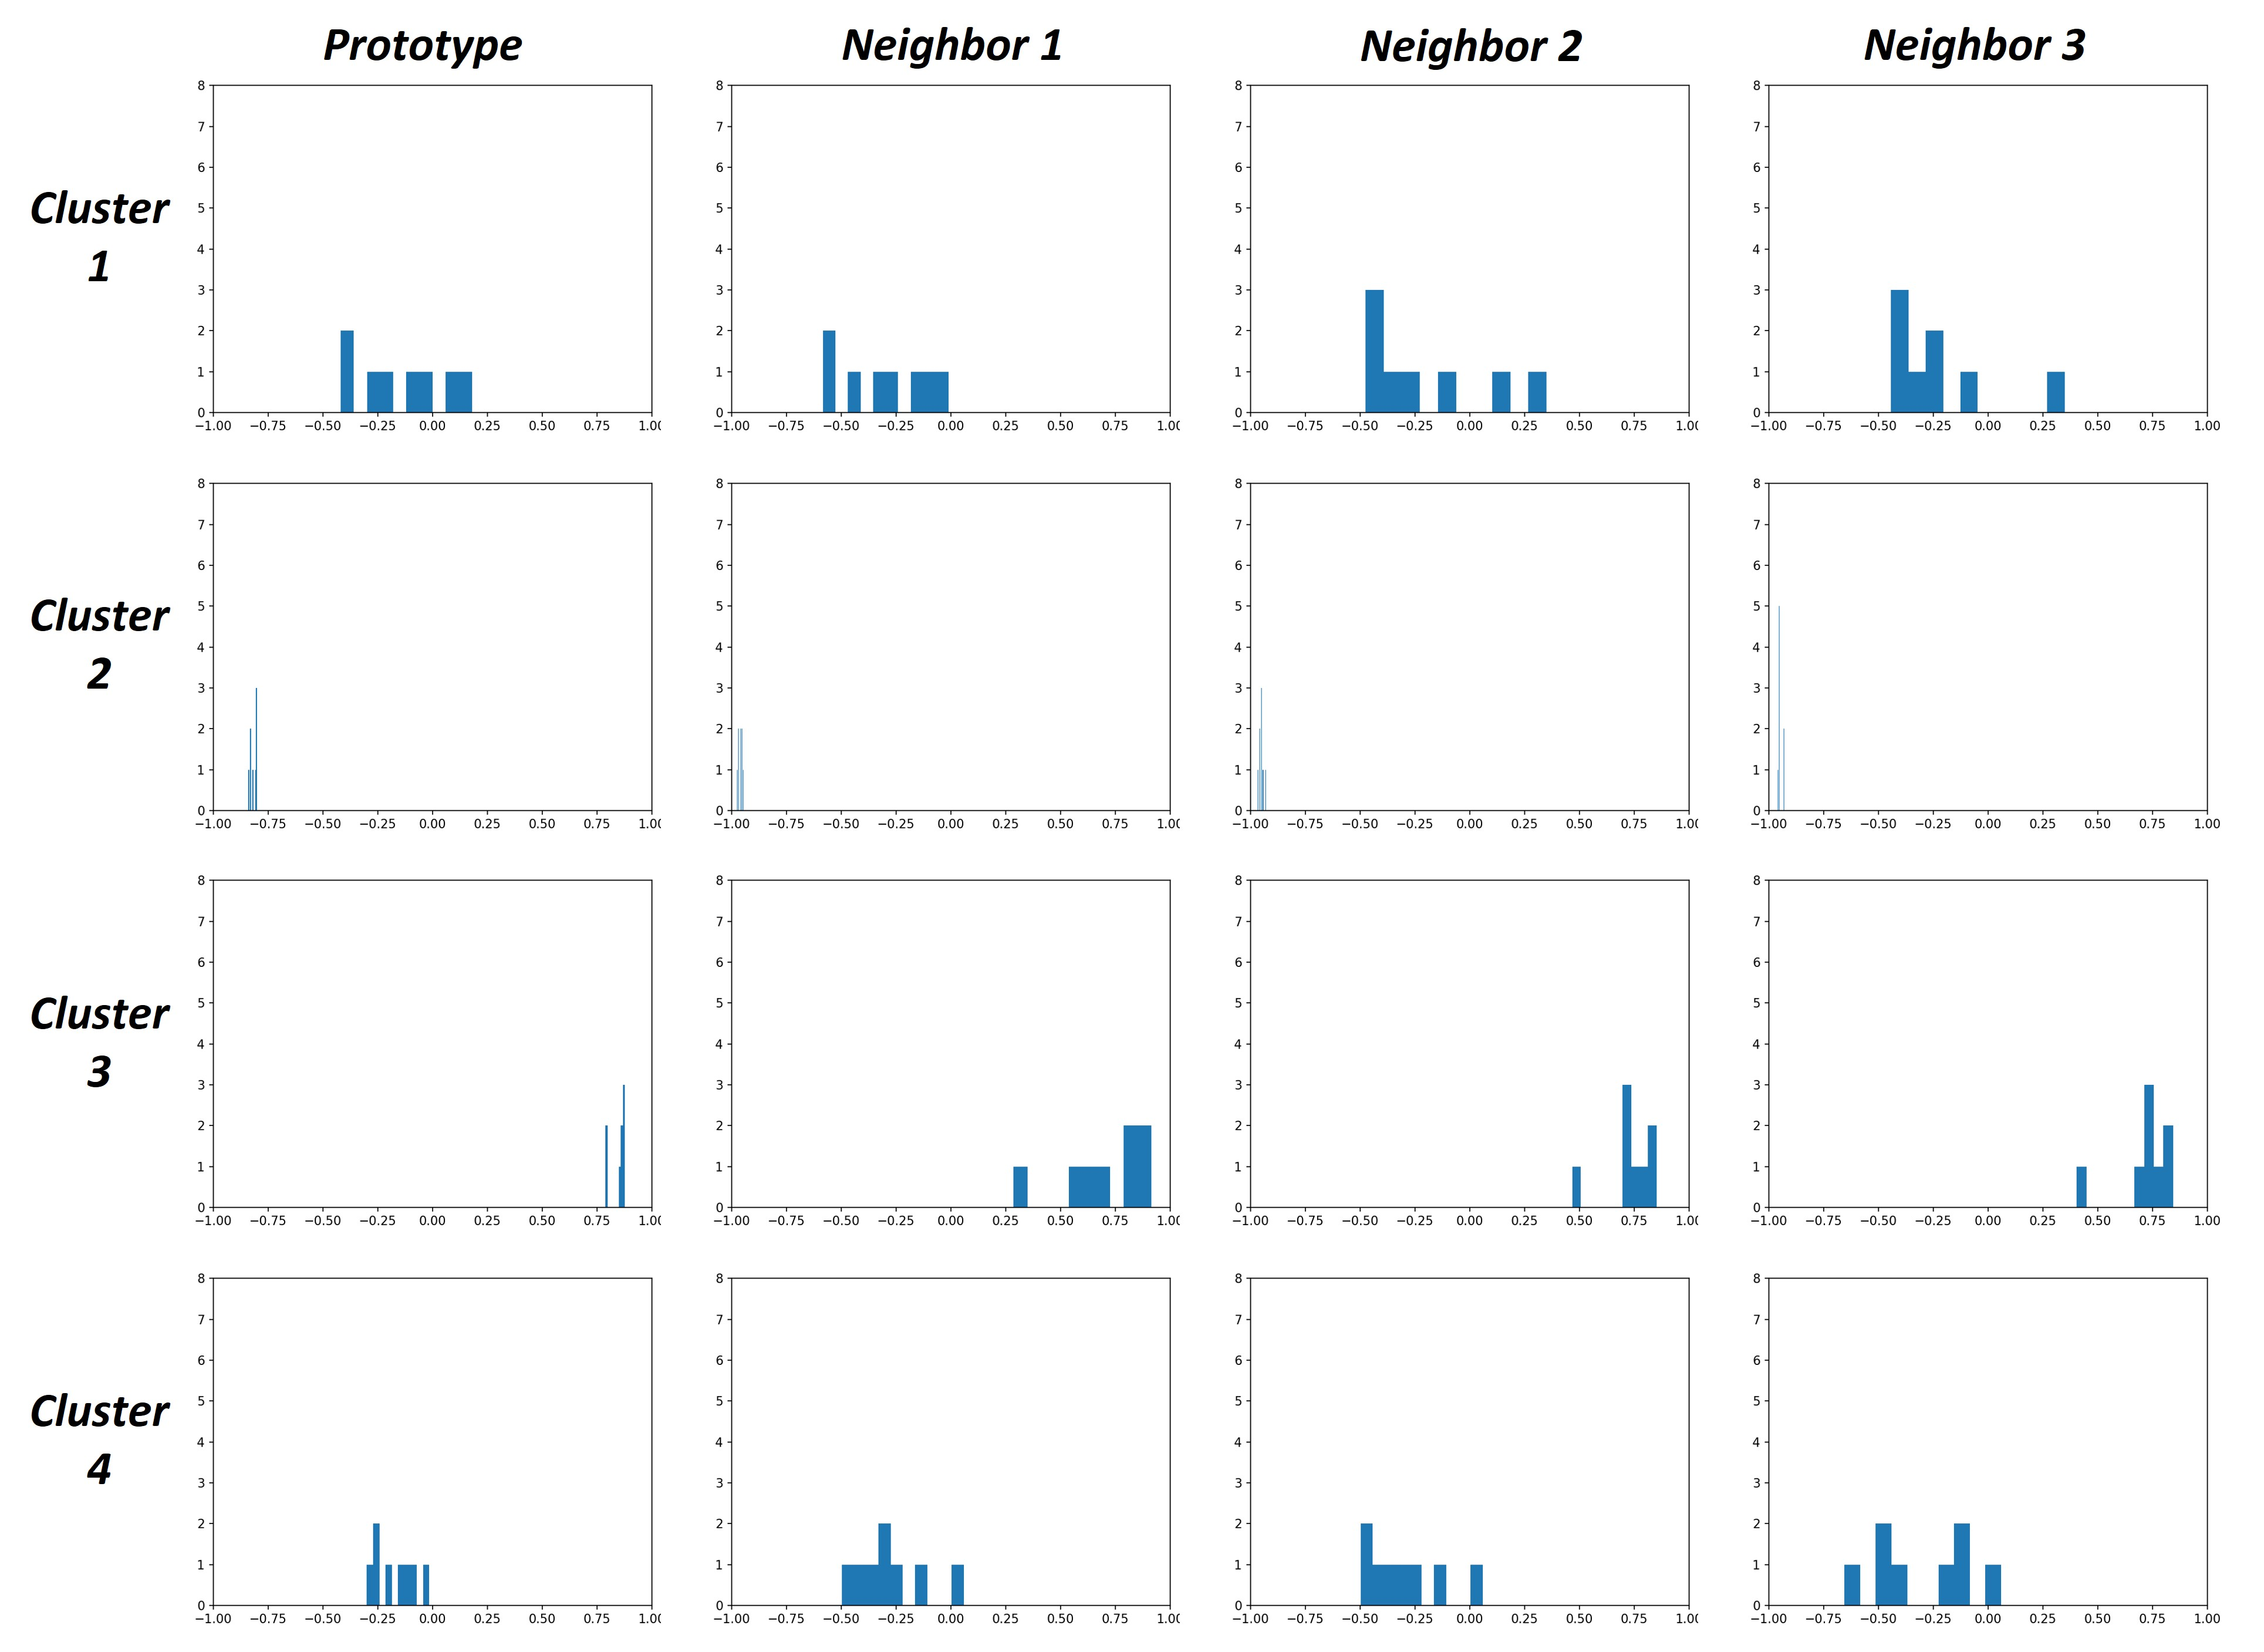}
\centering
\includegraphics[scale=0.48]{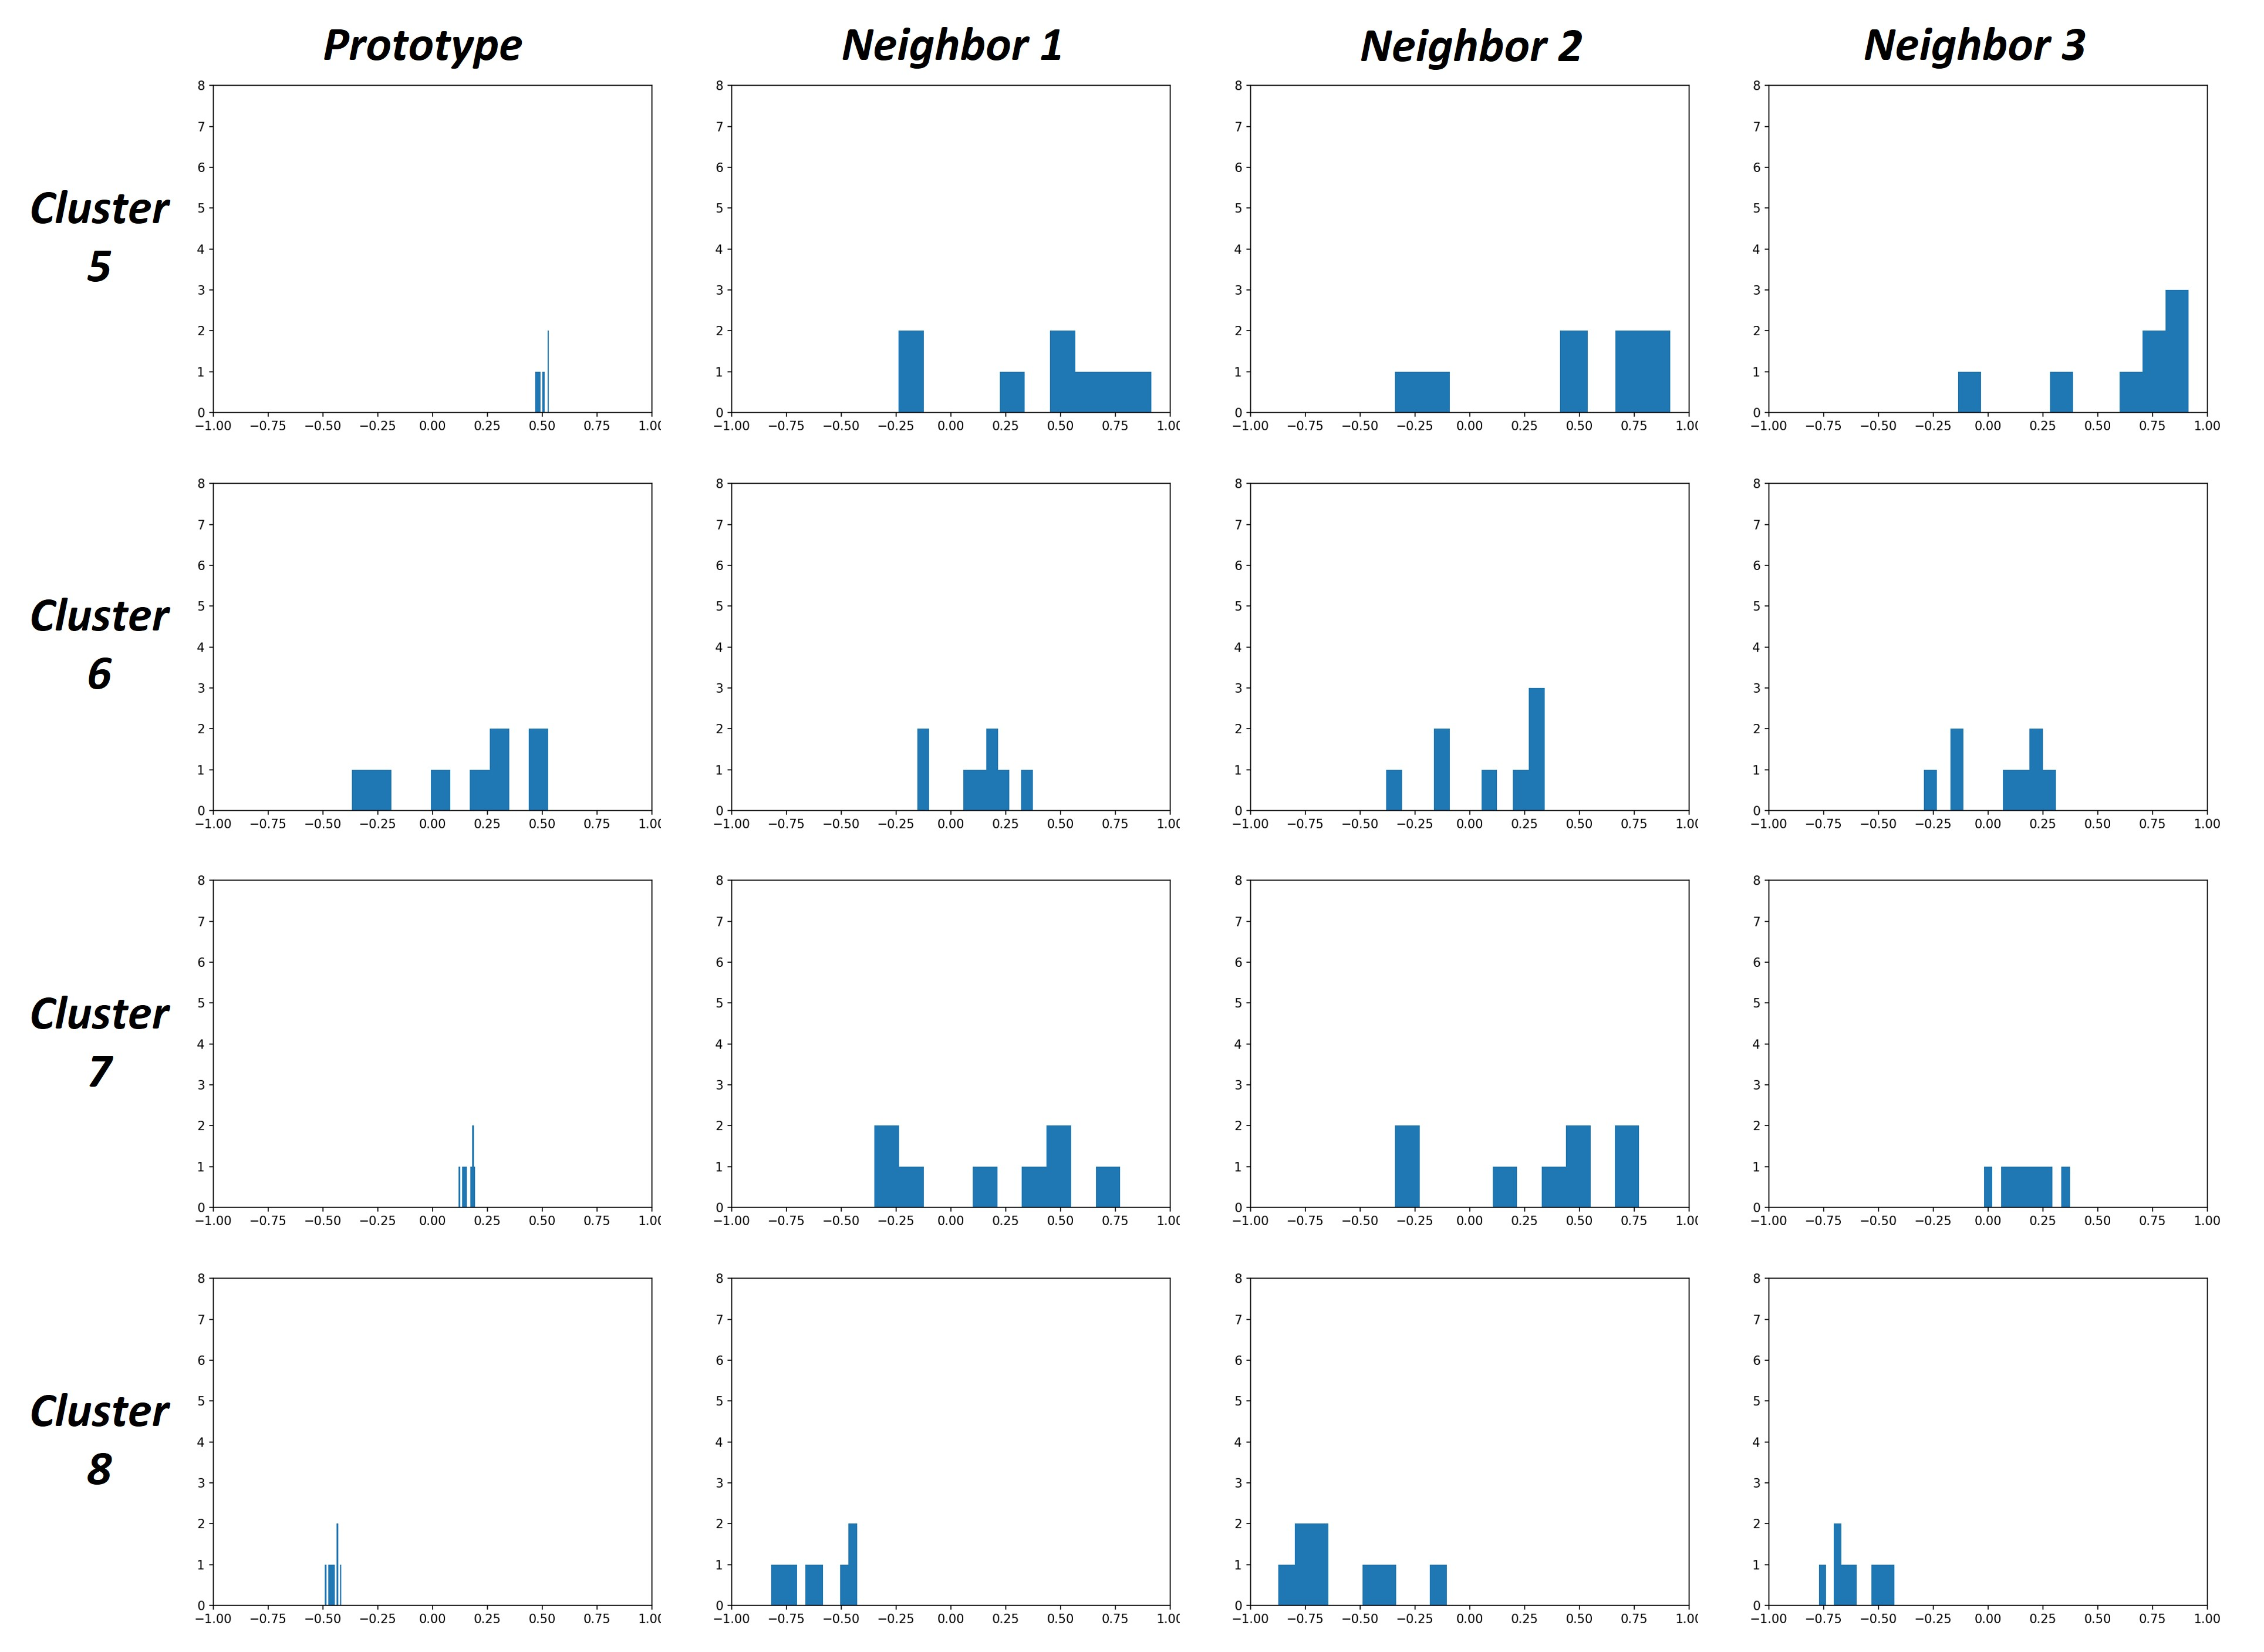}
\caption{The histogram of the eight centers (prototypes) and their neighbors in the \textbf{second band} of the flattened input. The band is in the \textbf{spatial domain}, and the prototypes are assigned according to the \textbf{L2-norm distance}.}
\label{fig:slice2_l2_spatial}
\end{figure*}

% slice 3
\begin{figure*}[h]
\centering
\includegraphics[scale=0.48]{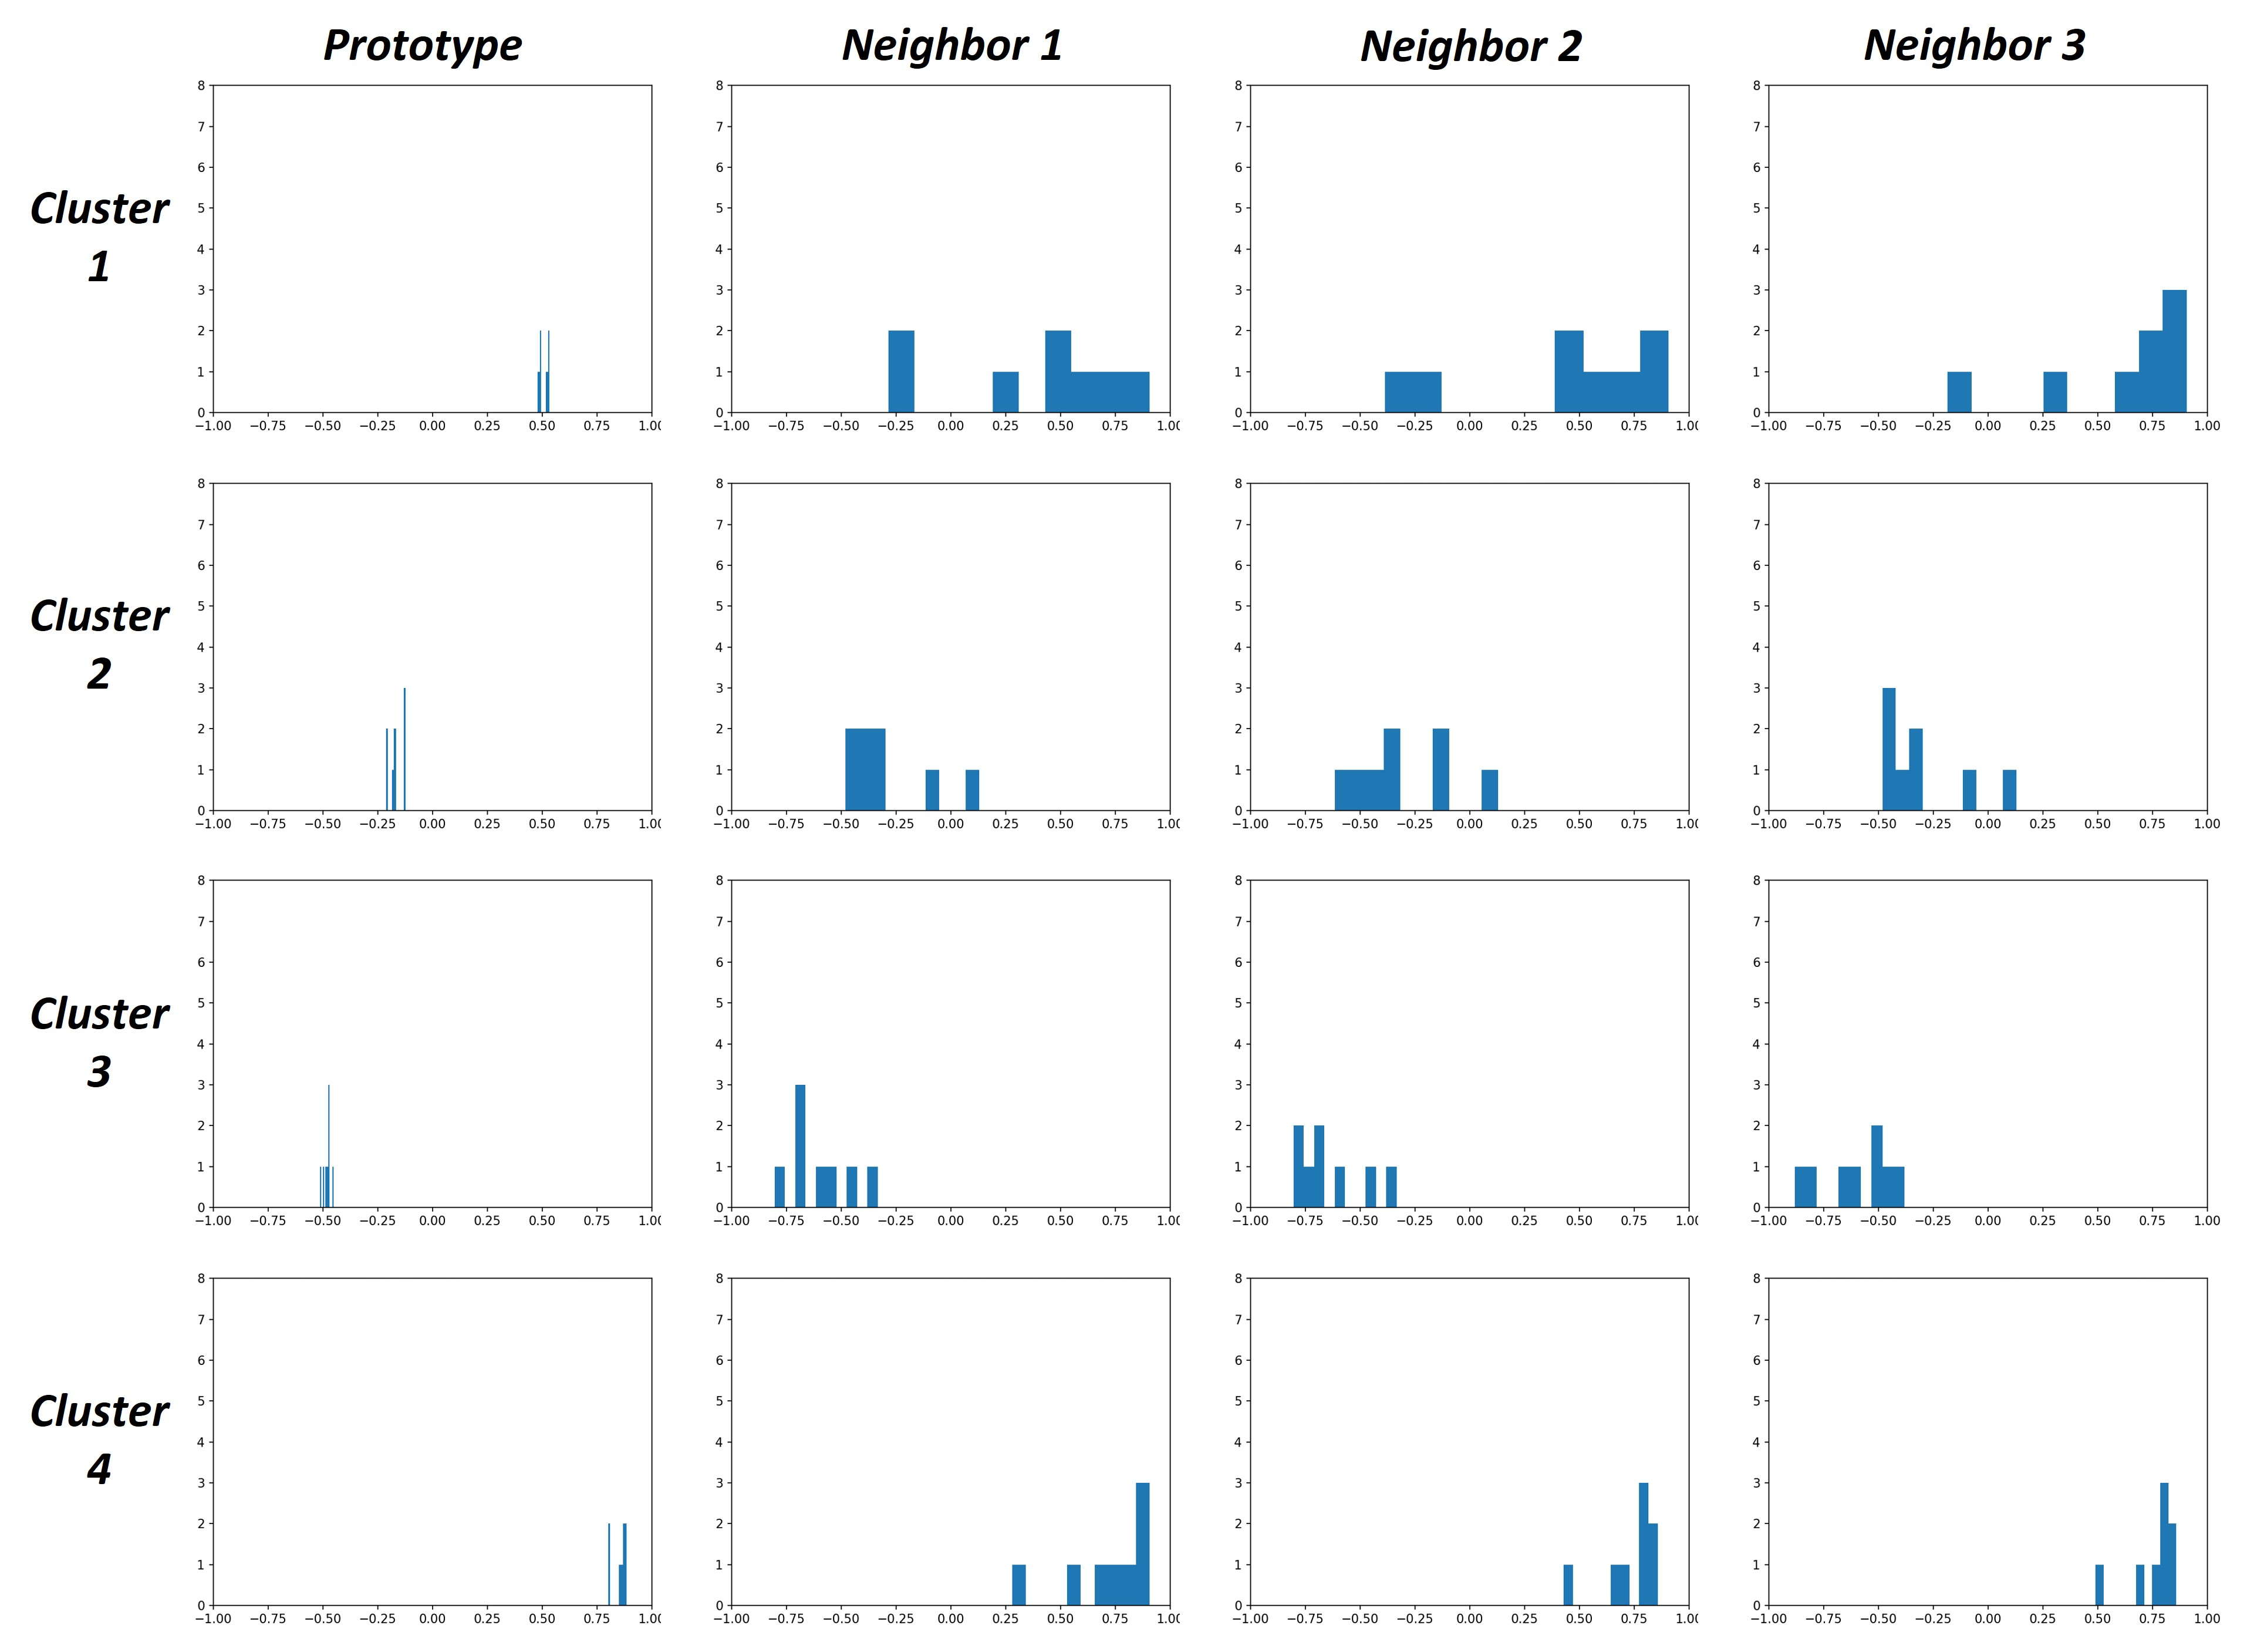}
\centering
\includegraphics[scale=0.48]{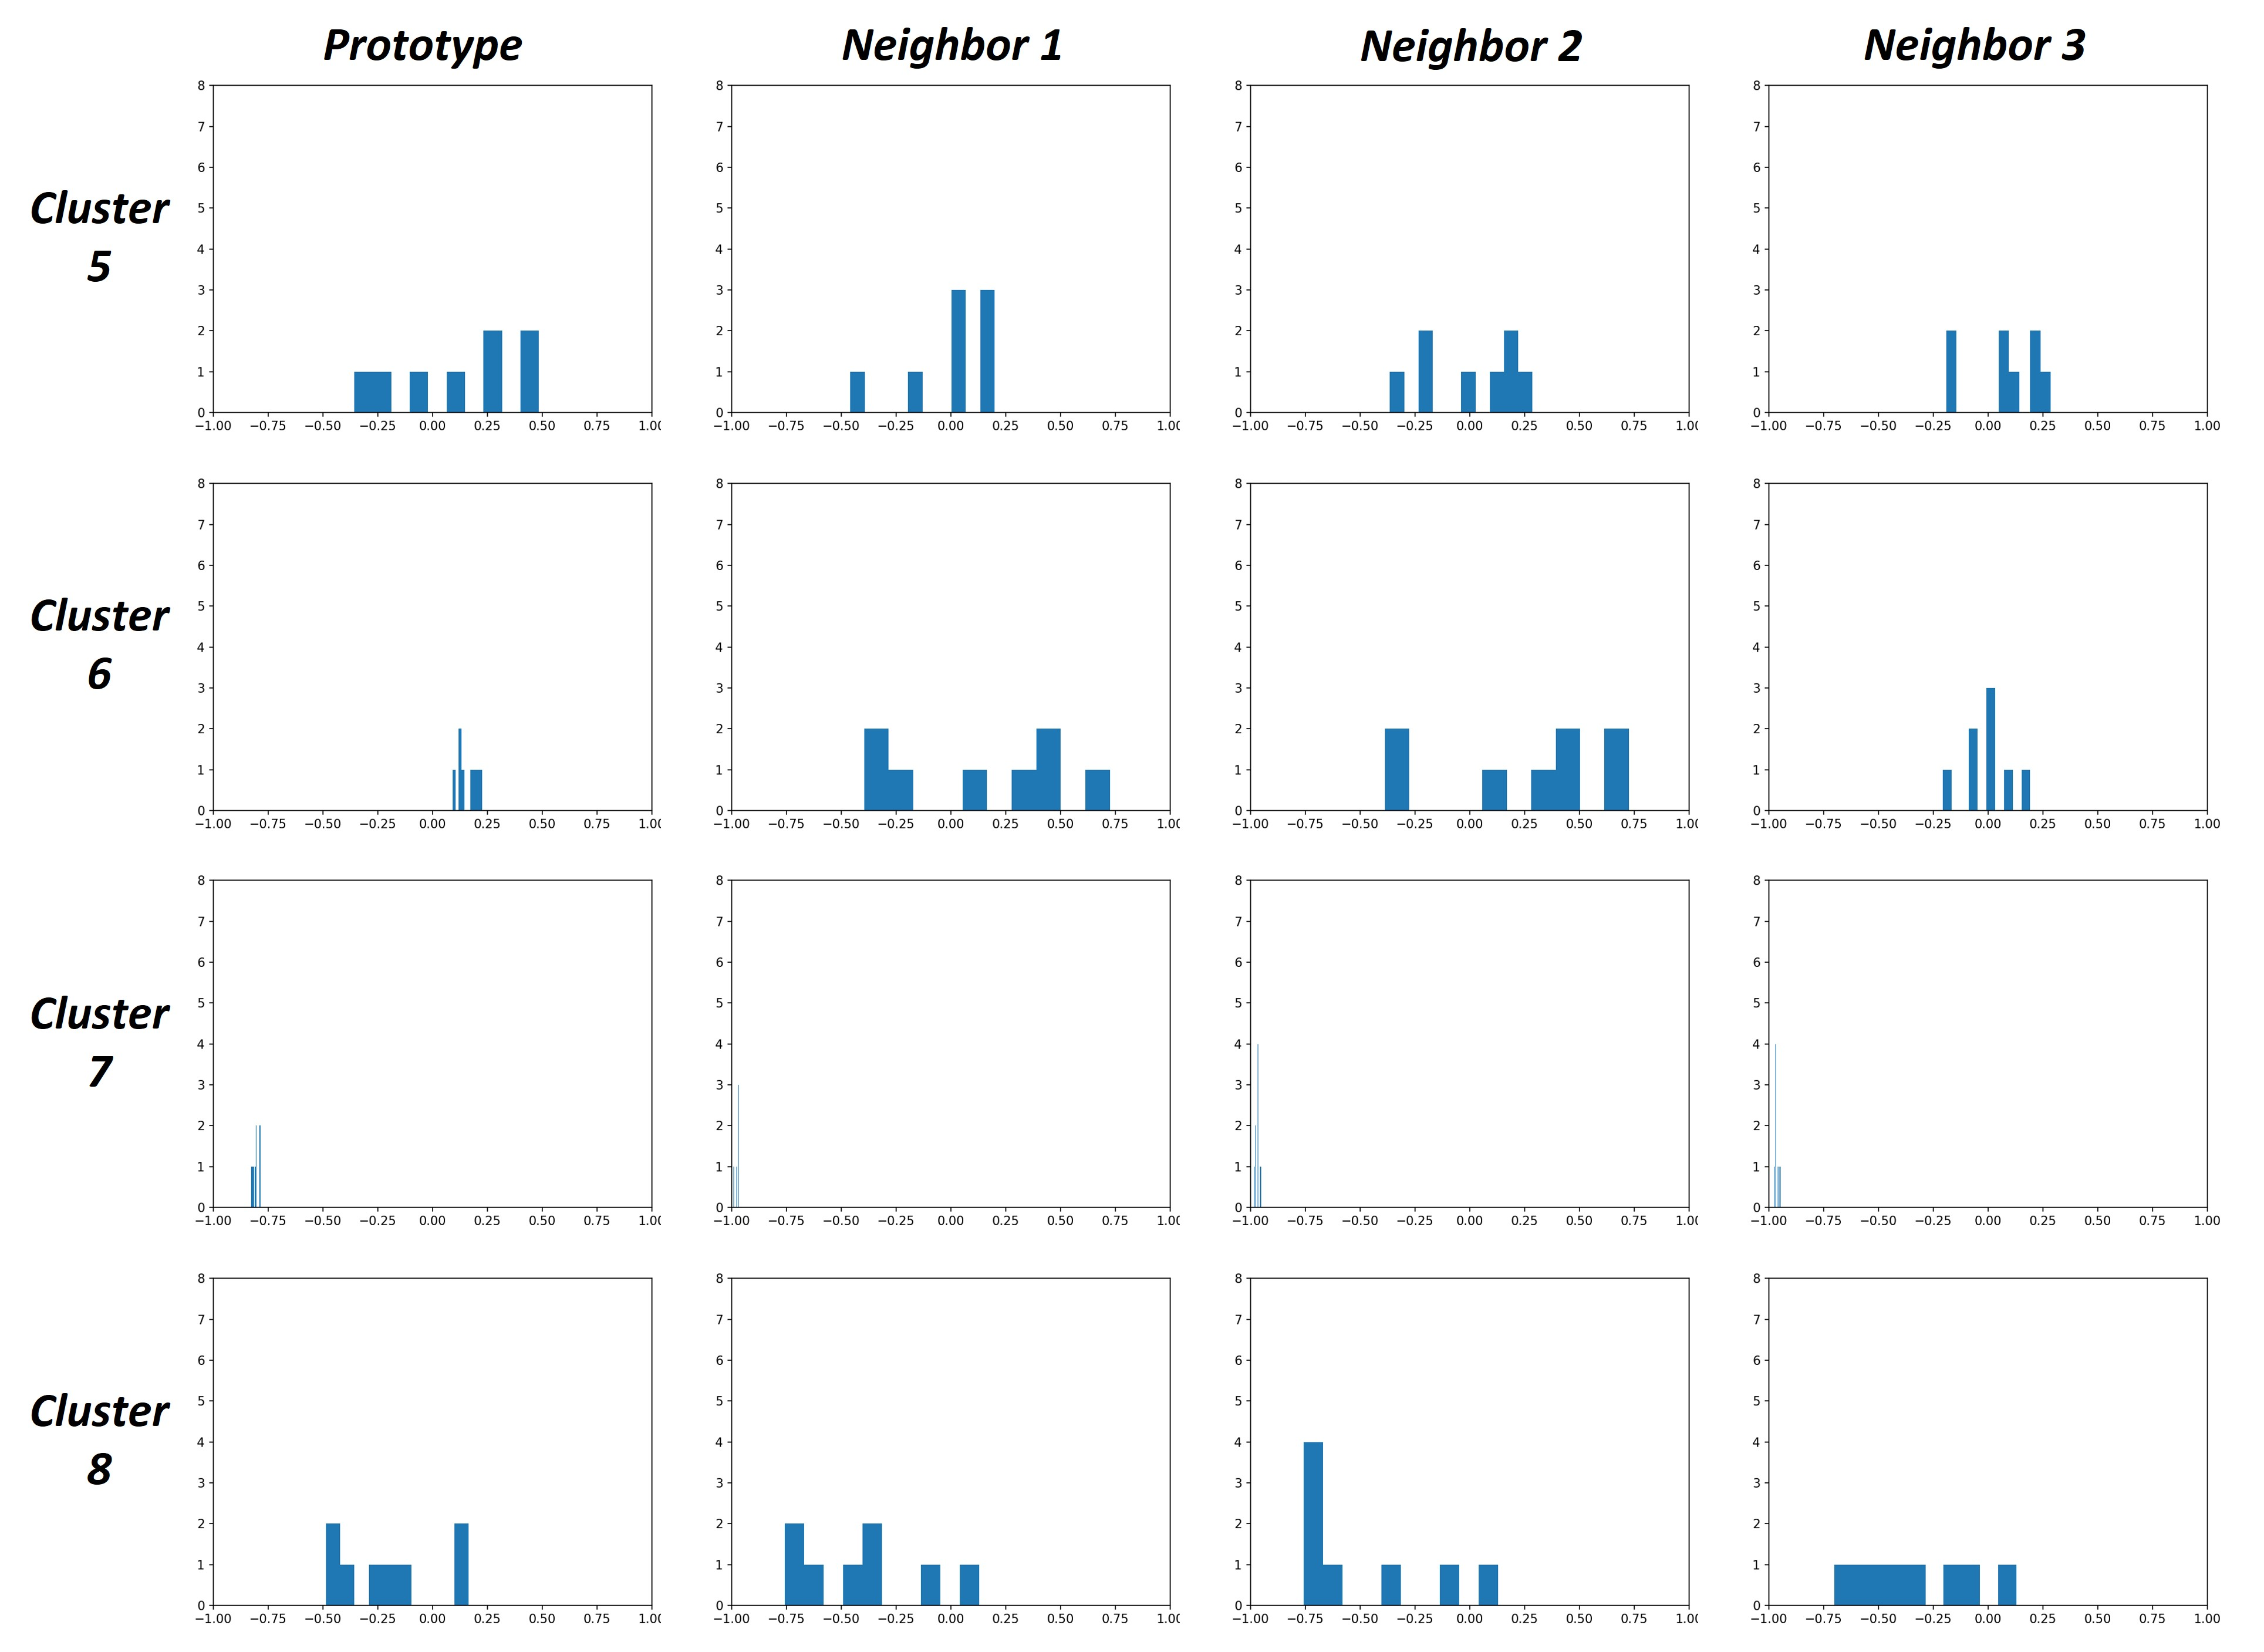}
\caption{The histogram of the eight centers (prototypes) and their neighbors in the \textbf{third band} of the flattened input. The band is in the \textbf{spatial domain}, and the prototypes are assigned according to the \textbf{L2-norm distance}.}
\label{fig:slice3_l2_spatial}
\end{figure*}

%%%%%%%%%% part 3 %%%%%%%%%%
\textbf{Centers and Selected Samples in Spatial Domain mapped to the Spectral Domain}

We draw Figure~\ref{fig:slice1_map} to \ref{fig:slice3_map} (Group 4) by applying WHT on the prototypes and their neighbors in Figure~\ref{fig:slice1_l2_spatial} to \ref{fig:slice3_l2_spatial}, respectively. We aim to determine whether the prototype and its neighbors found in the spatial domain based on L2-norm distance will keep their relations after being mapped to the spectral domain by WHT. 

Remark:
\begin{enumerate}
\item The corresponding subfigures in the Group 3 and 4 are the same.
\end{enumerate}

% slice 1
\begin{figure*}[h]
\centering
\includegraphics[scale=0.5]{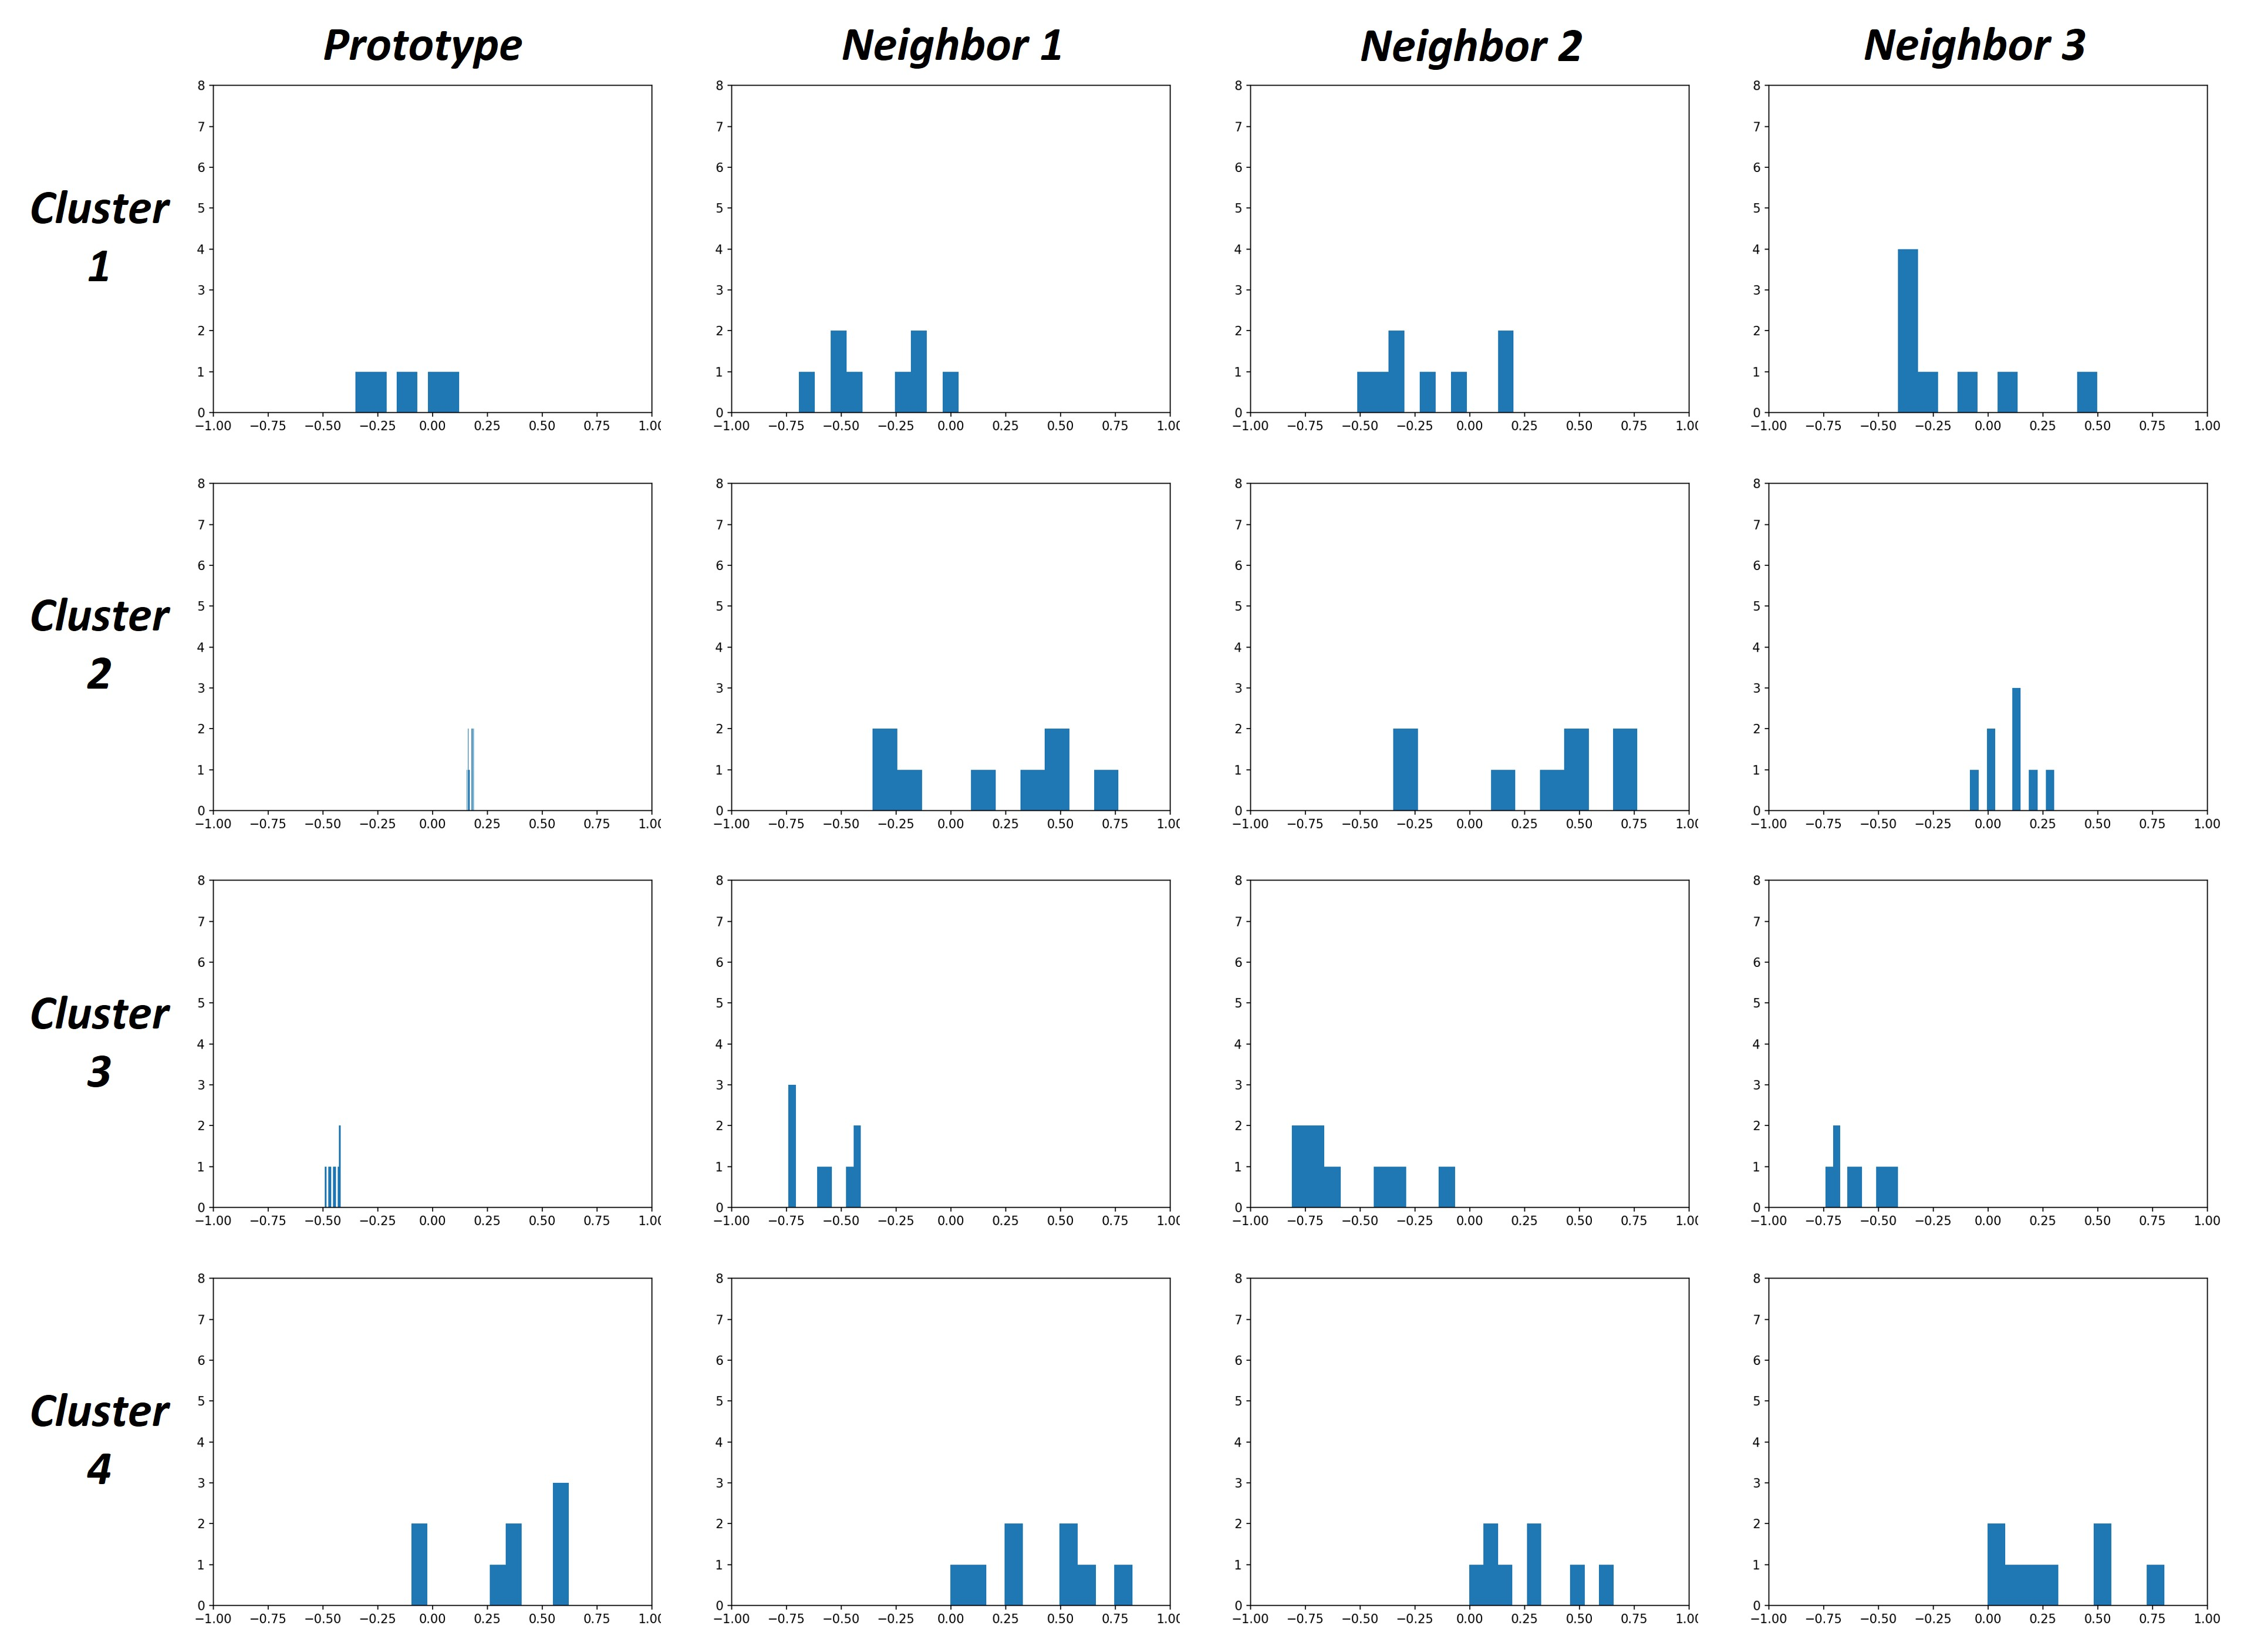}
\centering
\includegraphics[scale=0.5]{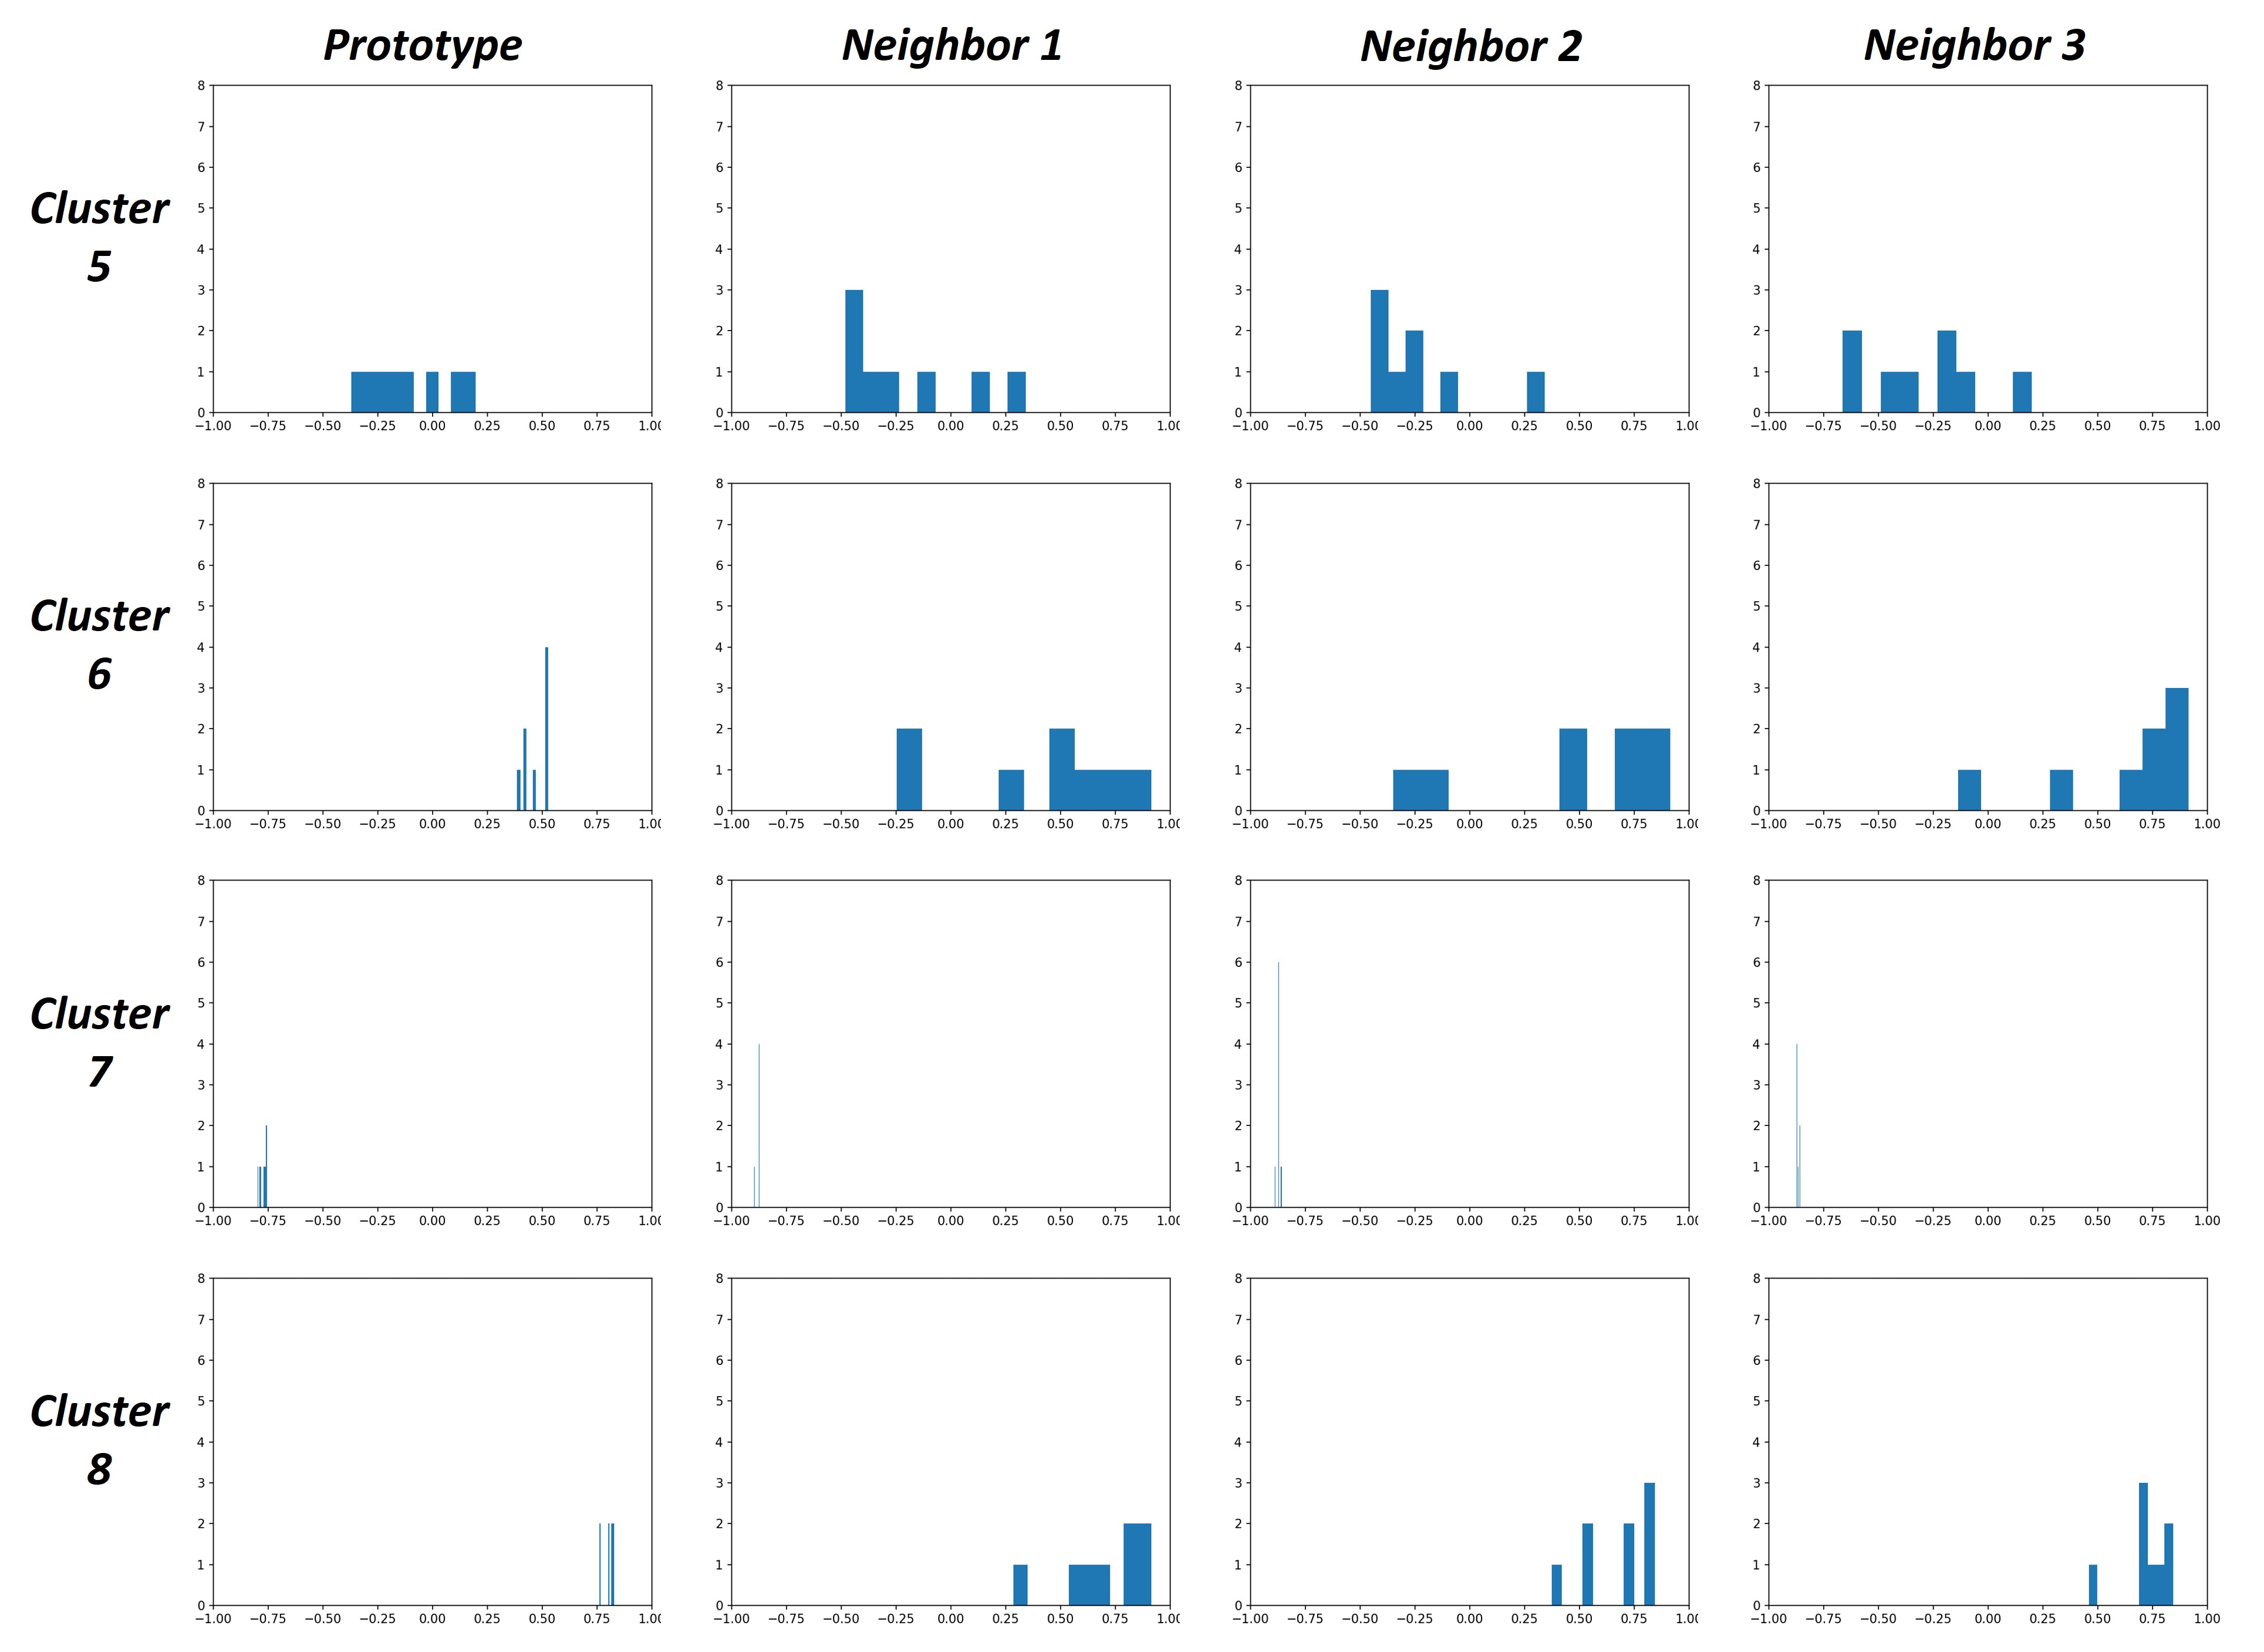}
\caption{Applying WHT to Figure~\ref{fig:slice1_l2_spatial}.}
\label{fig:slice1_map}
\end{figure*}

% slice 2
\begin{figure*}[h]
\centering
\includegraphics[scale=0.5]{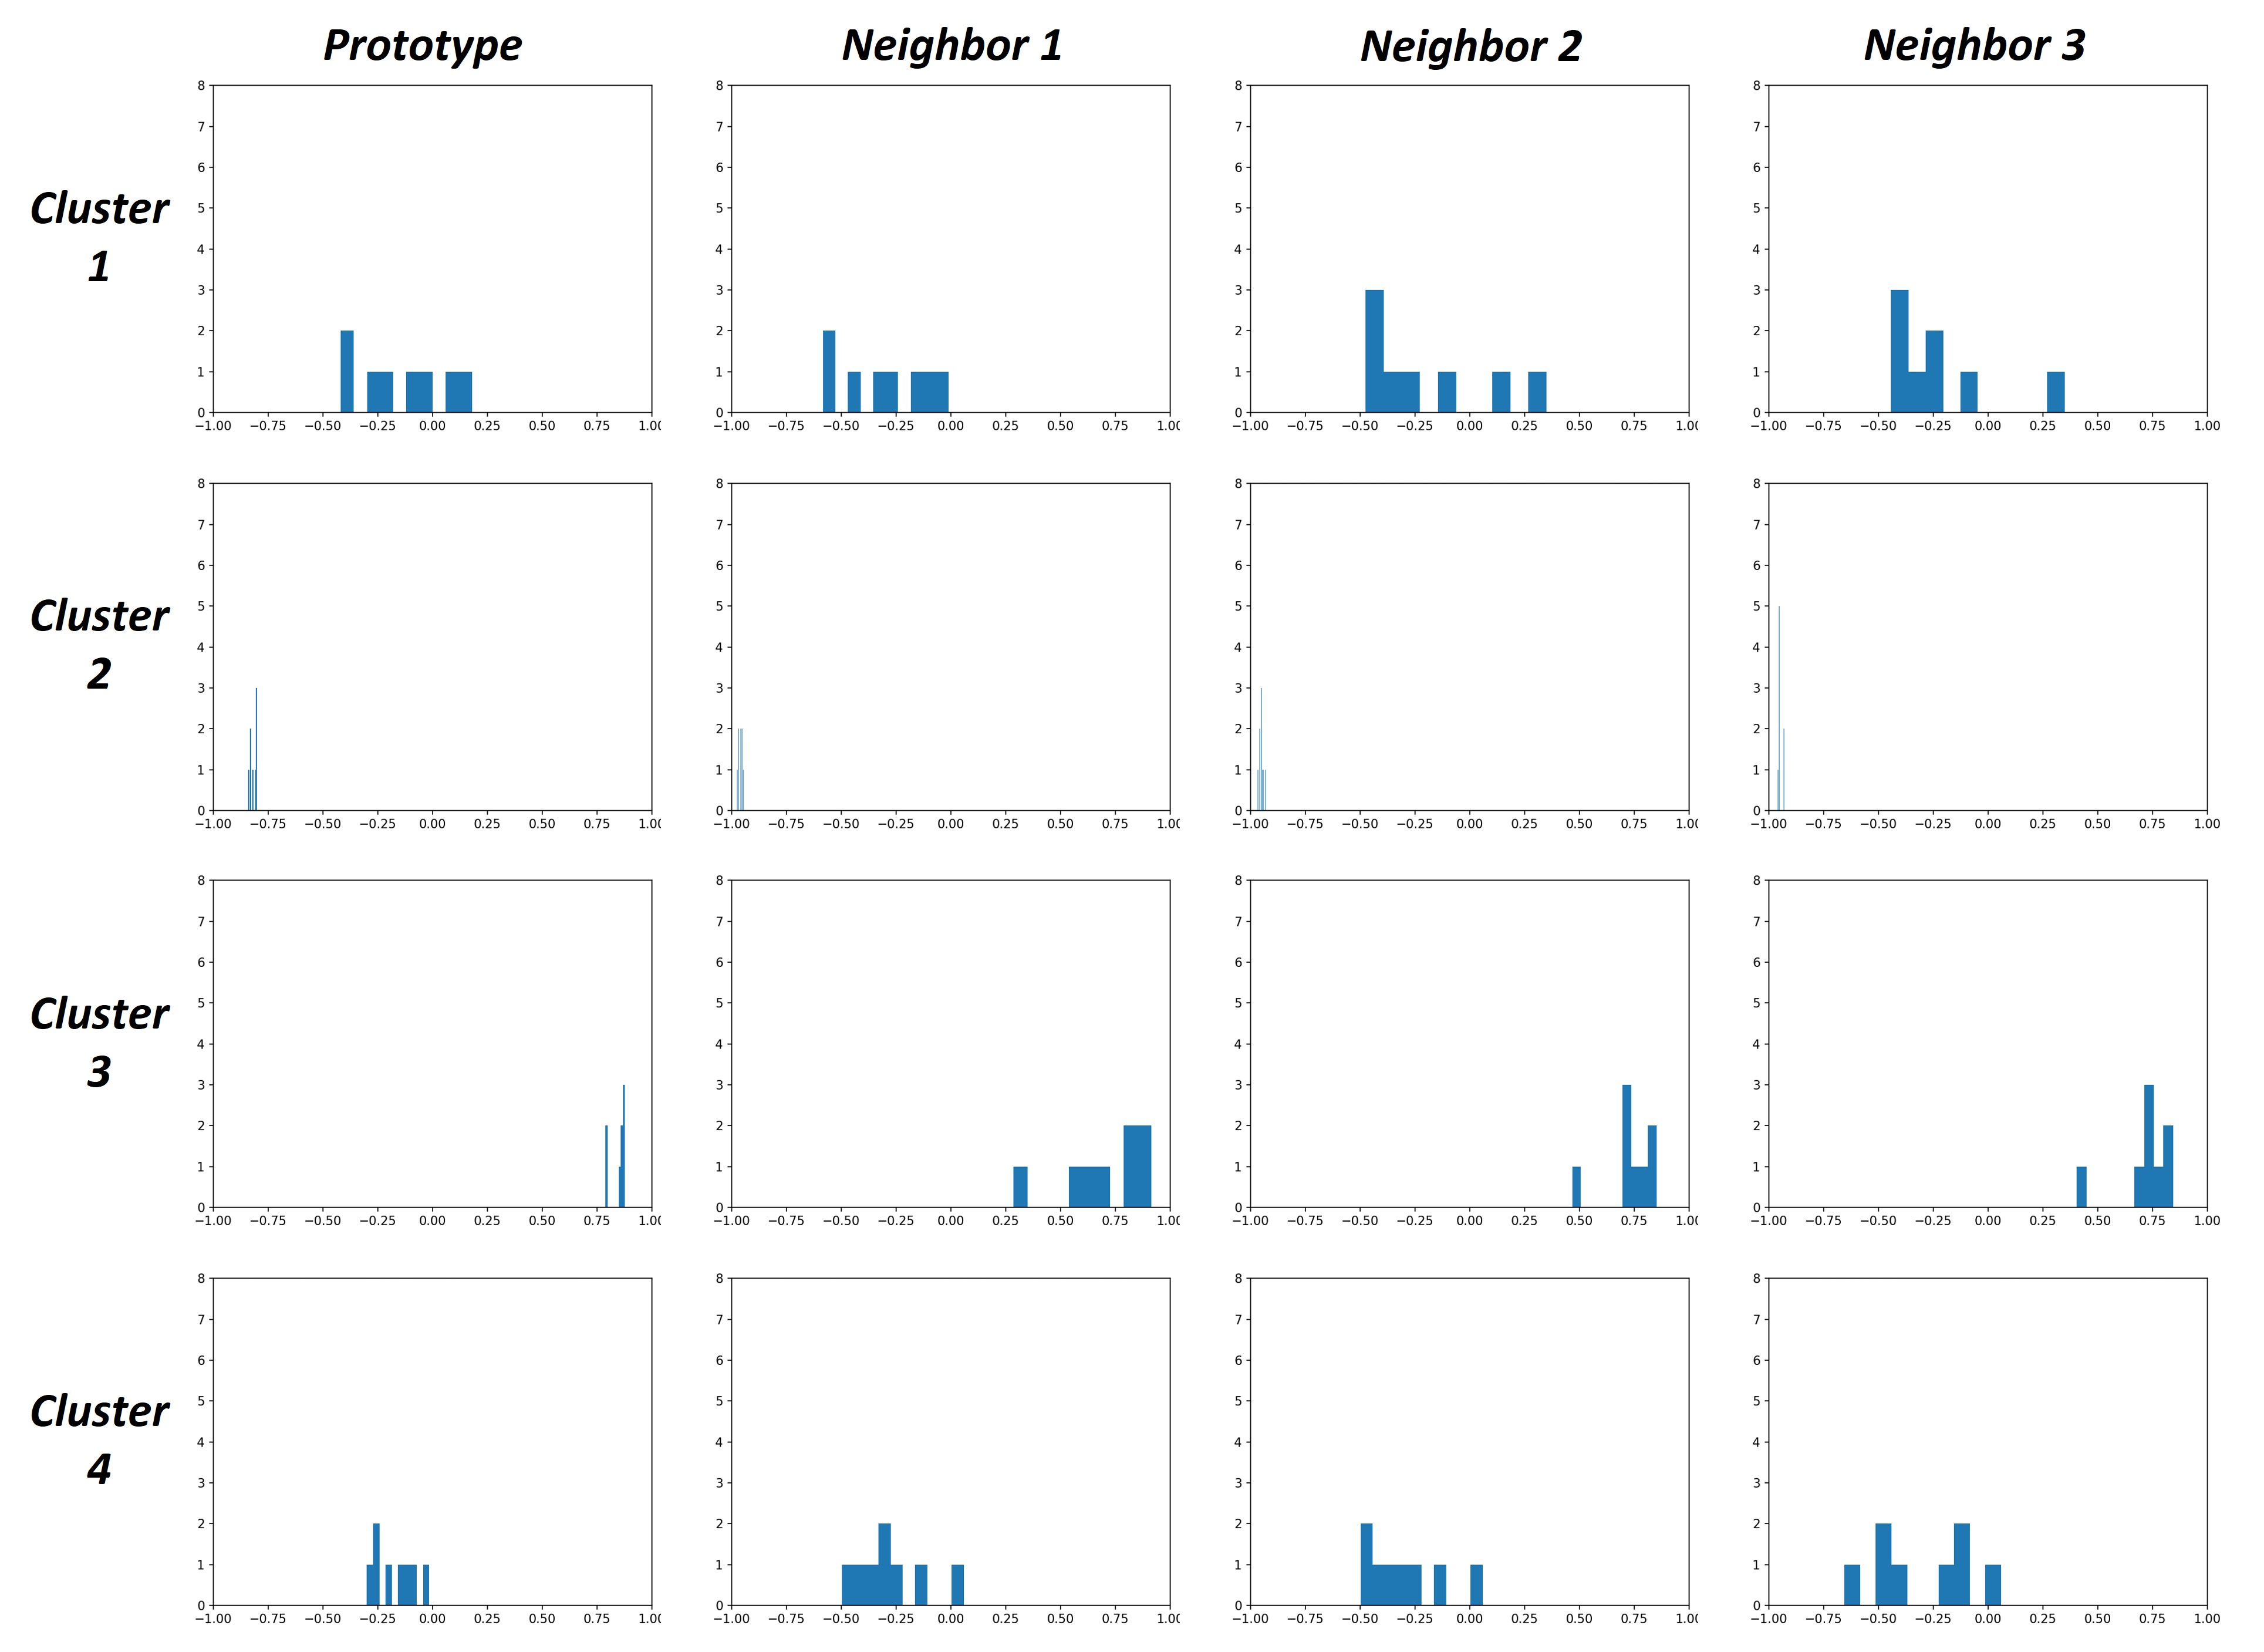}
\centering
\includegraphics[scale=0.5]{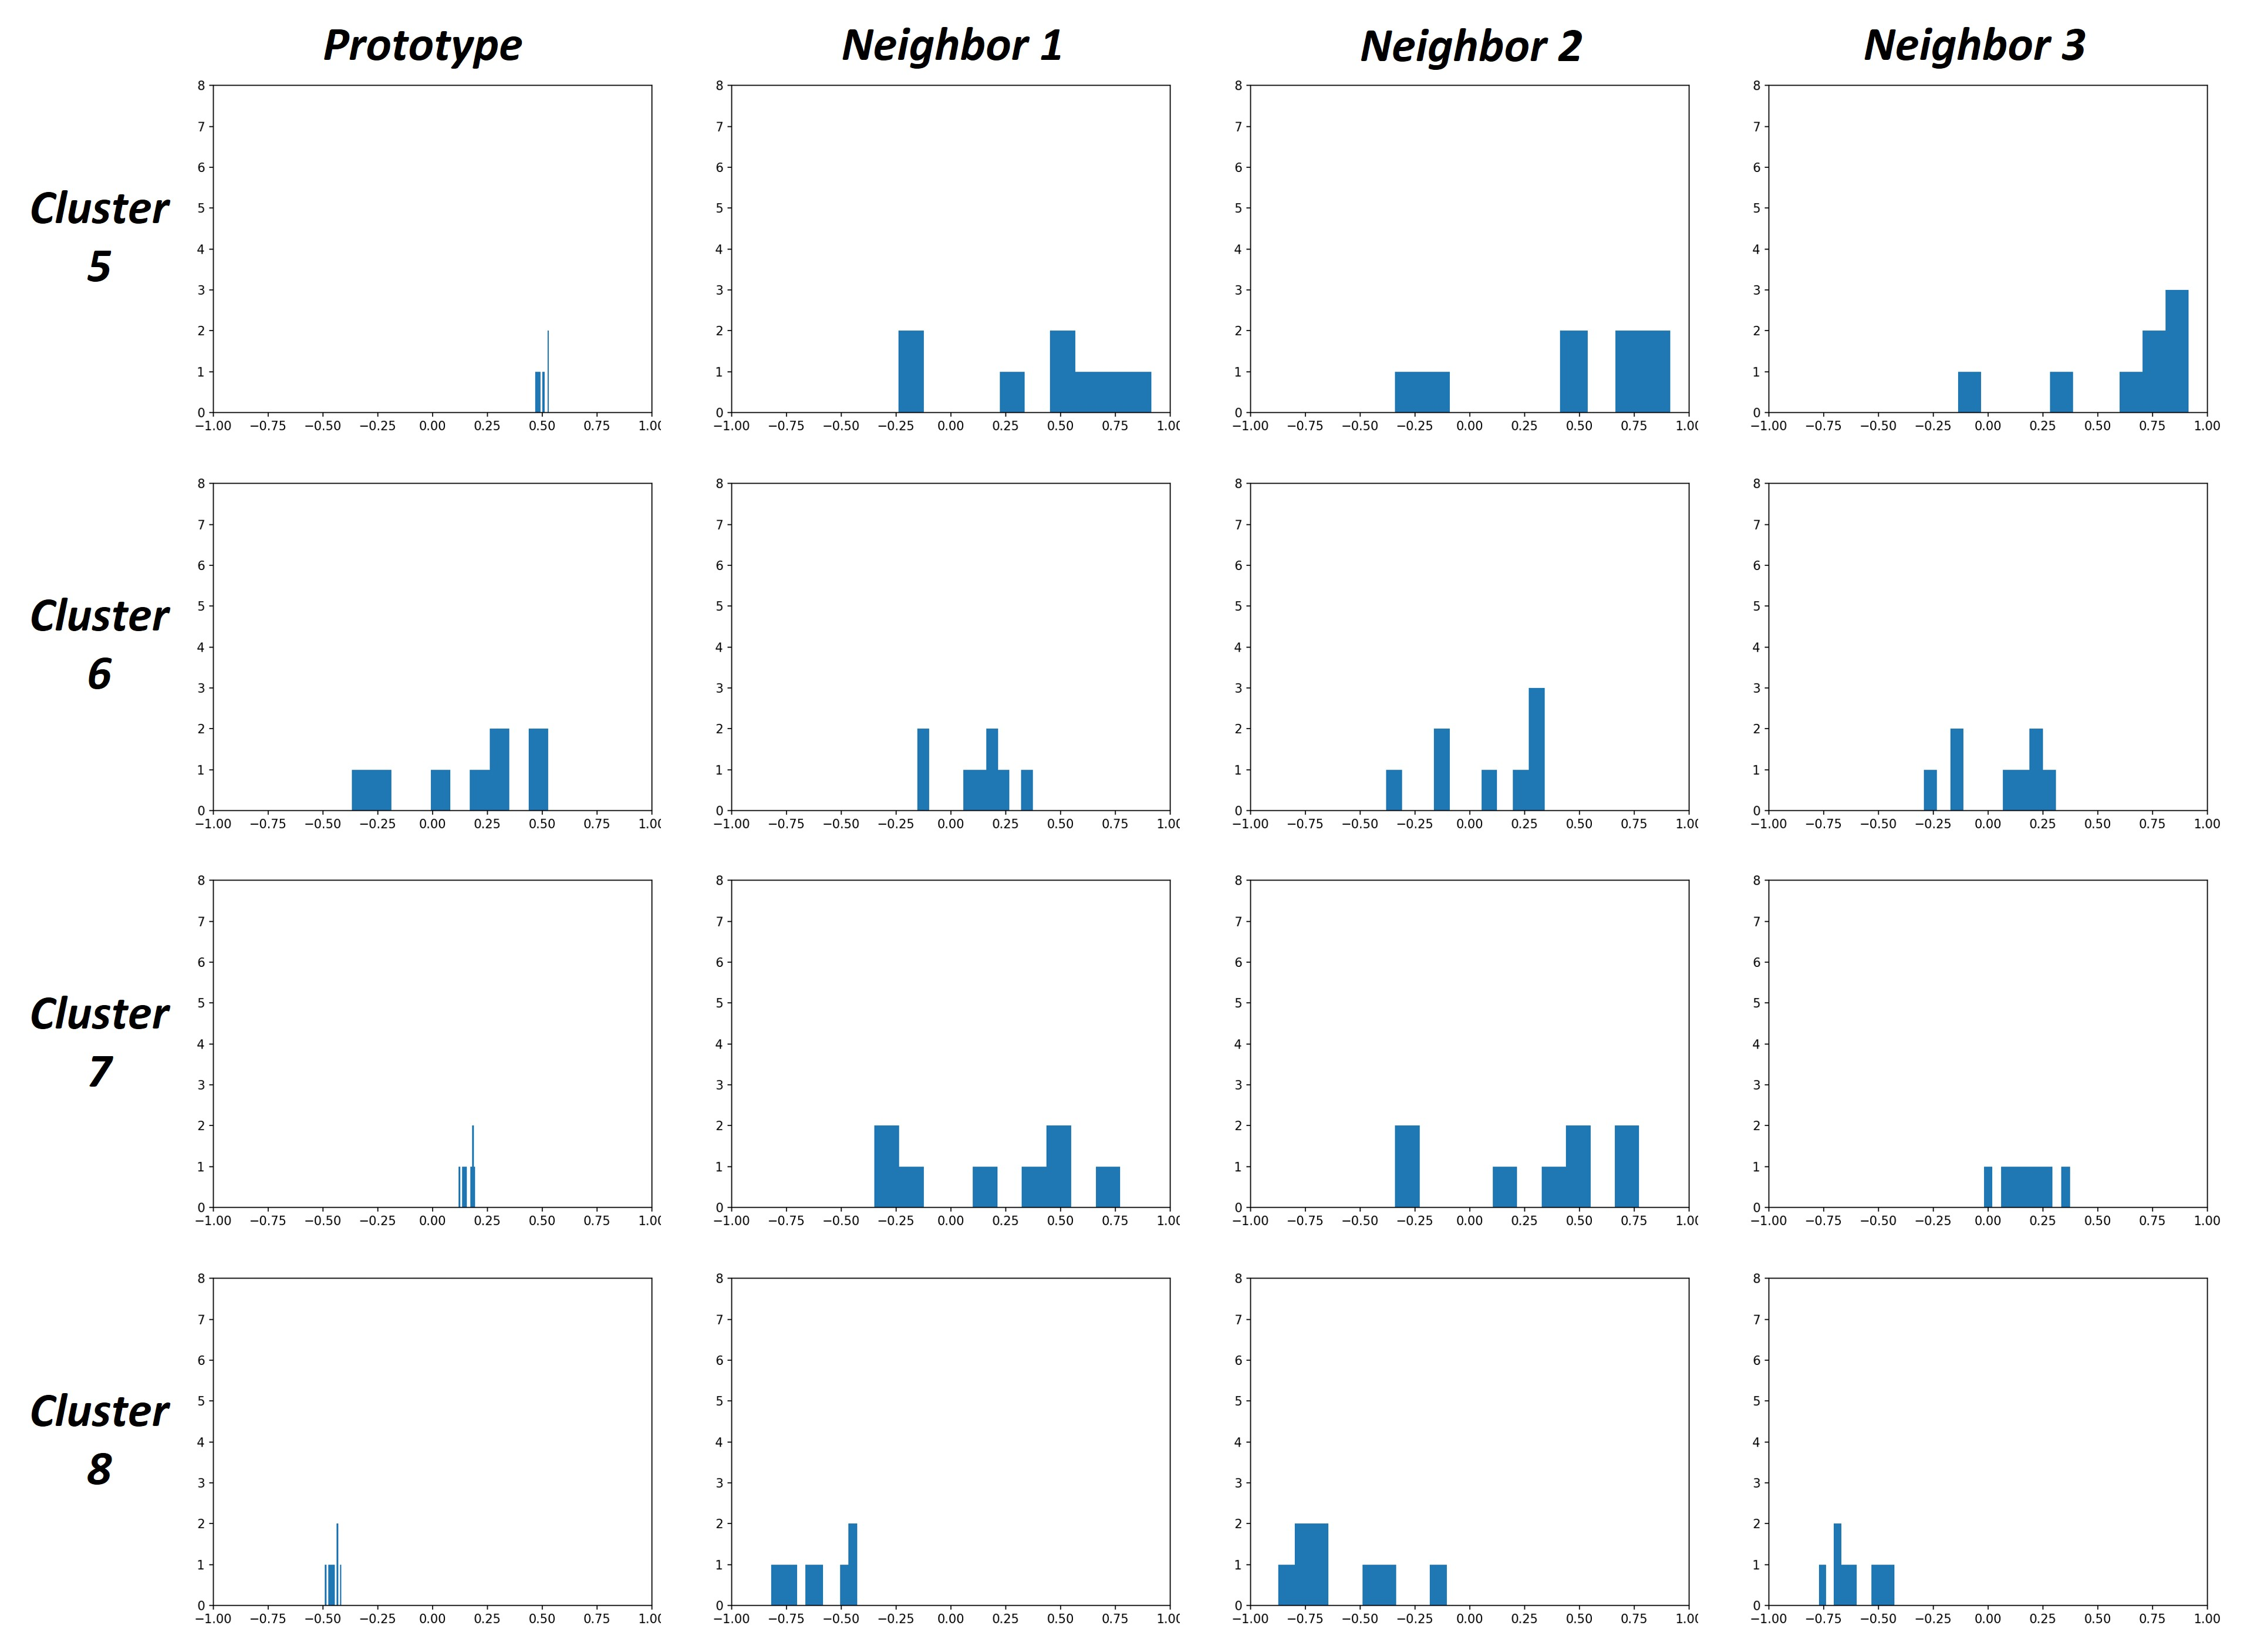}
\caption{Applying WHT to Figure~\ref{fig:slice2_l2_spatial}.}
\label{fig:slice2_map}
\end{figure*}

% slice 3
\begin{figure*}[h]
\centering
\includegraphics[scale=0.5]{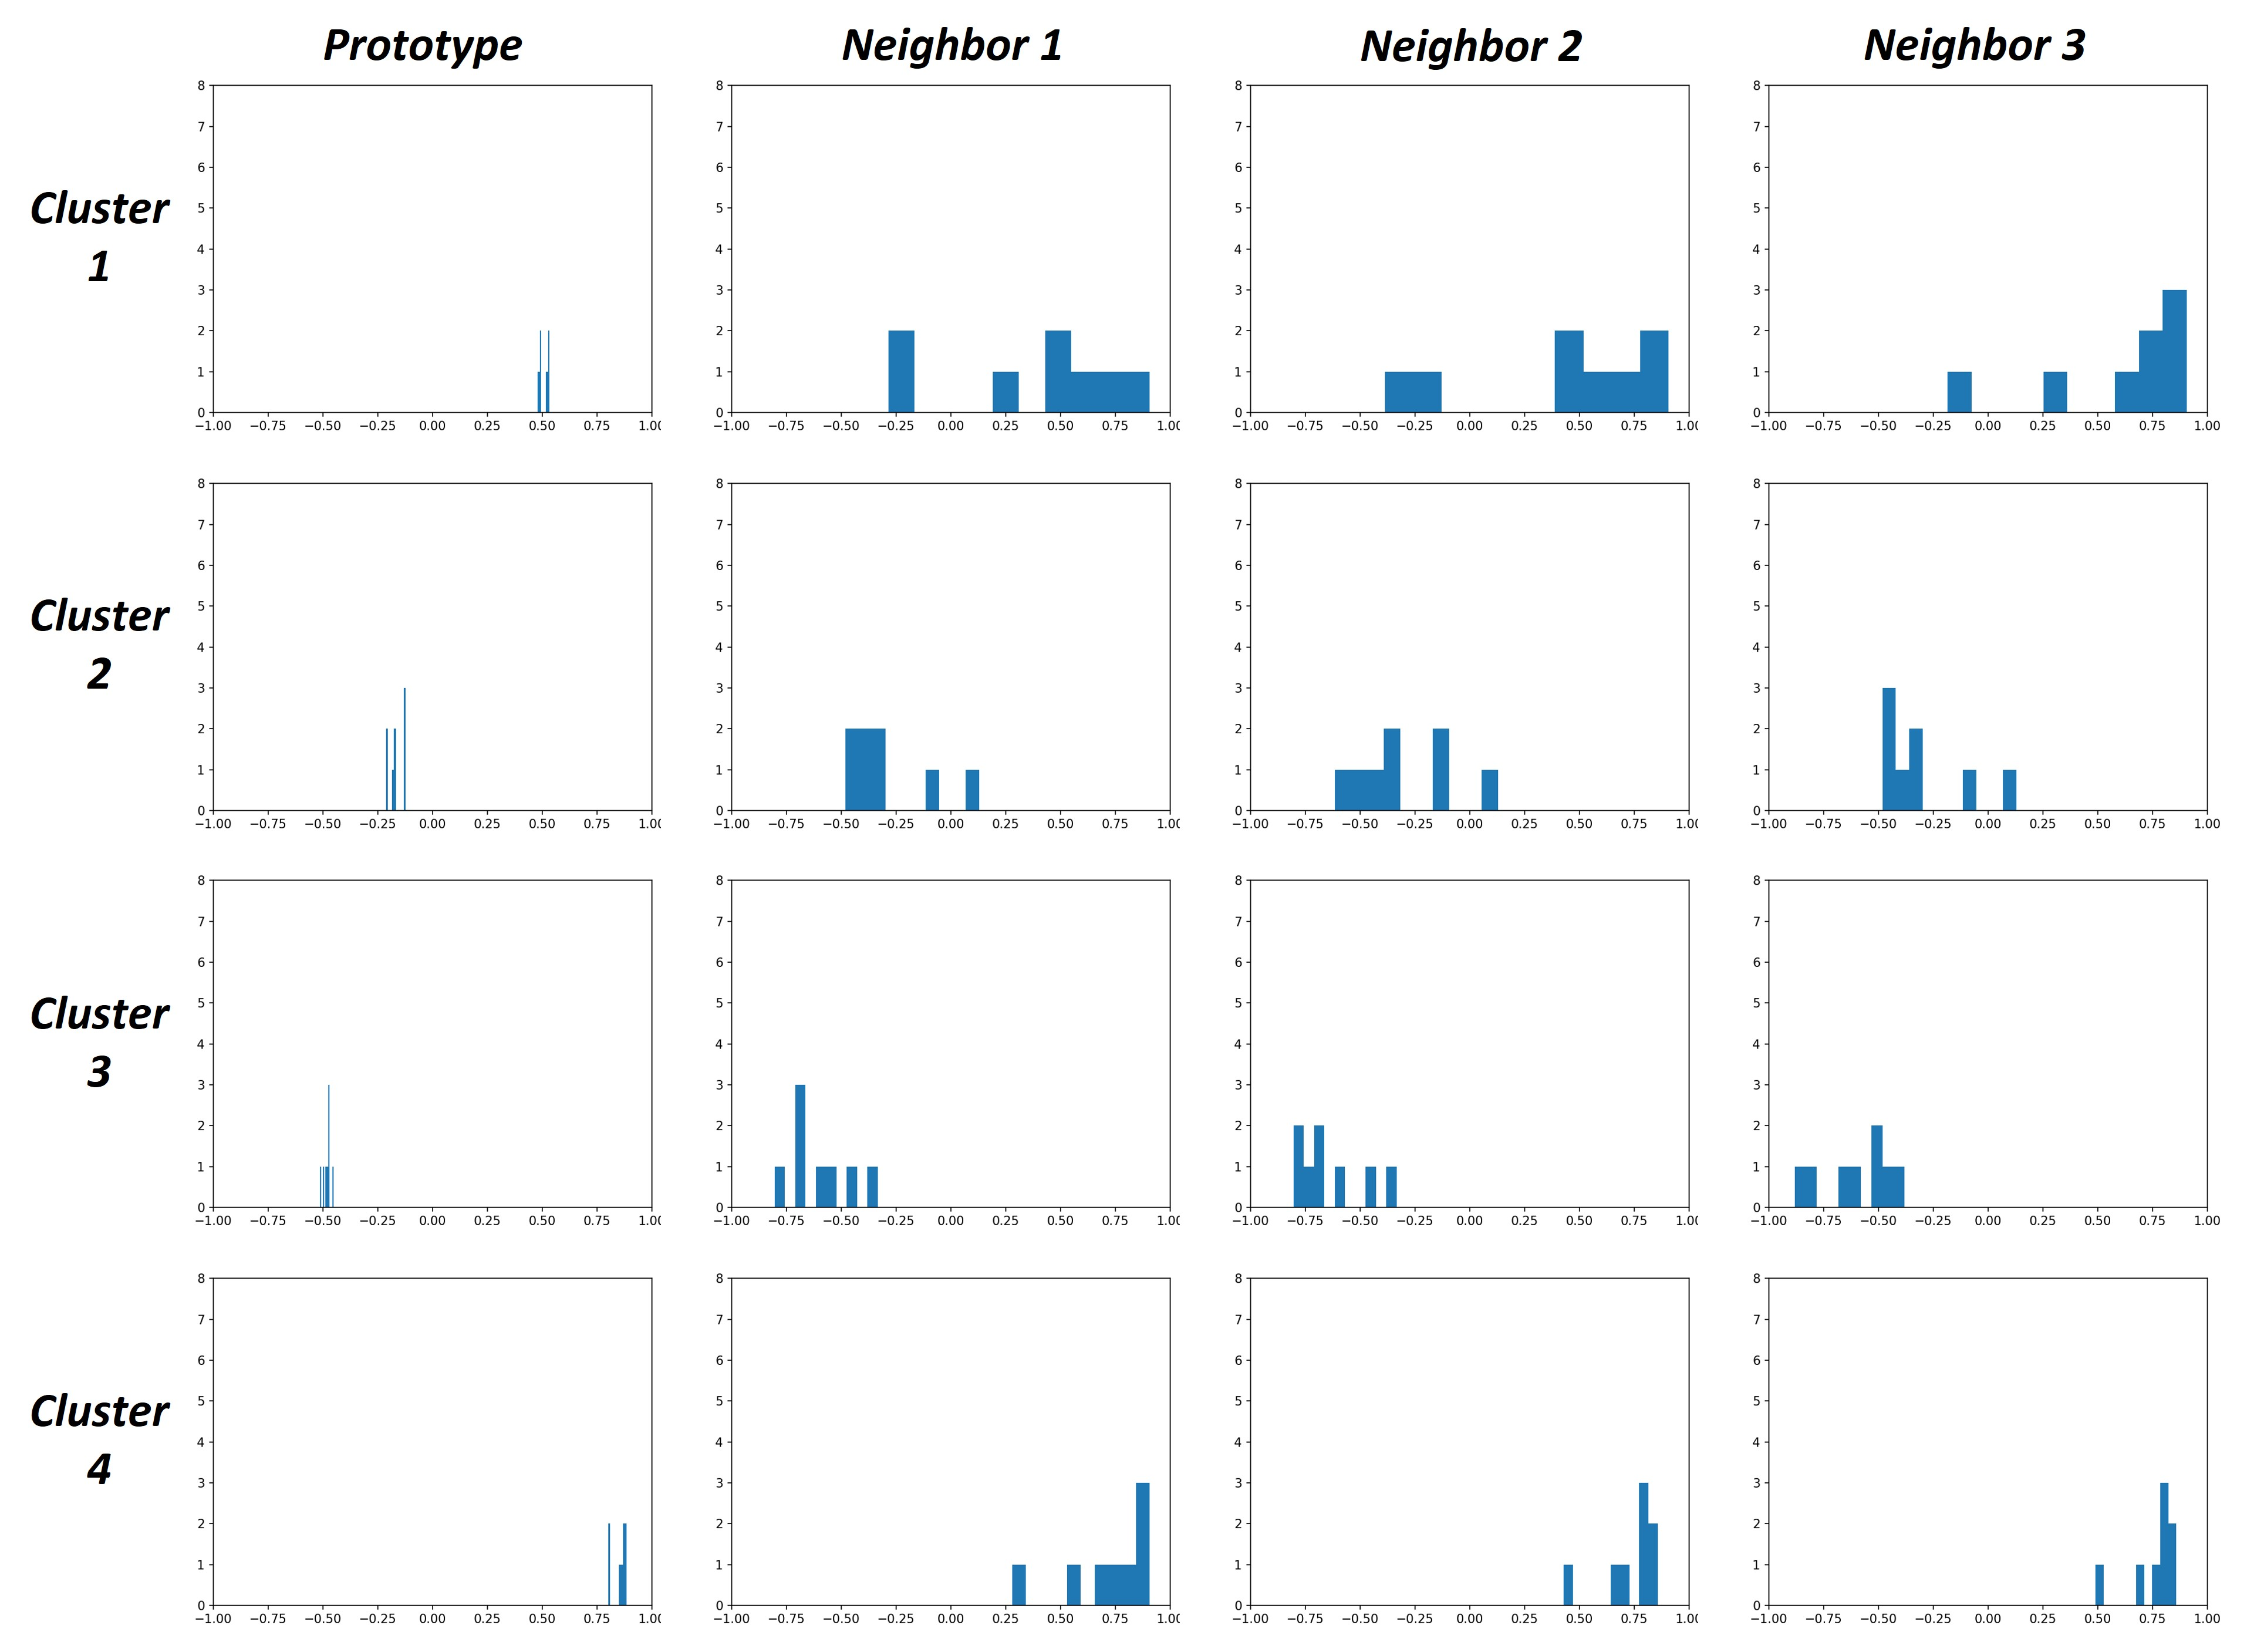}
\centering
\includegraphics[scale=0.5]{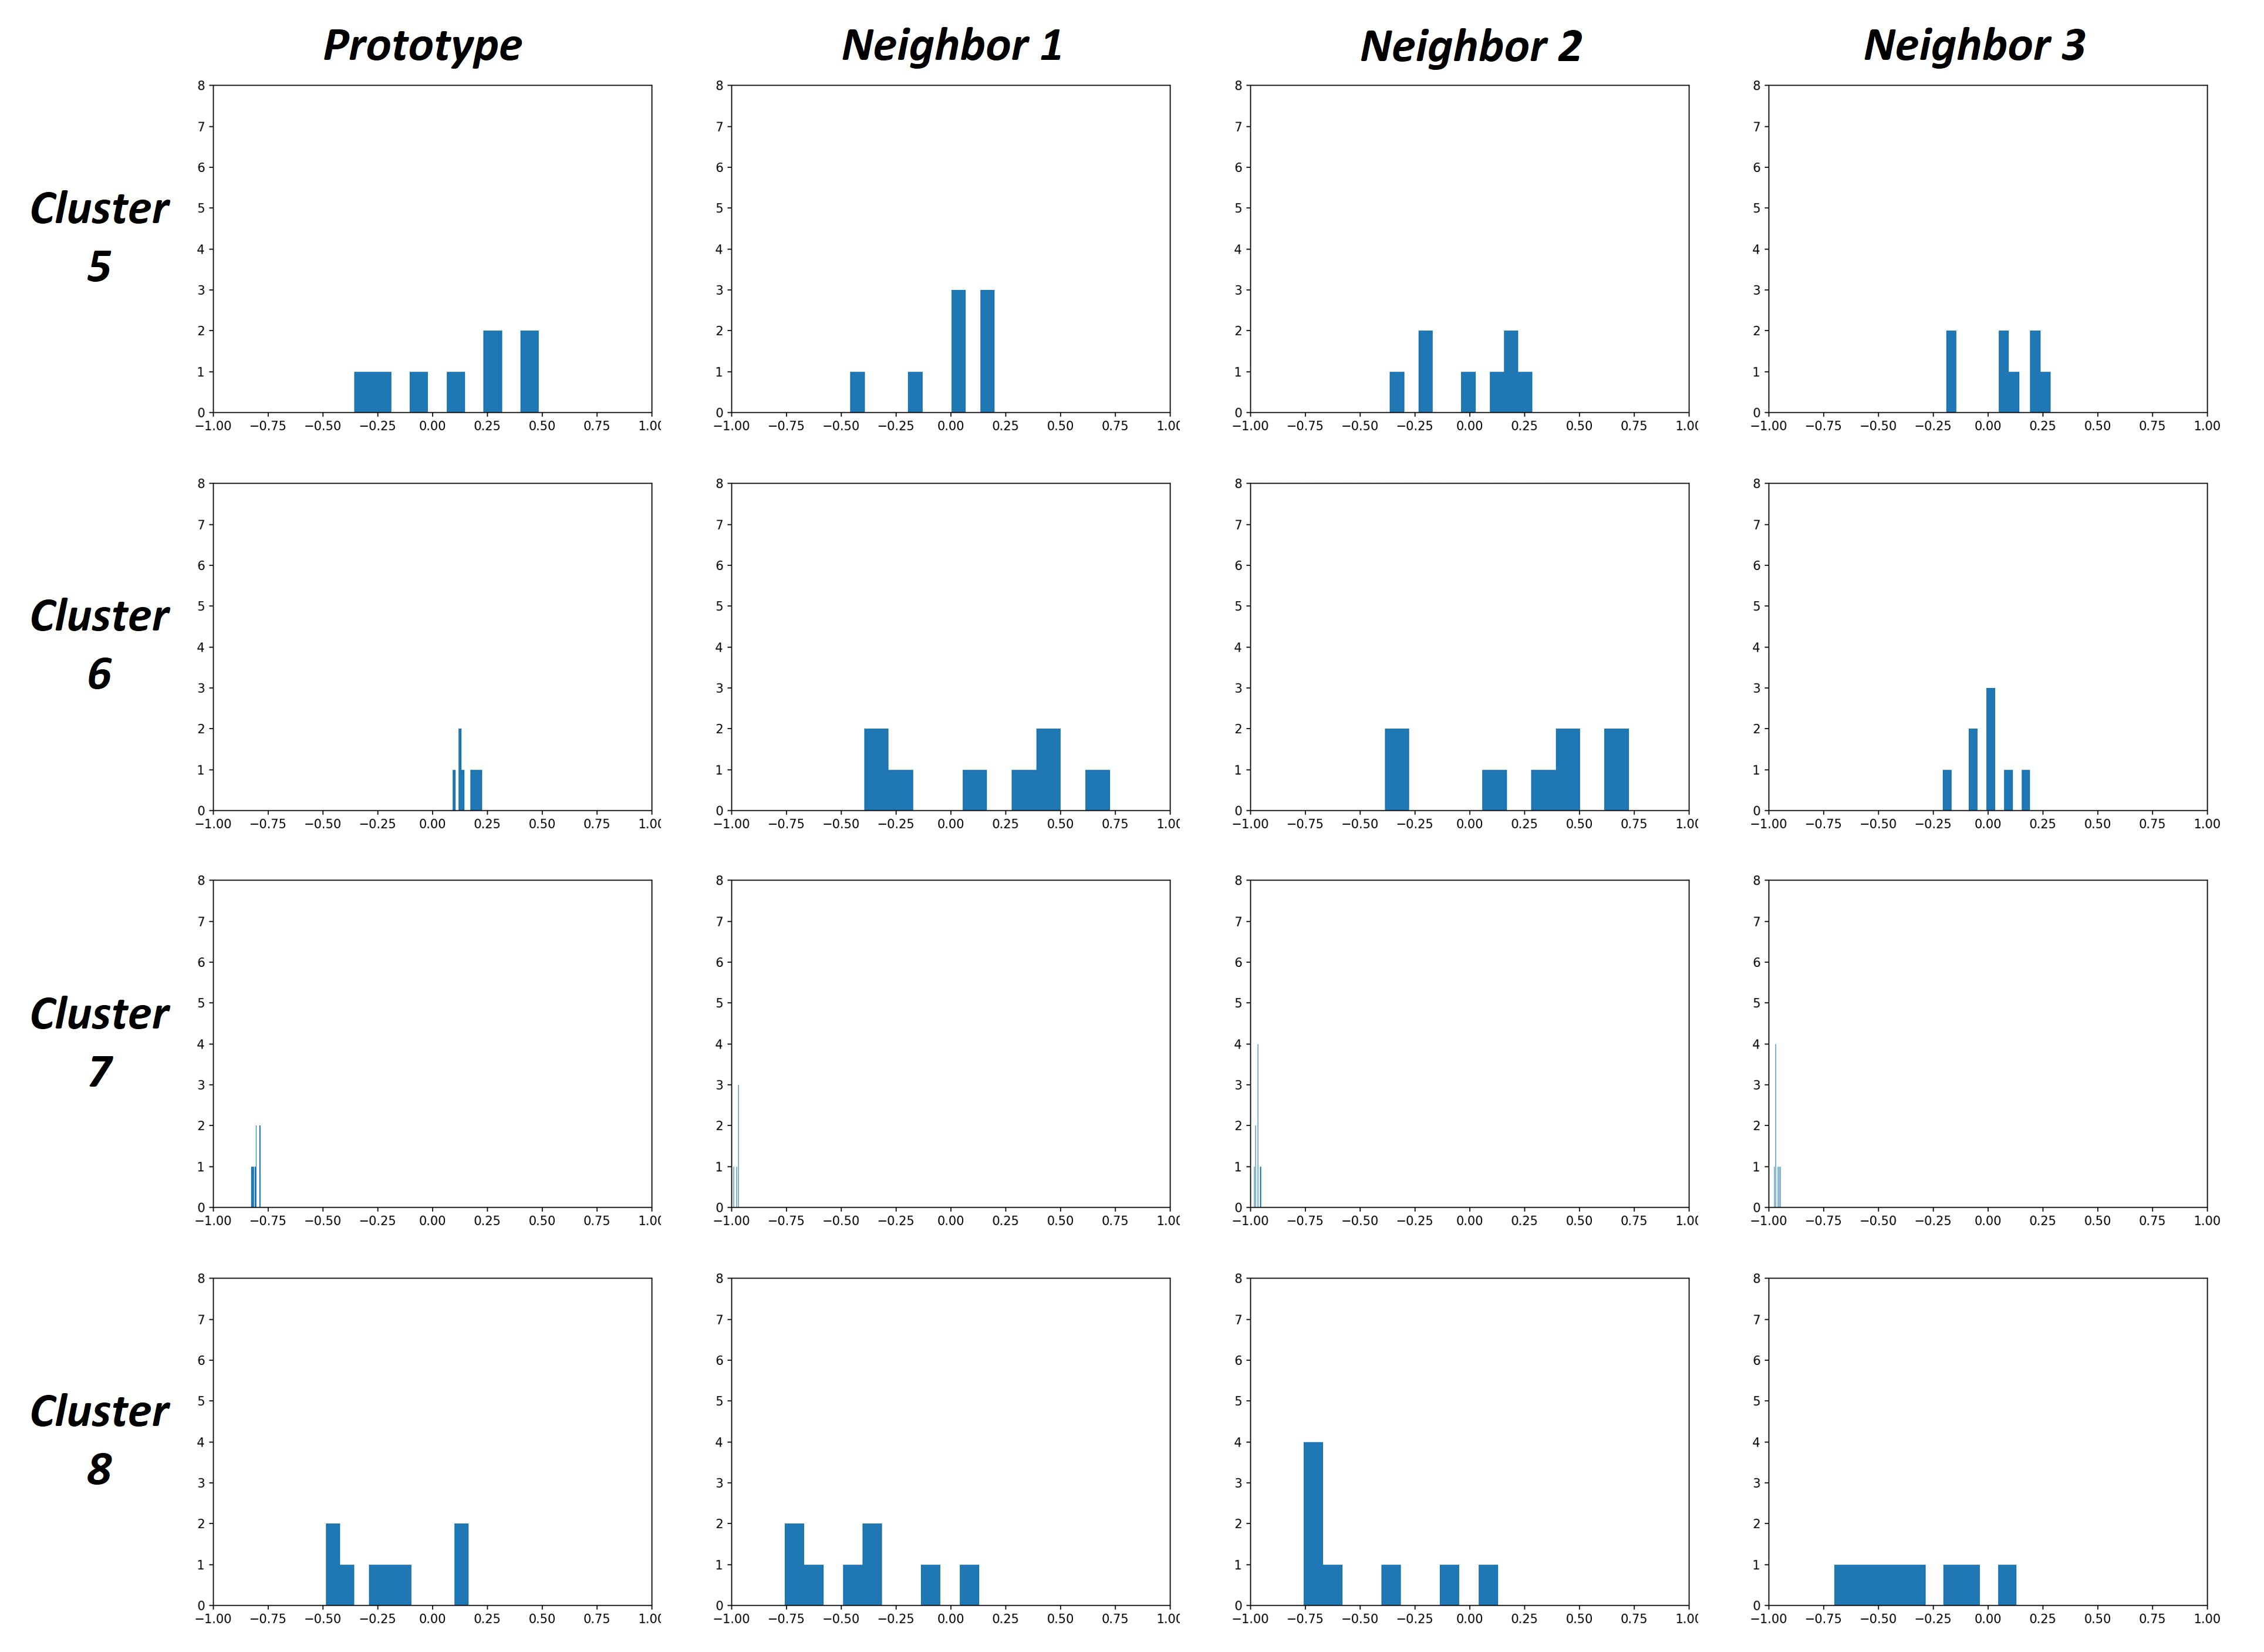}
\caption{Applying WHT to Figure~\ref{fig:slice3_l2_spatial}.}
\label{fig:slice3_map}
\end{figure*}


%%%%%% cosine & error %%%%%%
\section{Cosine Similarity Assignment}

{\color{red}{\textbf{Date: 2021.09.20 Monday}}}

%%%% part 1
%% cosine vs. l2
\textbf{Prototypes Assigned by Cosine Similarity}

Including comparing the prototype assignments results between using L2-norm and L1-norm, Table A and Table B display the comparing results of cosine similarity vs. L2-norm, and cosine similarity vs. L1-norm, respectively.

Remark:
\begin{enumerate}
\item Table~\ref{tab:cos_mismatching} vs. Table~\ref{tab:l1_mismatching}: Compared L2-norm prototype assignment results, L1-norm metric provides more similar outputs than cosine similarity.
\end{enumerate}

\setlength{\tabcolsep}{4.5mm}{
\begin{table*}[h]
\scriptsize
\centering
\begin{tabular}{ccccccccc}
\toprule
\#Clusters & 2 & 4 & 6 & 8 & 10 & 12 & 14 & 16 \\
\midrule
Slice 1 & $2.97\%$ & $44.28\%$ & $42.71\%$ & $48.78\%$ & $49.61\%$ & $50.53\%$ & $51.39\%$ & $51.91\%$ \\
Slice 2 & $2.83\%$ & $46.57\%$ & $48.74\%$ & $49.39\%$ & $50.94\%$ & $54.01\%$ & $54.11\%$ & $54.69\%$ \\
Slice 3 & $0.14\%$ & $44.49\%$ & $56.97\%$ & $51.06\%$ & $55.33\%$ & $53.82\%$ & $53.81\%$ & $54.91\%$ \\
\midrule
Avg. Mismatching Rate & $1.98\%$ & $45.11\%$ & $49.47\%$ & $49.74\%$ & $51.96\%$ & $52.79\%$ & $53.10\%$ & $53.84\%$ \\
\bottomrule
\end{tabular}
\caption{We compare the prototypes assigned by \textbf{cosine similarity} and \textbf{L2-norm}, respectively. The table shows the mismatching rates for samples in each slice (band) under different numbers of clusters when employing K-means to find the prototypes. The bottom row is the average mismatching rate under different cases.}
\label{tab:cos_mismatching}
\end{table*}}

%% cos vs. l1
\setlength{\tabcolsep}{4.5mm}{
\begin{table*}[h]
\scriptsize
\centering
\begin{tabular}{ccccccccc}
\toprule
\#Clusters & 2 & 4 & 6 & 8 & 10 & 12 & 14 & 16 \\
\midrule
Slice 1 & $3.04\%$ & $73.29\%$ & $41.11\%$ & $48.47\%$ & $48.74\%$ & $49.77\%$ & $51.90\%$ & $51.84\%$ \\
Slice 2 & $2.86\%$ & $46.39\%$ & $48.38\%$ & $49.88\%$ & $50.43\%$ & $53.32\%$ & $54.13\%$ & $55.00\%$ \\
Slice 3 & $99.37\%$ & $44.32\%$ & $56.23\%$ & $50.98\%$ & $54.71\%$ & $53.30\%$ & $53.74\%$ & $54.84\%$ \\
\midrule
Avg. Mismatching Rate & $35.09\%$ & $54.67\%$ & $48.57\%$ & $49.77\%$ & $51.30\%$ & $52.04\%$ & $52.99\%$ & $53.90\%$ \\
\bottomrule
\end{tabular}
\caption{We compare the prototypes assigned by \textbf{cosine similarity} and \textbf{L1-norm}, respectively. The table shows the mismatching rates for samples in each slice (band) under different numbers of clusters when employing K-means to find the prototypes. The bottom row is the average mismatching rate under different cases.}
\label{tab:l1_cos_mismatching}
\end{table*}}

%%%% Modified LeNet %%%%
\section{DPQ Reproduction on LeNet in DeBut}

\textbf{\color{red}{Date: 2021.09.21 Tuesday}}

The structure of LeNet we employed is shown in Table~\ref{tab:DeBut_lenet}. The experiments are handled by Jie.

\setlength{\tabcolsep}{1mm}{
\begin{table}[h]
\scriptsize
\centering
\begin{tabular}{llcllcl}
\toprule
\multirow{2}{*}{LeNet} & Input & ~ & \multicolumn{2}{c}{Weight} & ~ & Output \\
\cline{2-2}
\cline{4-5}
\cline{7-7}
~ & $[c_i, H_i, W_i]$ & ~ & $[c_i, c_o, k, k]$ & $[c_o, k^2\cdot c_i]$ & ~ & $[c_o, H_o, W_o]$\\
\midrule
CONV1 & $[1, 28, 28]$ & ~ & $[1, 8, 3, 3]$ & $[8, 9]$ & ~ & $[8, 26, 26]$\\
ReLU1 & $[8, 26, 26]$ & ~ & $-$ & $-$ & ~ & $[8, 26, 26]$\\
MaxPooling1 & $[8, 26, 26]$ & ~ & $-$ & $-$ & ~ & $[8, 13, 13]$\\
\midrule
CONV2 & $[8, 13, 13]$ & ~ & $[8, 16, 3, 3]$ & $[16, 72]$ & ~ & $[16, 11, 11]$\\
ReLU2 & $[16, 11, 11]$ & ~ & $-$ & $-$ & ~ & $[16, 11, 11]$\\
MaxPooling2 & $[16, 11, 11]$ & ~ & $-$ & $-$ & ~ & $[16, 5, 5]$\\
\midrule
FC1 & $[16, 5, 5]$ & ~ & $[16, 128, 5, 5]$ & $[128, 400]$ & ~ & $[128, 1, 1]$ \\
ReLU3 & $[128, 1, 1]$ & ~ & $-$ & $-$ & ~ & $[128, 1, 1]$ \\
\midrule
FC2 & $[128, 1, 1]$ & ~ & $[128, 64, 1, 1]$ & $[64, 128]$ & ~ & $[64, 1, 1]$ \\
\midrule
FC3 & $[64, 1, 1]$ & ~ & $[64, 10, 1, 1]$ & $[10, 64]$ & ~ & $[10, 1, 1]$ \\

\midrule
\end{tabular}
\caption{Complete structure of LeNet used in DeBut.}
\label{tab:DeBut_lenet}
\end{table}}

%%%%% softmax vs. l1-norm in the spation and spectral domain
\section{Softmax vs. L1-Norm Assignment}

\textcolor{red}{\textbf{Date: 2021.09.28 Tuesday}}

We compare three different ways, namely, softmax in DPQ, L1-Norm in the spatial domain, and L1-Norm in the spectral domain, to assign prototypes as shown in Figure~\ref{fig:mapping}. The experiment aims to verify whether L1-Norm based assignment can have similar results compared with the softmax way. The detailed steps are displayed below:
\begin{enumerate}
\item Select a pretrained neural network, then extract the flattened input by $\rm{im2col}$ operation and the corresponding prototypes.
\item Choose several $p$ shown in Figure~\ref{fig:mapping}, employing different assignment metrics to compare the distances between $p$ and the available prototypes.
\item Compare the bar charts which represent the distance under different metrics. 
\end{enumerate}

\textbf{Remarks:}
\begin{enumerate}
\item Softmax vs. l1-norm: the assignments are always different (10 / 10).
\item L1-norm in the spatial domain vs. L1-norm in the spectral domain: the assignments are usually consistent (7 / 10).
\end{enumerate}

\begin{figure*}[h]
\centering
\includegraphics[scale=.34]{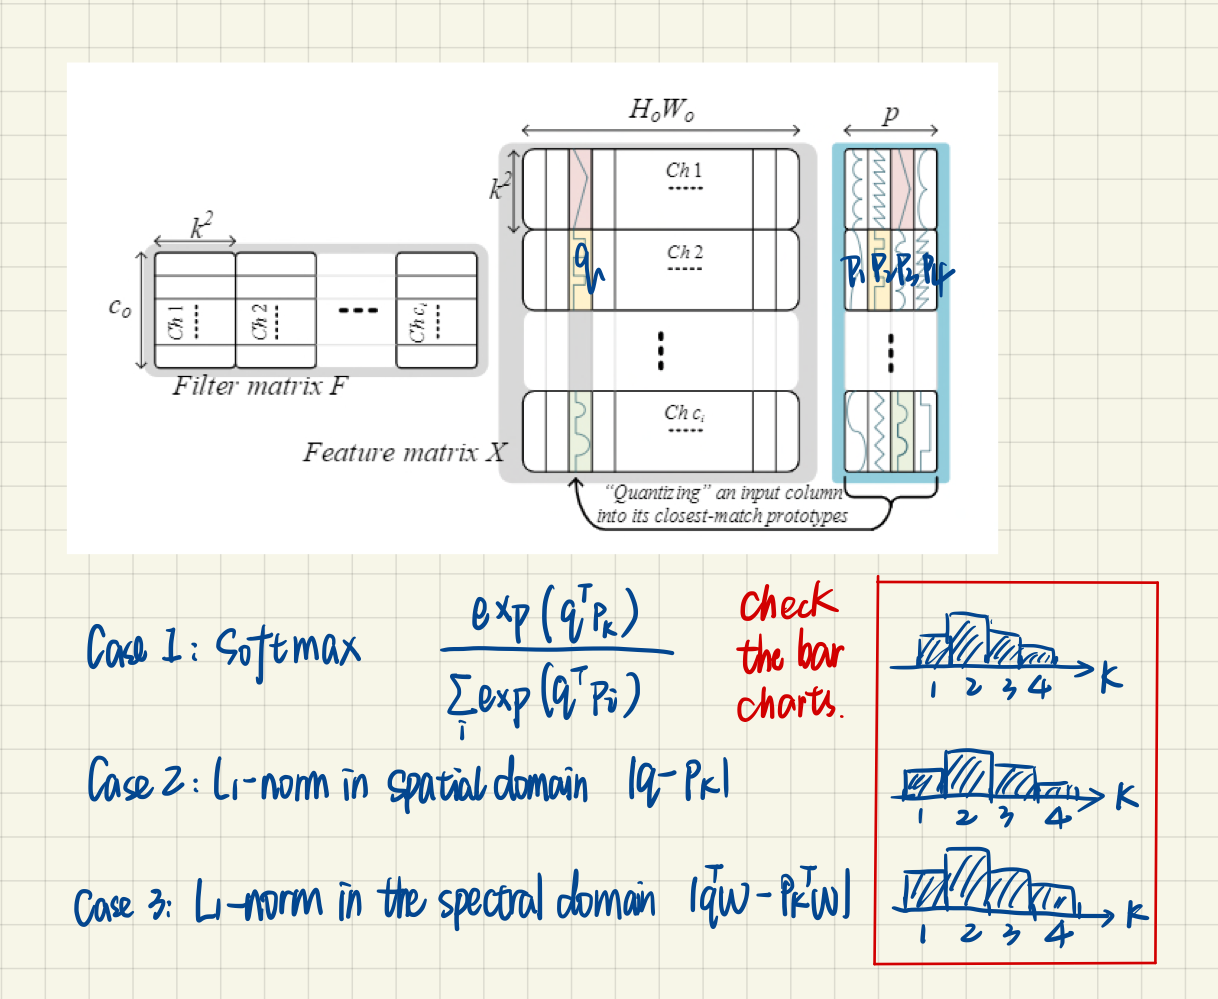}
\caption{The mapping of input data columns onto prototype subvectors in a CNN layer under the im2col setting.}
\label{fig:mapping}
\end{figure*}

%% 1
\begin{figure*}
\centering
\includegraphics[scale=1]{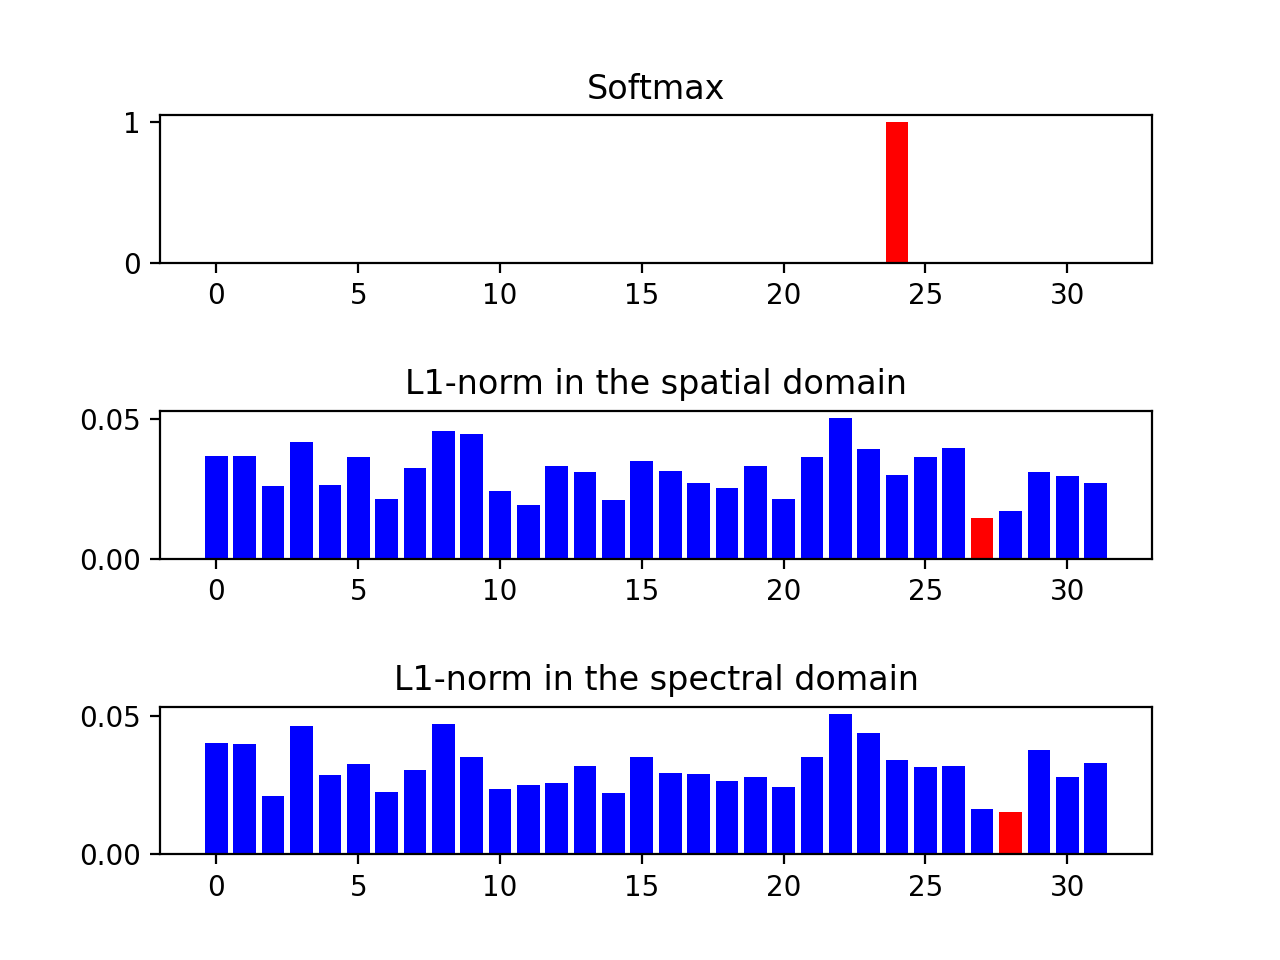}
\caption{Prototype assignments for a fixed vector under different metric.}
\label{fig:soft_l1_1}
\end{figure*}
%% 2
\begin{figure*}
\centering
\includegraphics[scale=1]{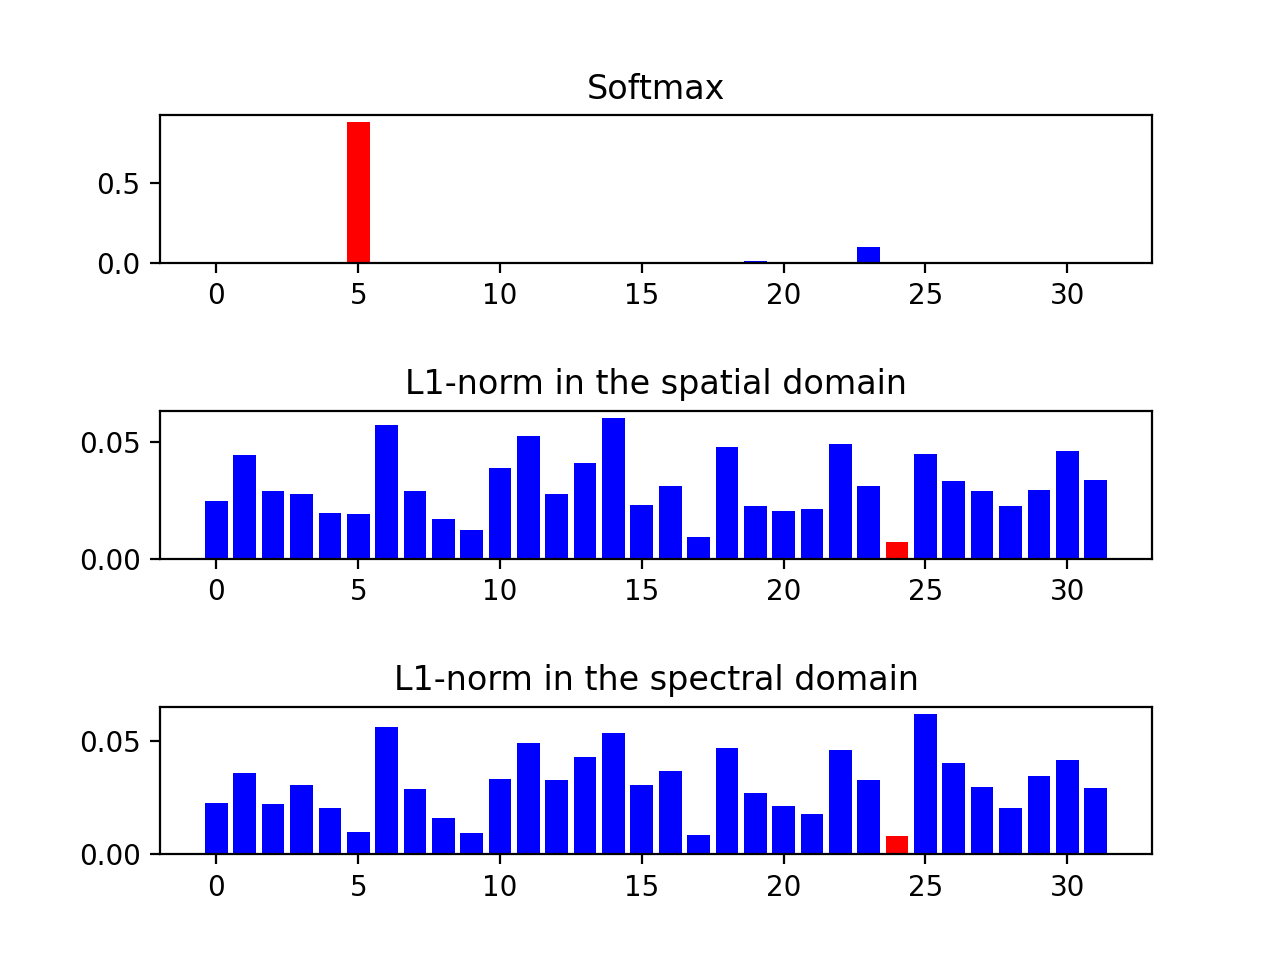}
\caption{Prototype assignments for a fixed vector under different metric.}
\label{fig:soft_l1_2}
\end{figure*}
%% 3
\begin{figure*}
\centering
\includegraphics[scale=1]{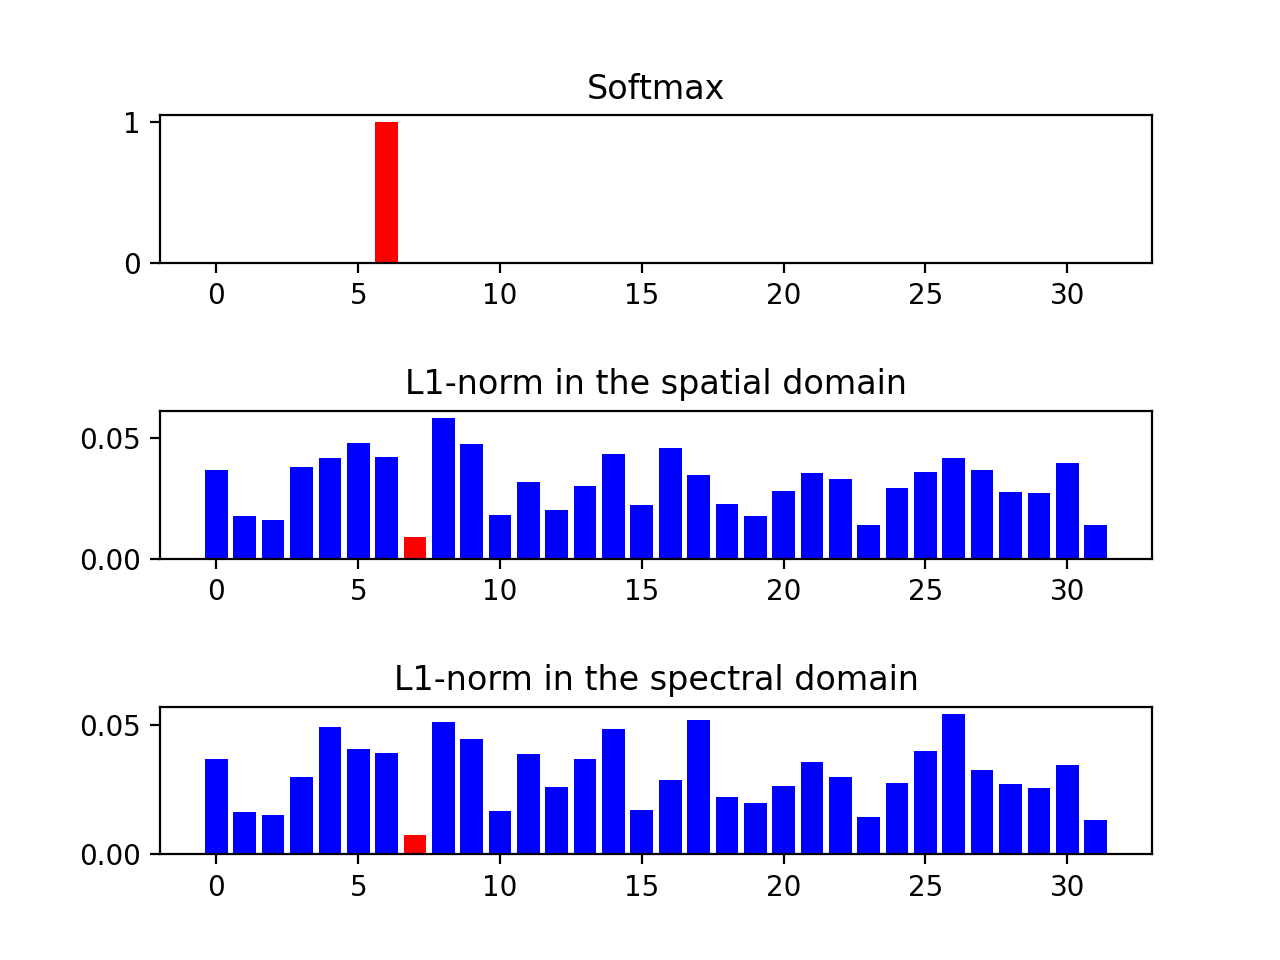}
\caption{Prototype assignments for a fixed vector under different metric.}
\label{fig:soft_l1_3}
\end{figure*}
%% 4
\begin{figure*}
\centering
\includegraphics[scale=1]{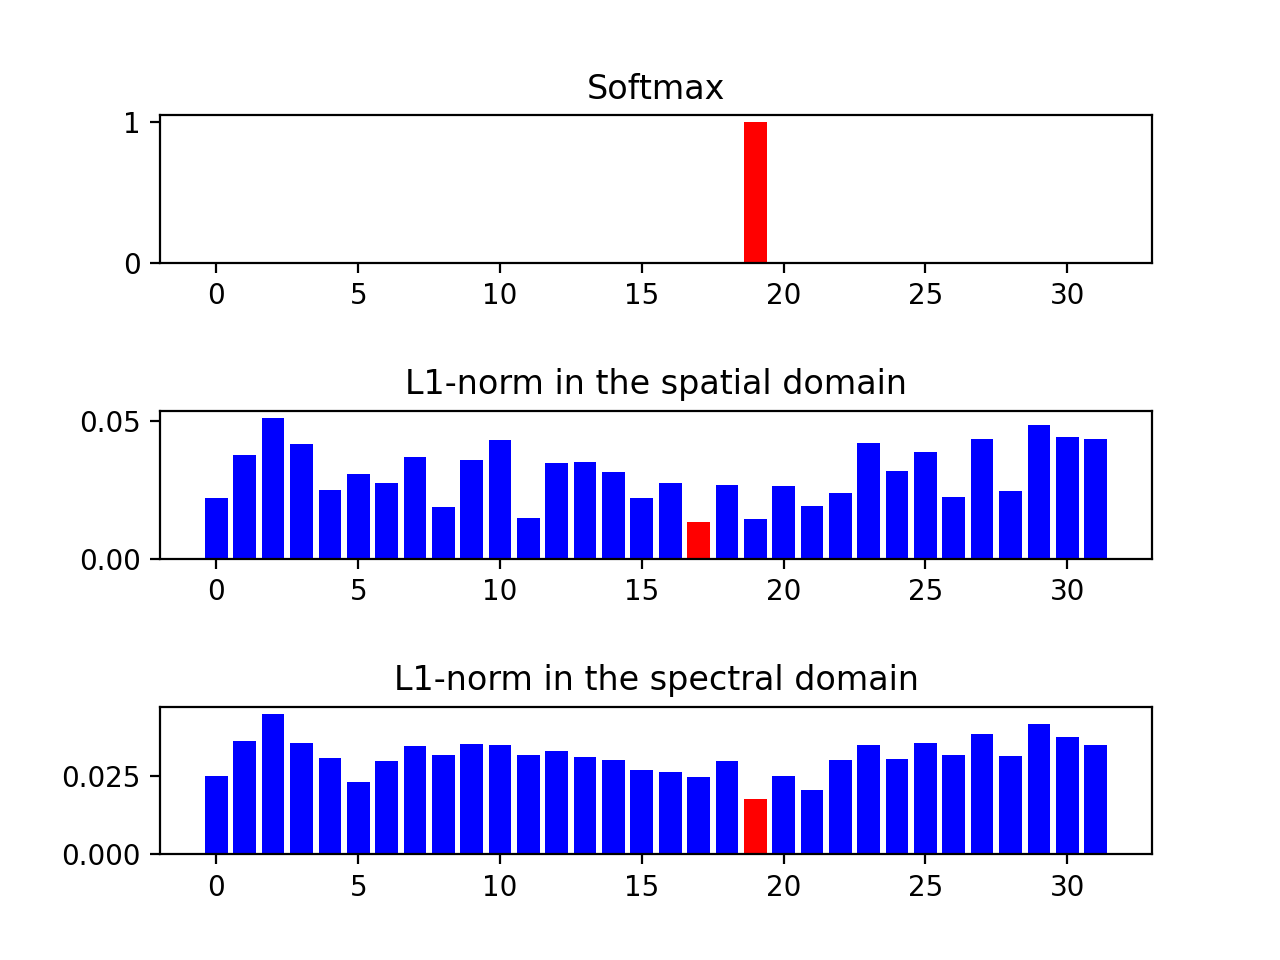}
\caption{Prototype assignments for a fixed vector under different metric.}
\label{fig:soft_l1_4}
\end{figure*}
%% 5
\begin{figure*}
\centering
\includegraphics[scale=1]{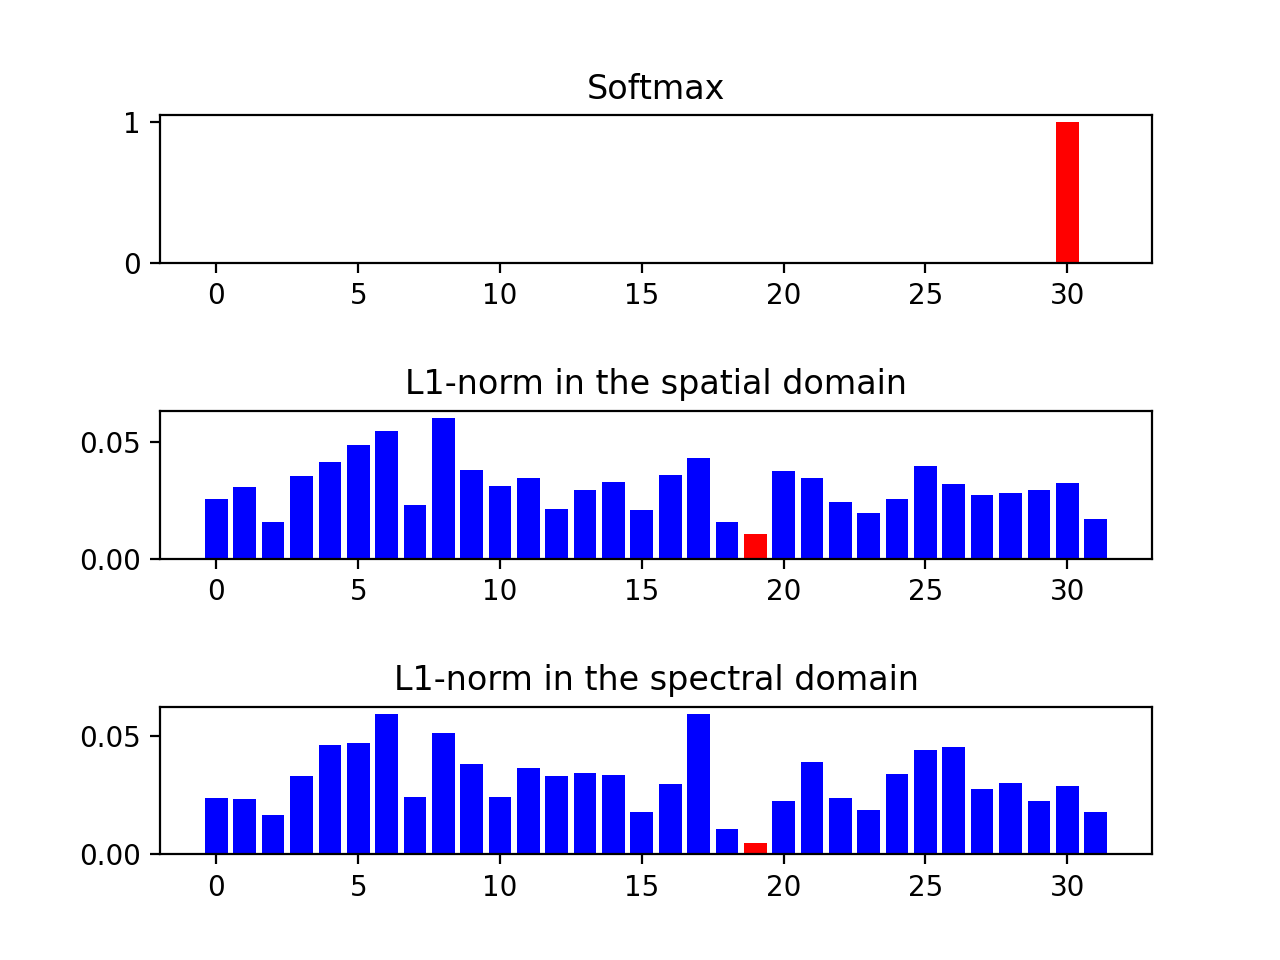}
\caption{Prototype assignments for a fixed vector under different metric.}
\label{fig:soft_l1_5}
\end{figure*}
%% 6
\begin{figure*}
\centering
\includegraphics[scale=1]{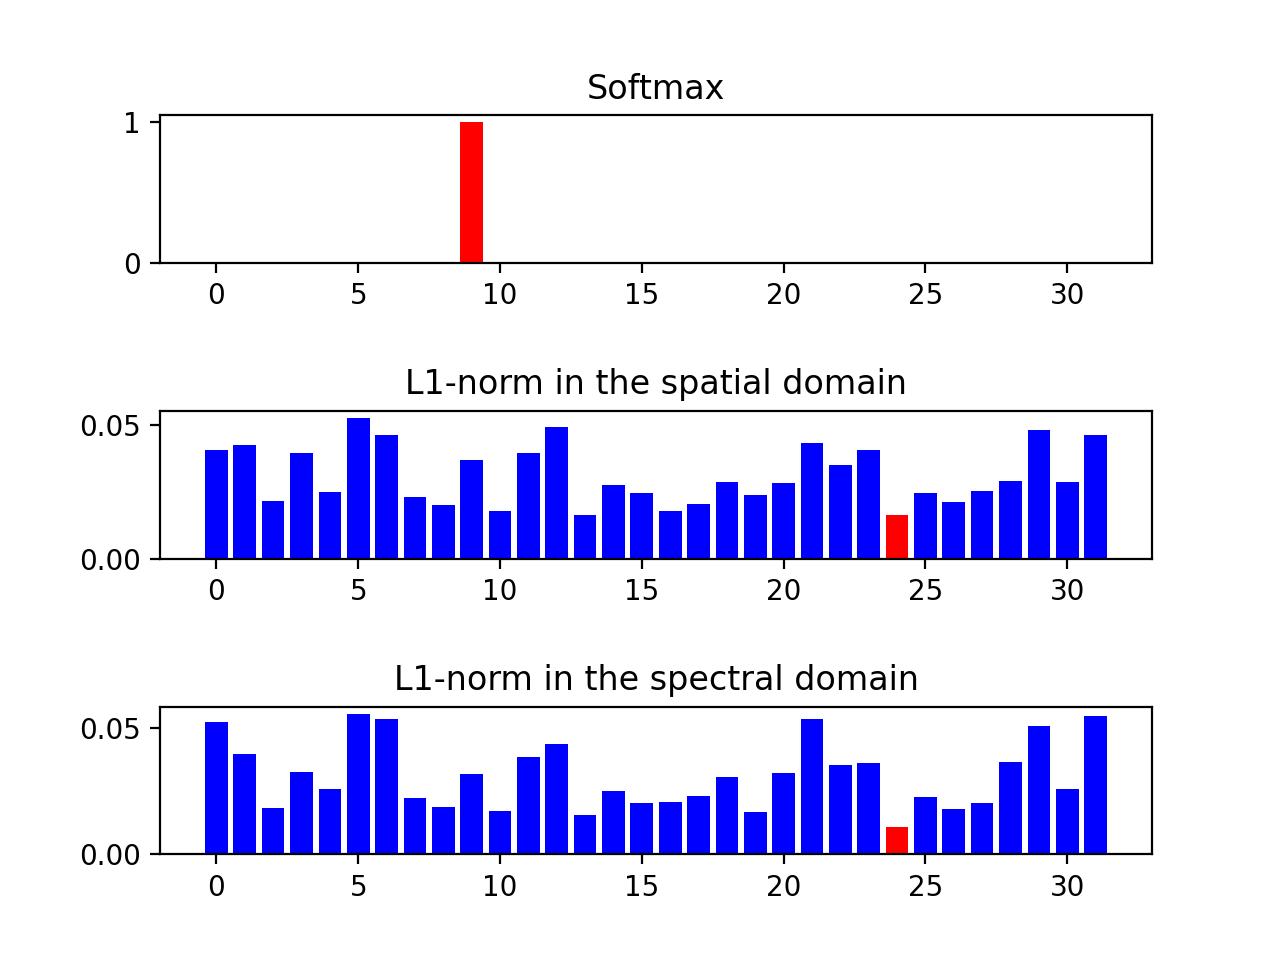}
\caption{Prototype assignments for a fixed vector under different metric.}
\label{fig:soft_l1_6}
\end{figure*}
%% 7
\begin{figure*}
\centering
\includegraphics[scale=1]{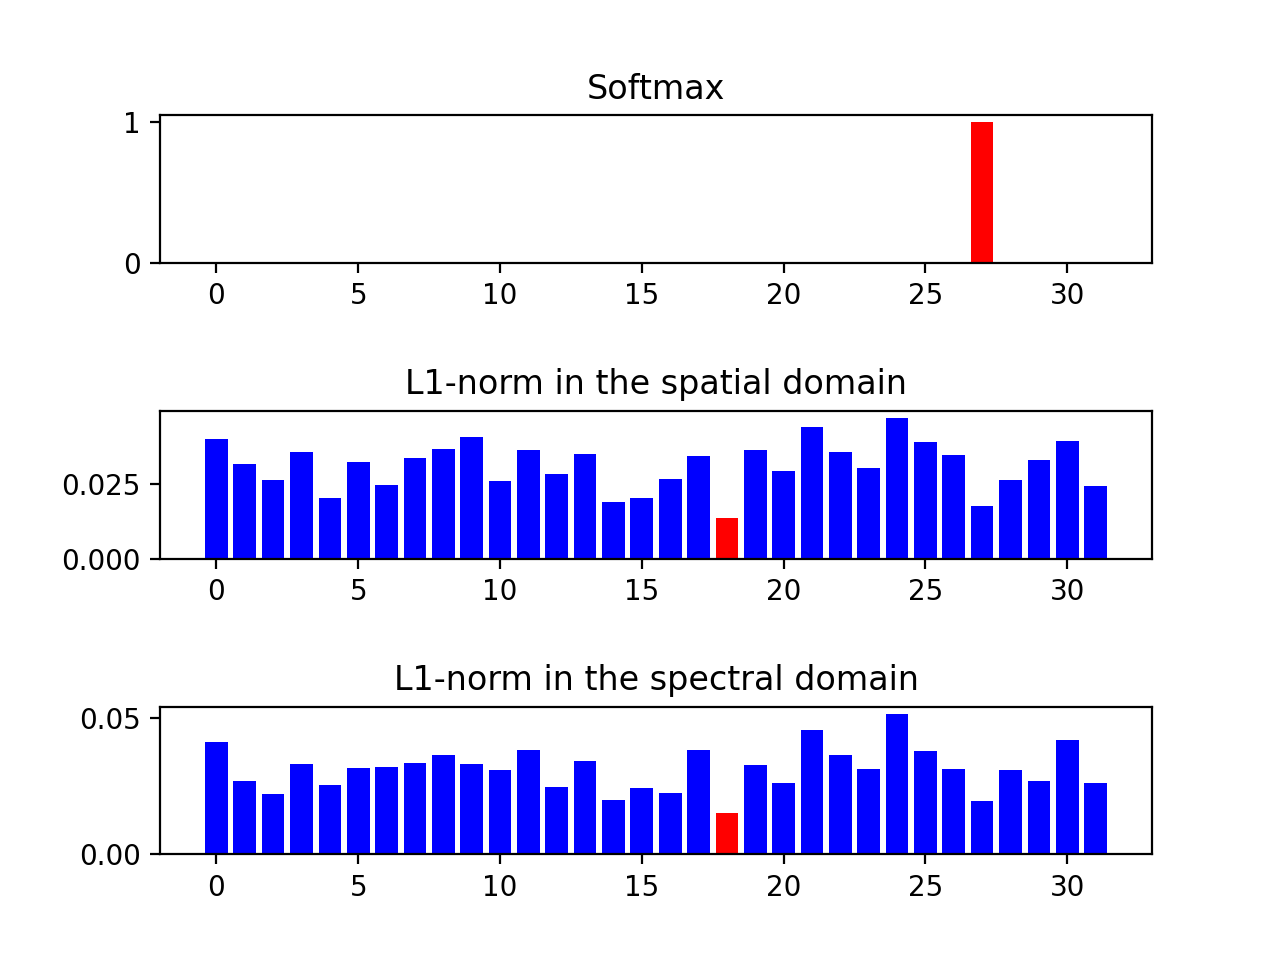}
\caption{Prototype assignments for a fixed vector under different metric.}
\label{fig:soft_l1_7}
\end{figure*}
%% 8
\begin{figure*}
\centering
\includegraphics[scale=1]{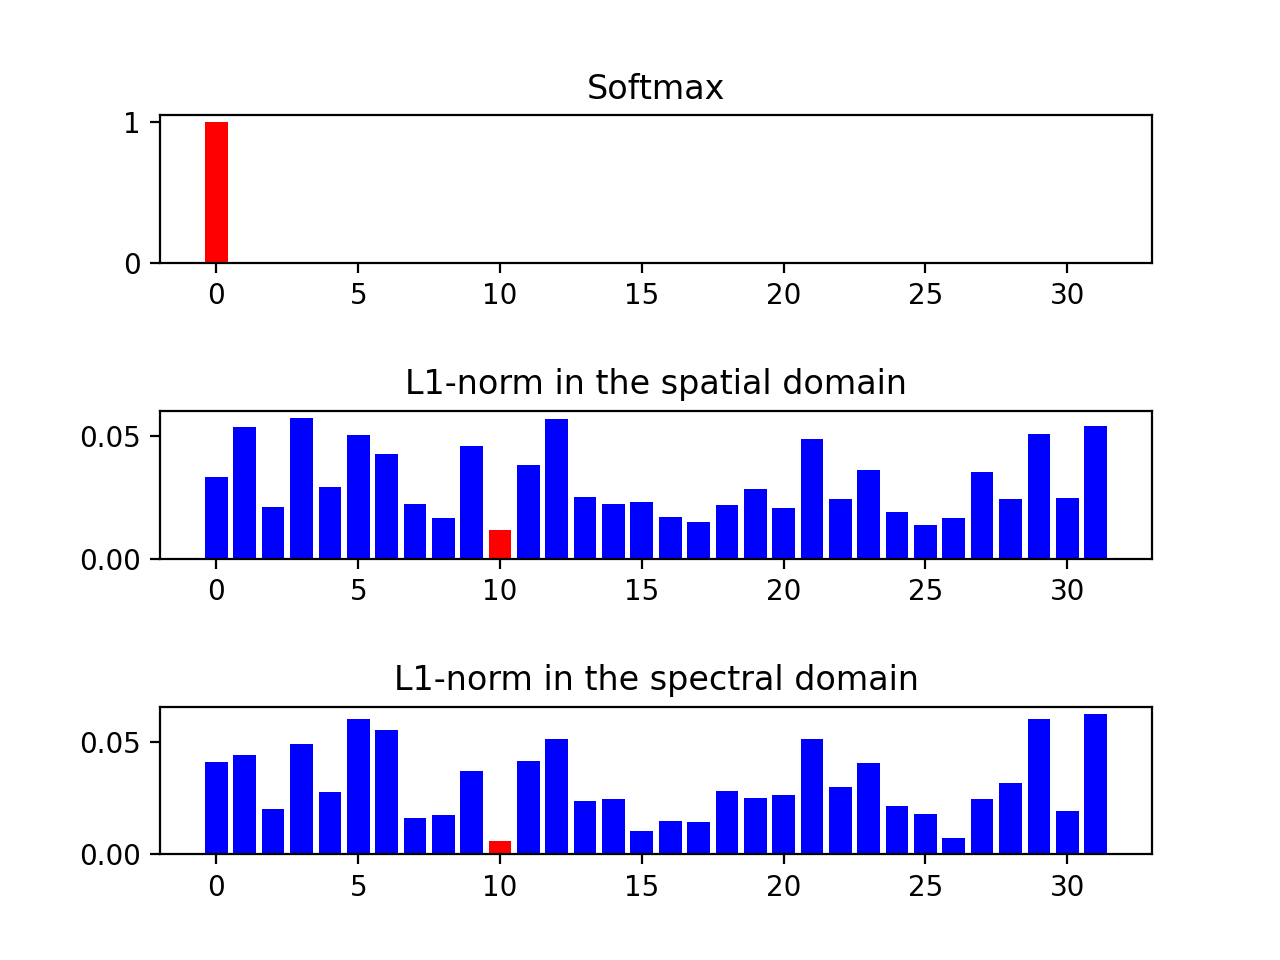}
\caption{Prototype assignments for a fixed vector under different metric.}
\label{fig:soft_l1_8}
\end{figure*}
%% 9
\begin{figure*}
\centering
\includegraphics[scale=1]{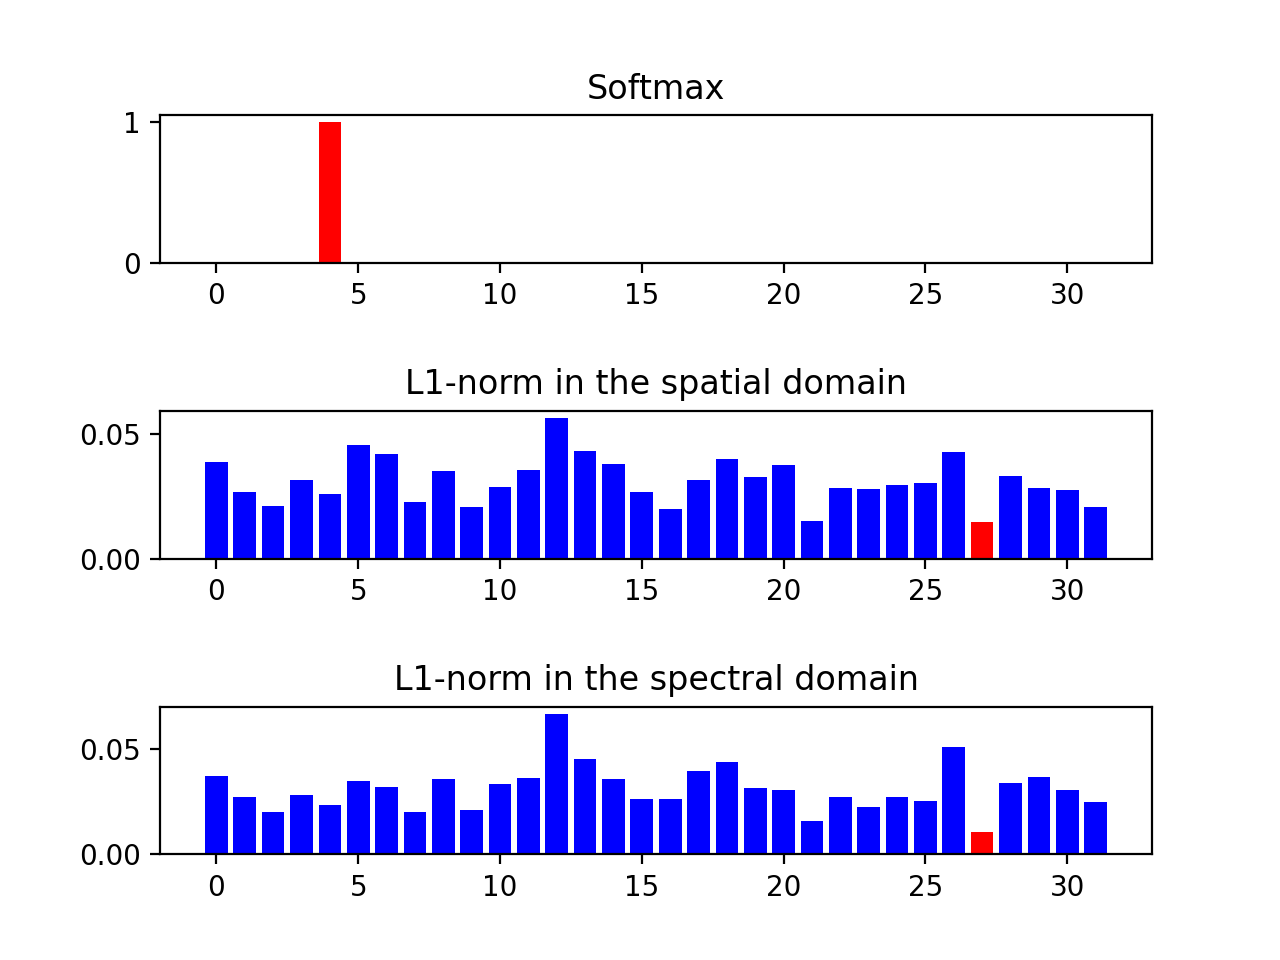}
\caption{Prototype assignments for a fixed vector under different metric.}
\label{fig:soft_l1_9}
\end{figure*}
%% 10
\begin{figure*}
\centering
\includegraphics[scale=1]{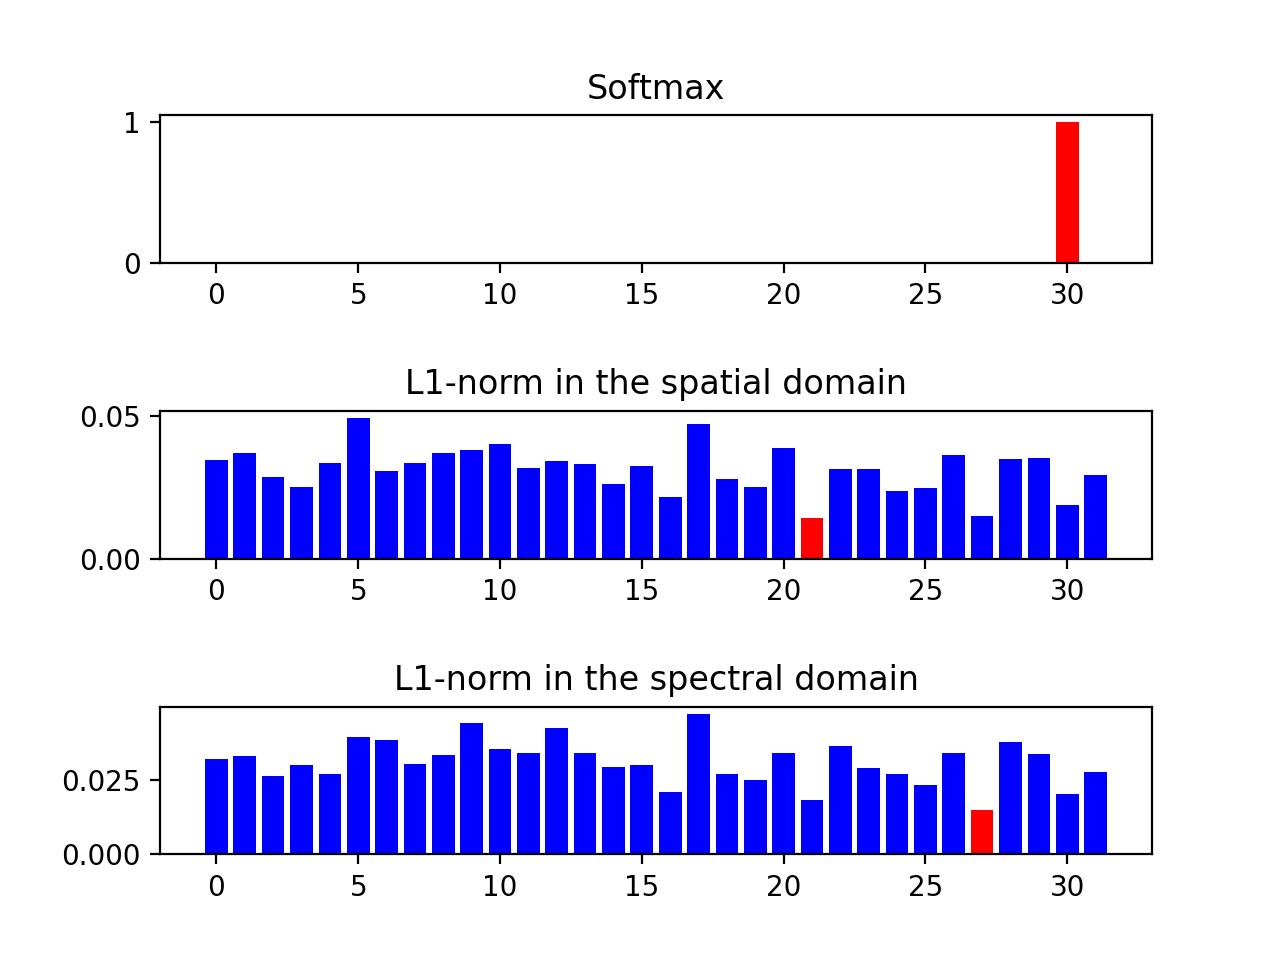}
\caption{Prototype assignments for a fixed vector under different metric.}
\label{fig:soft_l1_10}
\end{figure*}





%%%%%%%%% REFERENCES
{\small
\bibliographystyle{ieee_fullname}
\bibliography{egbib}
}

\end{document}
